# Supplementary material for: SCRREAM : SCan, Register, REnder And Map:A Framework for Annotating Accurate and Dense 3D Indoor Scenes with a Benchmark
Source: arXiv:2410.22715 source file (2025-01-06)
Supplement: Supplementary file 1 [file suppl_1_hardware.tex]

\section{Hardware Setup} \label{sec:suppl_hardware}

We use a specially designed camera rig (Fig.~\ref{fig:hardware}, (a)) to capture the synchronized multi-modal image sequences in a free hand manner. RGB and polarization images are acquired with a Phoenix 5.0 MP Polarization camera (PHX050S1-QC, LUCID Vision Labs, Canada) equipped with a Sony Polarsens sensor (IMX264MYR CMOS, Sony, Japan). For the depth images, we use two depth modality, active stereo depth and indirect time-of-flight depth. Intel RealSense D435 (Intel, USA) is used for the active stereo depth and Lucid Helios (HLS003S-001, LUCID Vision Labs, Canada) is used for indirect time-of-flight depth. For synchronization, a Raspberry Pi generates a trigger signal that is connected to all cameras to trigger the image acquisition. 

Two different types of scanners are used for the scanning. For the small household objects, such as cups or water bottles, we use the table-top scanner (EinScan-SP, SHINING 3D Tech. Co., Ltd., Hangzhou, China, Fig.~\ref{fig:hardware}, (b)) to capture the meshes with fine details. For the larger objects that do not fit to the table-top scanner, such as furniture or medium size objects or room, we use hand held scanner (Artec-Leo, Artec 3D, Luxembourg, Fig.~\ref{fig:hardware}, (c)) that runs SLAM internally for tracking the scanning. To scan large texture-less areas, such as walls or big tables, we use small stripes of masking tape on the surface to provide additional texture (Fig.~\ref{fig:wall_example}, (a)) during the scanning. Later, the textures from the masking tapes are removed via the texture healing function in Artec Studio 17 ((Fig.~\ref{fig:wall_example}, (b)).

\begin{figure*}[!h]
 \centering
    \includegraphics[width=\linewidth]{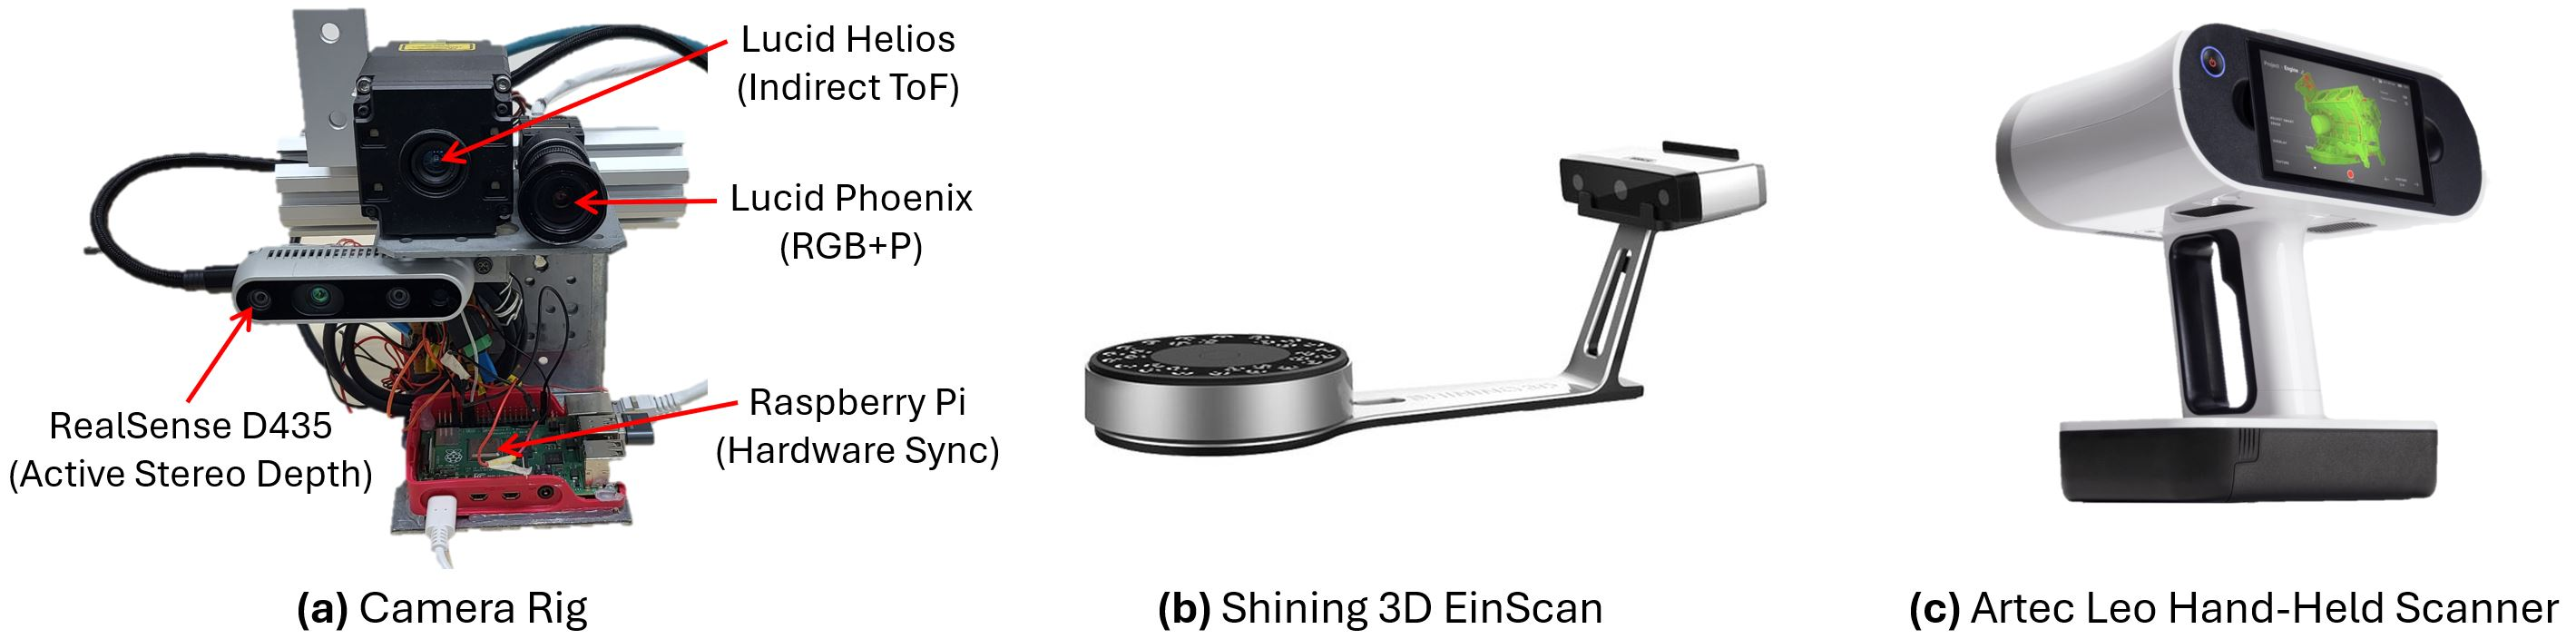}
    \caption{\textbf{Hardware Setup.}}
    \label{fig:hardware}
\end{figure*}

\begin{figure*}[!h]
 \centering
    \includegraphics[width=\linewidth]{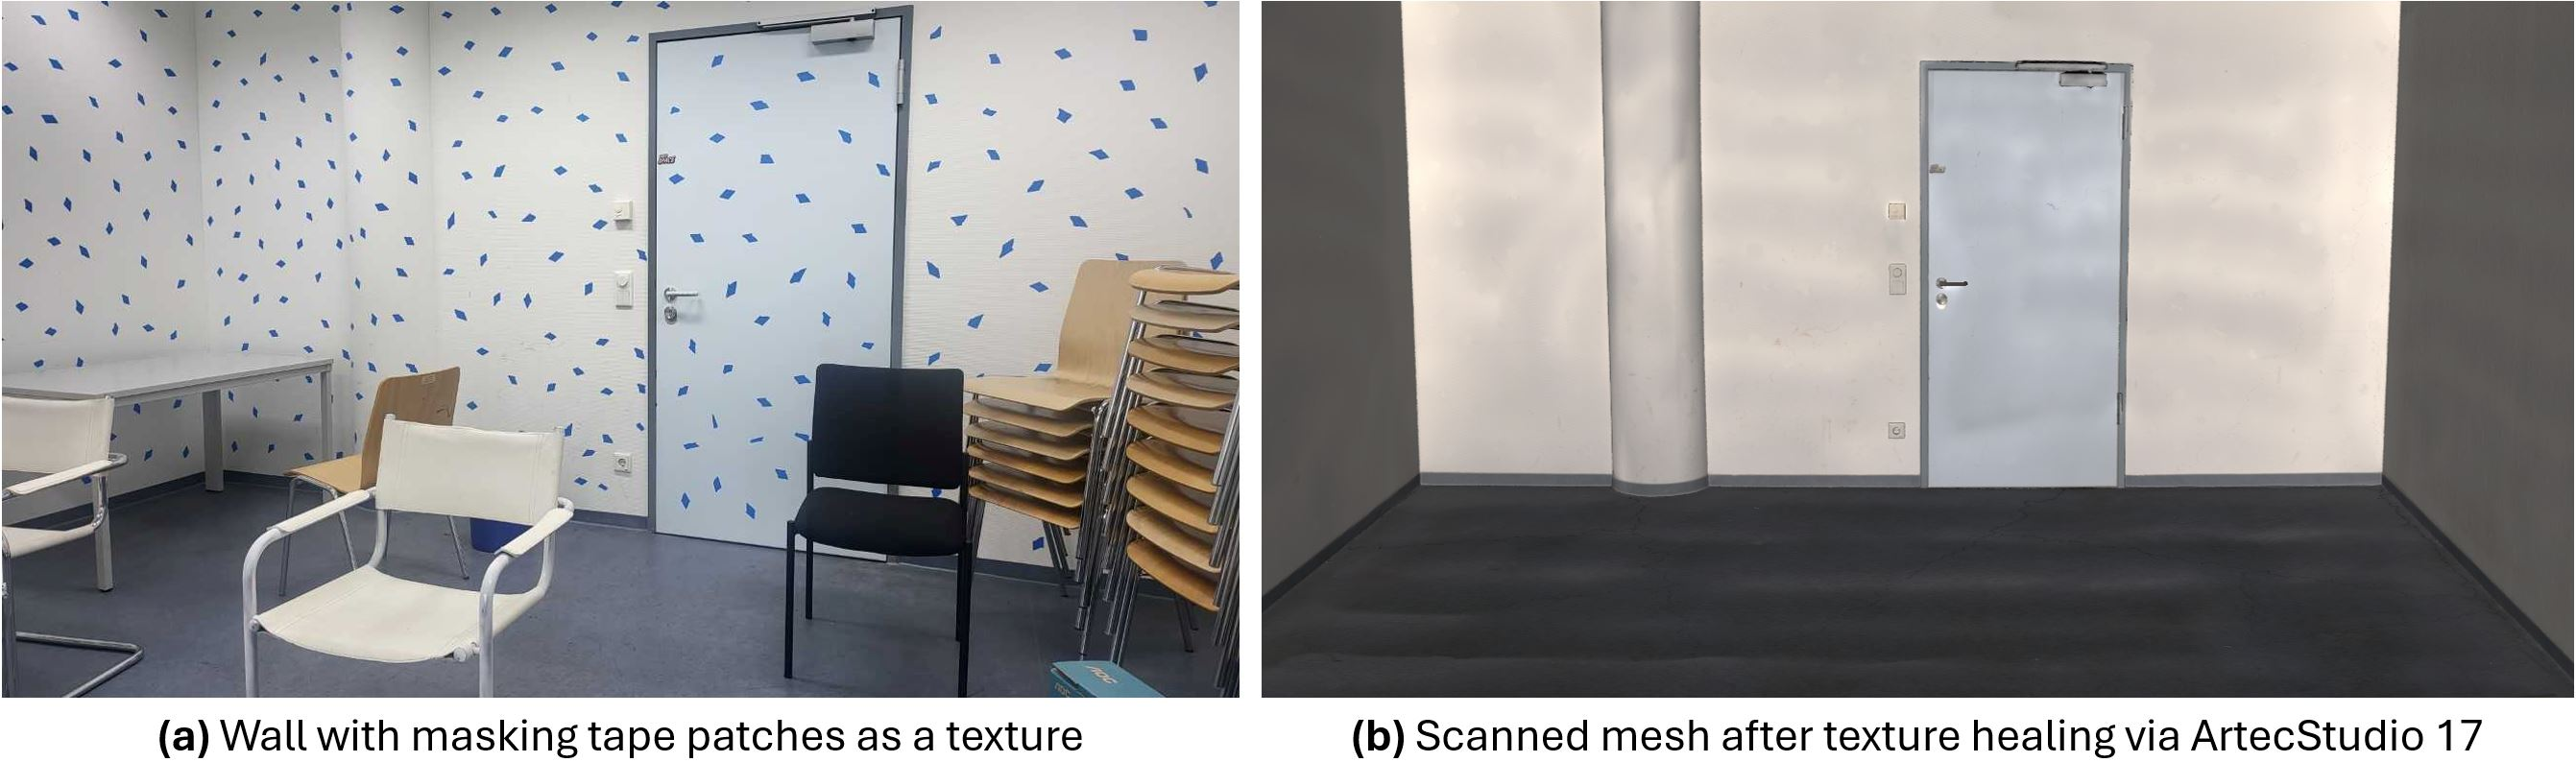}
    \caption{\textbf{Example of Wall Scanning.} To help tracking the hand-held scanner on the plain white wall, we attach patches of masking tape on the wall to provide additional texture (a). Later, the texture of the tape can be removed in a post-processing step (b).}
    \label{fig:wall_example}
\end{figure*}
