# Supplementary material for: SCRREAM : SCan, Register, REnder And Map:A Framework for Annotating Accurate and Dense 3D Indoor Scenes with a Benchmark
Source: arXiv:2410.22715 source file (2025-01-06)
Supplement: Supplementary file 2 [file suppl_2_data_example.tex]

\section{Dataset Examples} \label{sec:suppl_dataset_example}

\textbf{Indoor Reconstruction and SLAM Dataset.} We provide 11 scenes that comprise 7114 frames, 94 object \& furniture meshes and 7 indoor room meshes for the indoor reconstruction and SLAM dataset. Note that all furniture and objects in the scenes are scanned prior to ensure the meshes are high resolution and water-tight, in order to serve as digital twin assets so that the rendered depth does not miss any parts of the scene. The visualization of each scene mesh is shown in Fig.~\ref{fig:indoor_example}.

\textbf{Object Removal \& Scene Editing Dataset.} We capture multiple additional video sequences for each of the 8 selected scenes from the indoor reconstruction and SLAM dataset each with a reduced number of objects or furniture to obtain multiple examples for object removal and scene editing tasks. This set is comprised of additional 9323 frames. A visualization of each reduced scene is shown in Fig.~\ref{fig:removal_example_s1}-~\ref{fig:removal_example_s9}. Note that for each reduced scene, we capture the real image sequence with the camera rig.

\textbf{Human Reconstruction Dataset.} For the semi-dynamic human sequences with the mannequin, we do scanning, registration, rendering and mapping for all individual frames. We showcase 2 scenes captured with this setup. We show the scene with a single human mesh from the first frame (Fig~\ref{fig:human_scenes}, left) to show the scene setup as well as all human meshes from the entire video sequence (Fig~\ref{fig:human_scenes}, right) to show the motion range of the mannequin. Note that around 4 real images are captured per time frame for the mapping step.

\textbf{6D Pose Estimation Dataset.} We showcase two pose dataset scenes in Fig~\ref{fig:pose_scenes}. By nature of our dataset annotation pipeline, we can obtain object poses w.r.t. the world coordinate system \(T_{obj->world}\) and camera poses w.r.t. the world coordinate system \(T_{cam->world}\). By concatenating both pose in the right order (e.g. \(T_{obj->world}^{-1}\cdot T_{obj->world}\)), the object pose w.r.t. the camera center \(T_{obj->cam}\), the so called 6D object pose, can be obtained. Having registered the object poses using our framework, the free-hand camera rig can be used to quickly and easily capture a pose dataset with extensive camera coverage.

\begin{figure*}[!t]
 \centering
    \includegraphics[width=\linewidth]{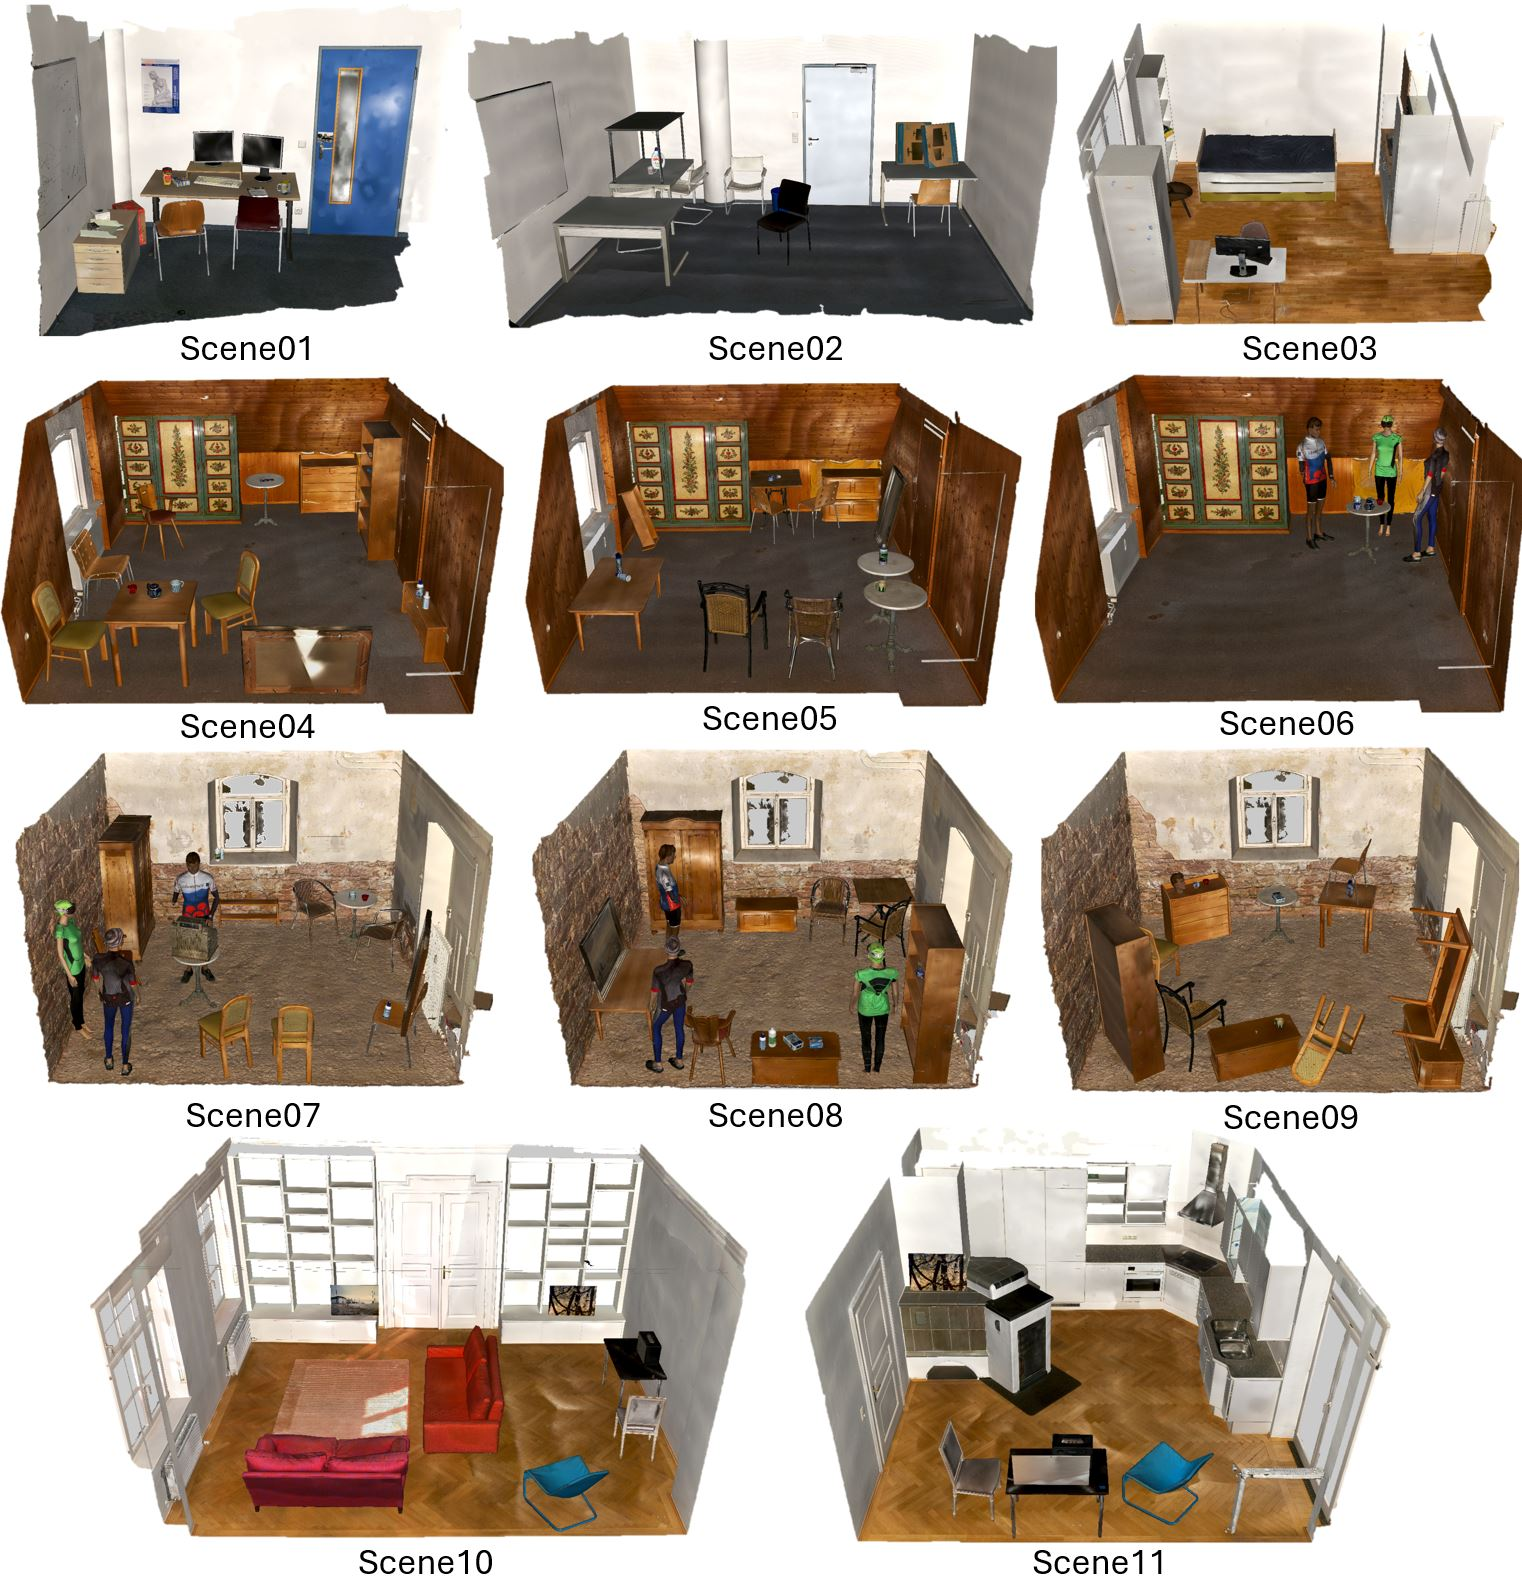}
    \caption{\textbf{Example of Indoor Reconstruction and SLAM Scenes.}}
    \label{fig:indoor_example}
\end{figure*}

\begin{figure*}[!t]
 \centering
    \includegraphics[width=\linewidth]{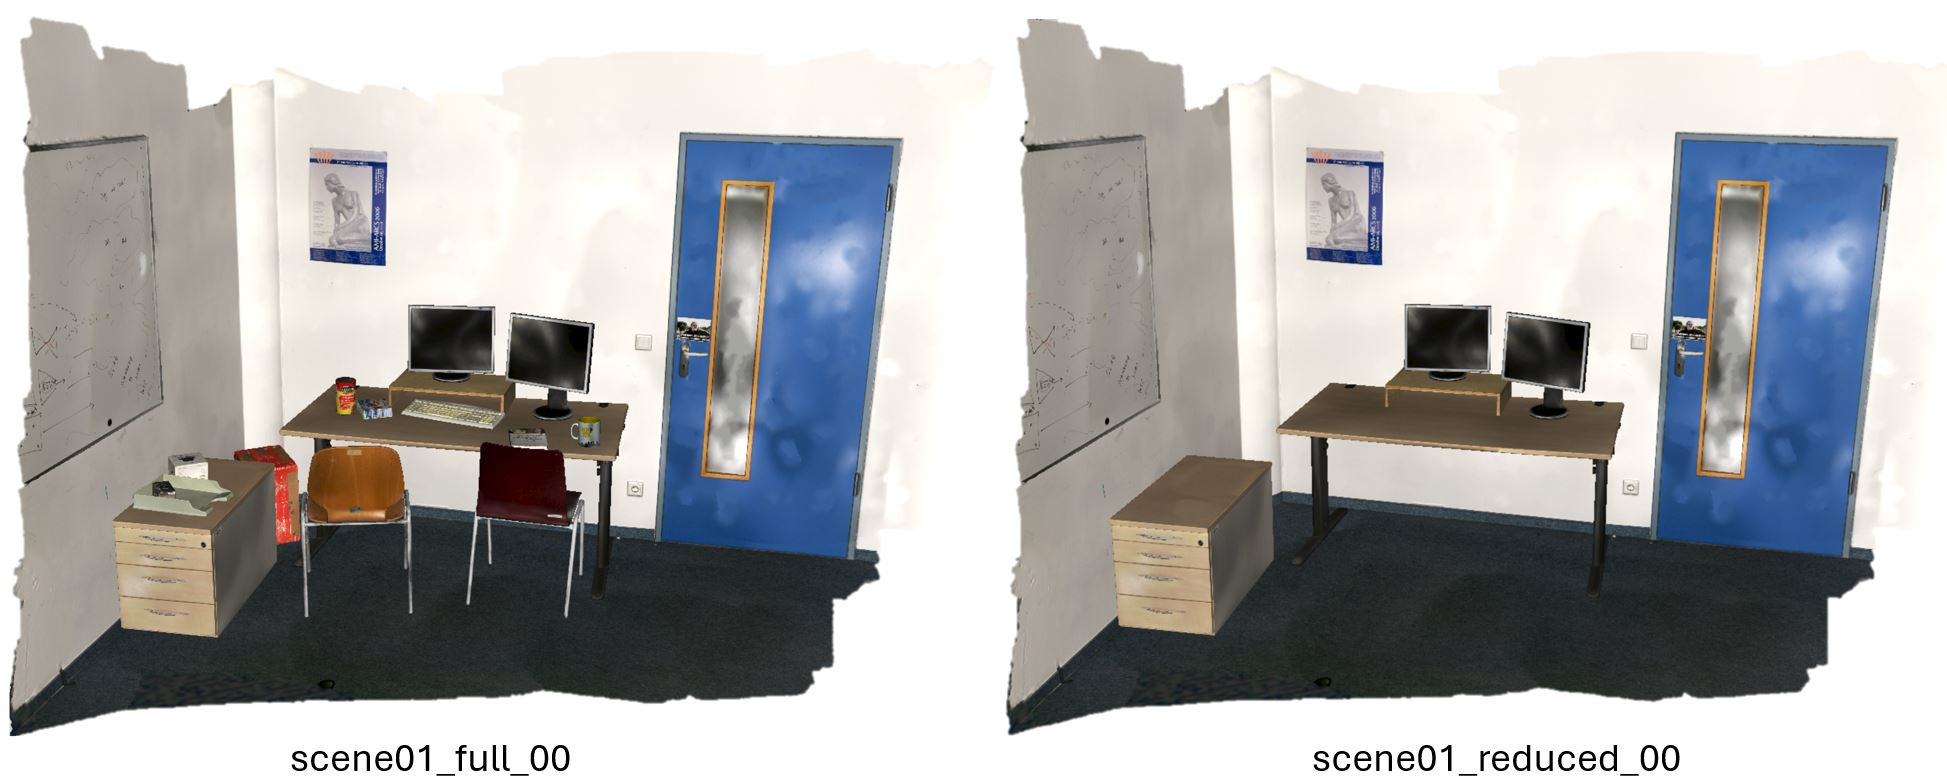}
    \caption{\textbf{Example of Reduced Scenes For Scene01.}}
    \label{fig:removal_example_s1}
\end{figure*}

\begin{figure*}[!t]
 \centering
    \includegraphics[width=\linewidth]{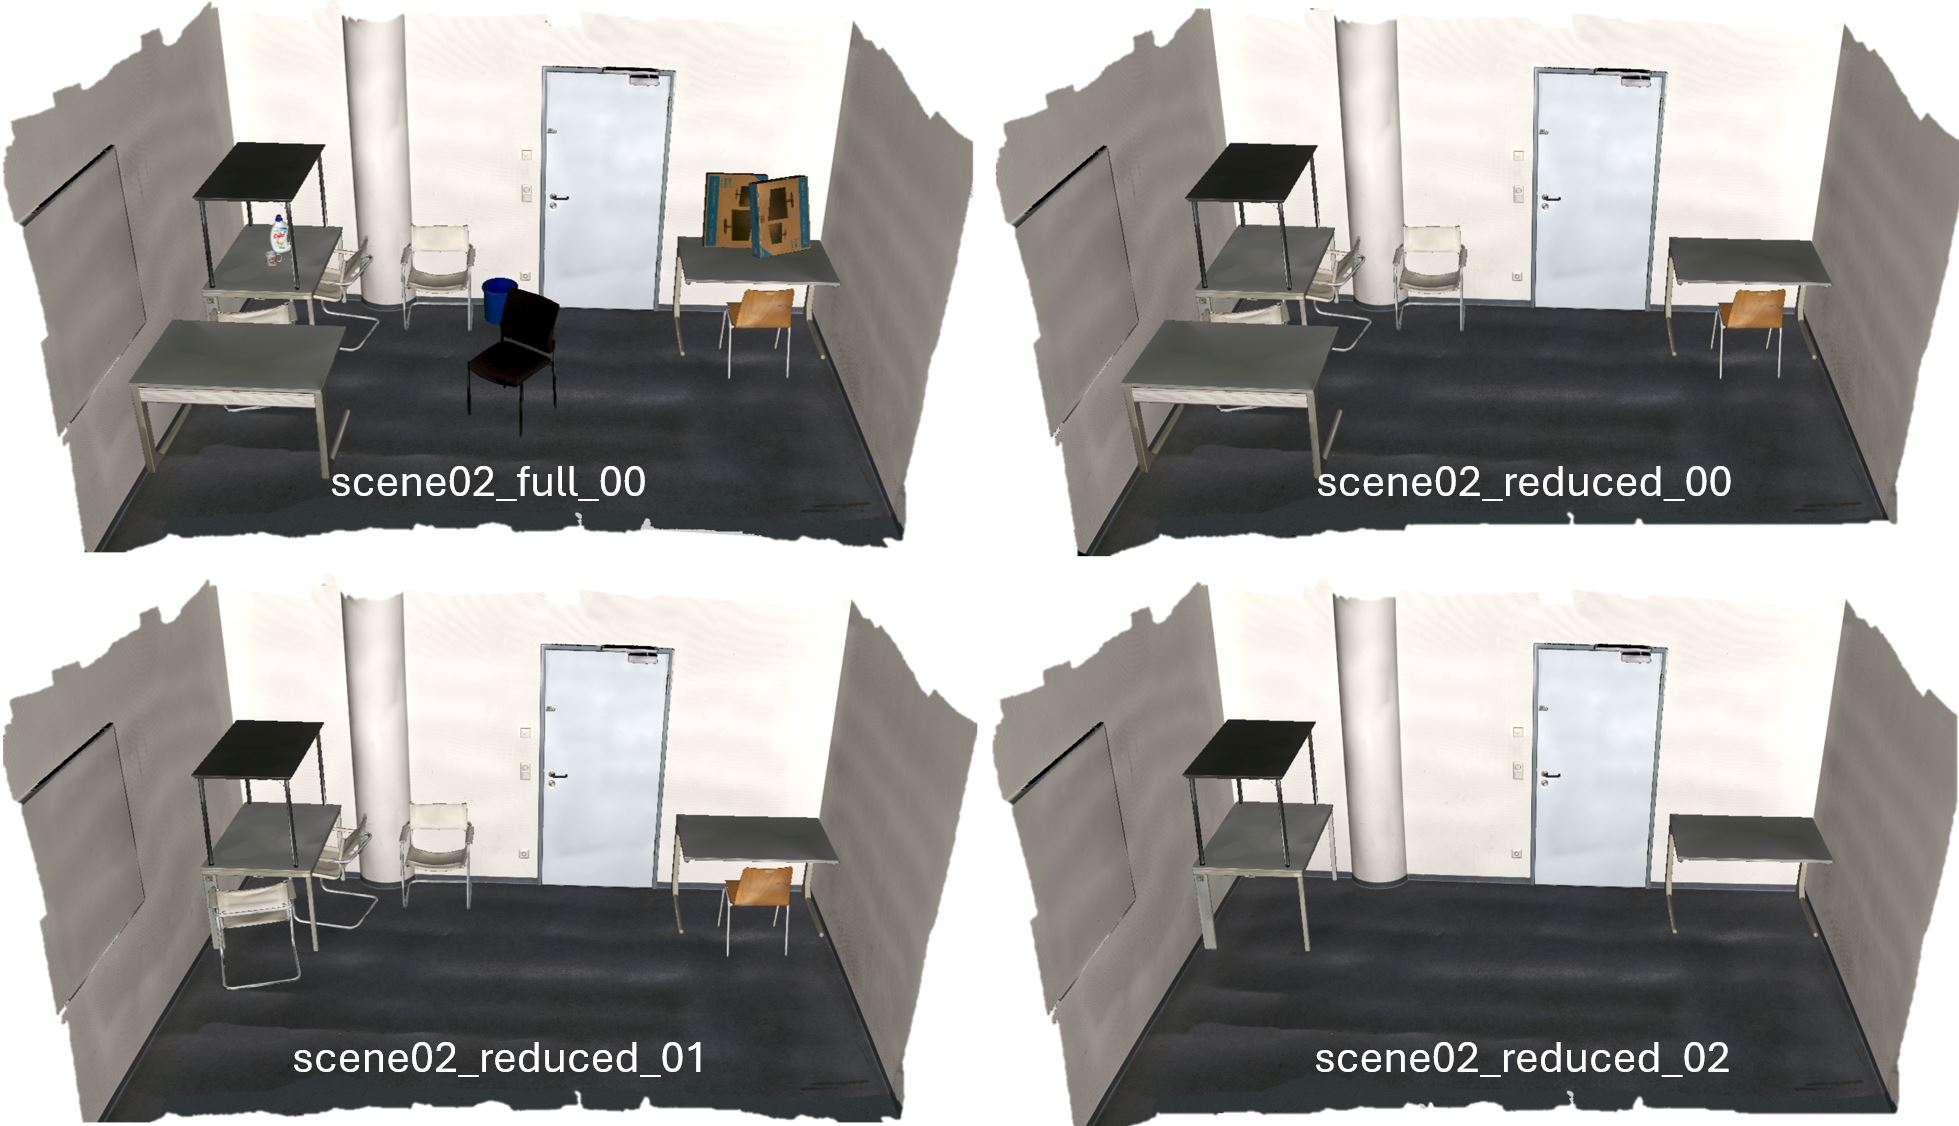}
    \caption{\textbf{Example of Reduced Scenes For Scene02.}}
    \label{fig:removal_example_s2}
\end{figure*}

\begin{figure*}[!t]
 \centering
    \includegraphics[width=\linewidth]{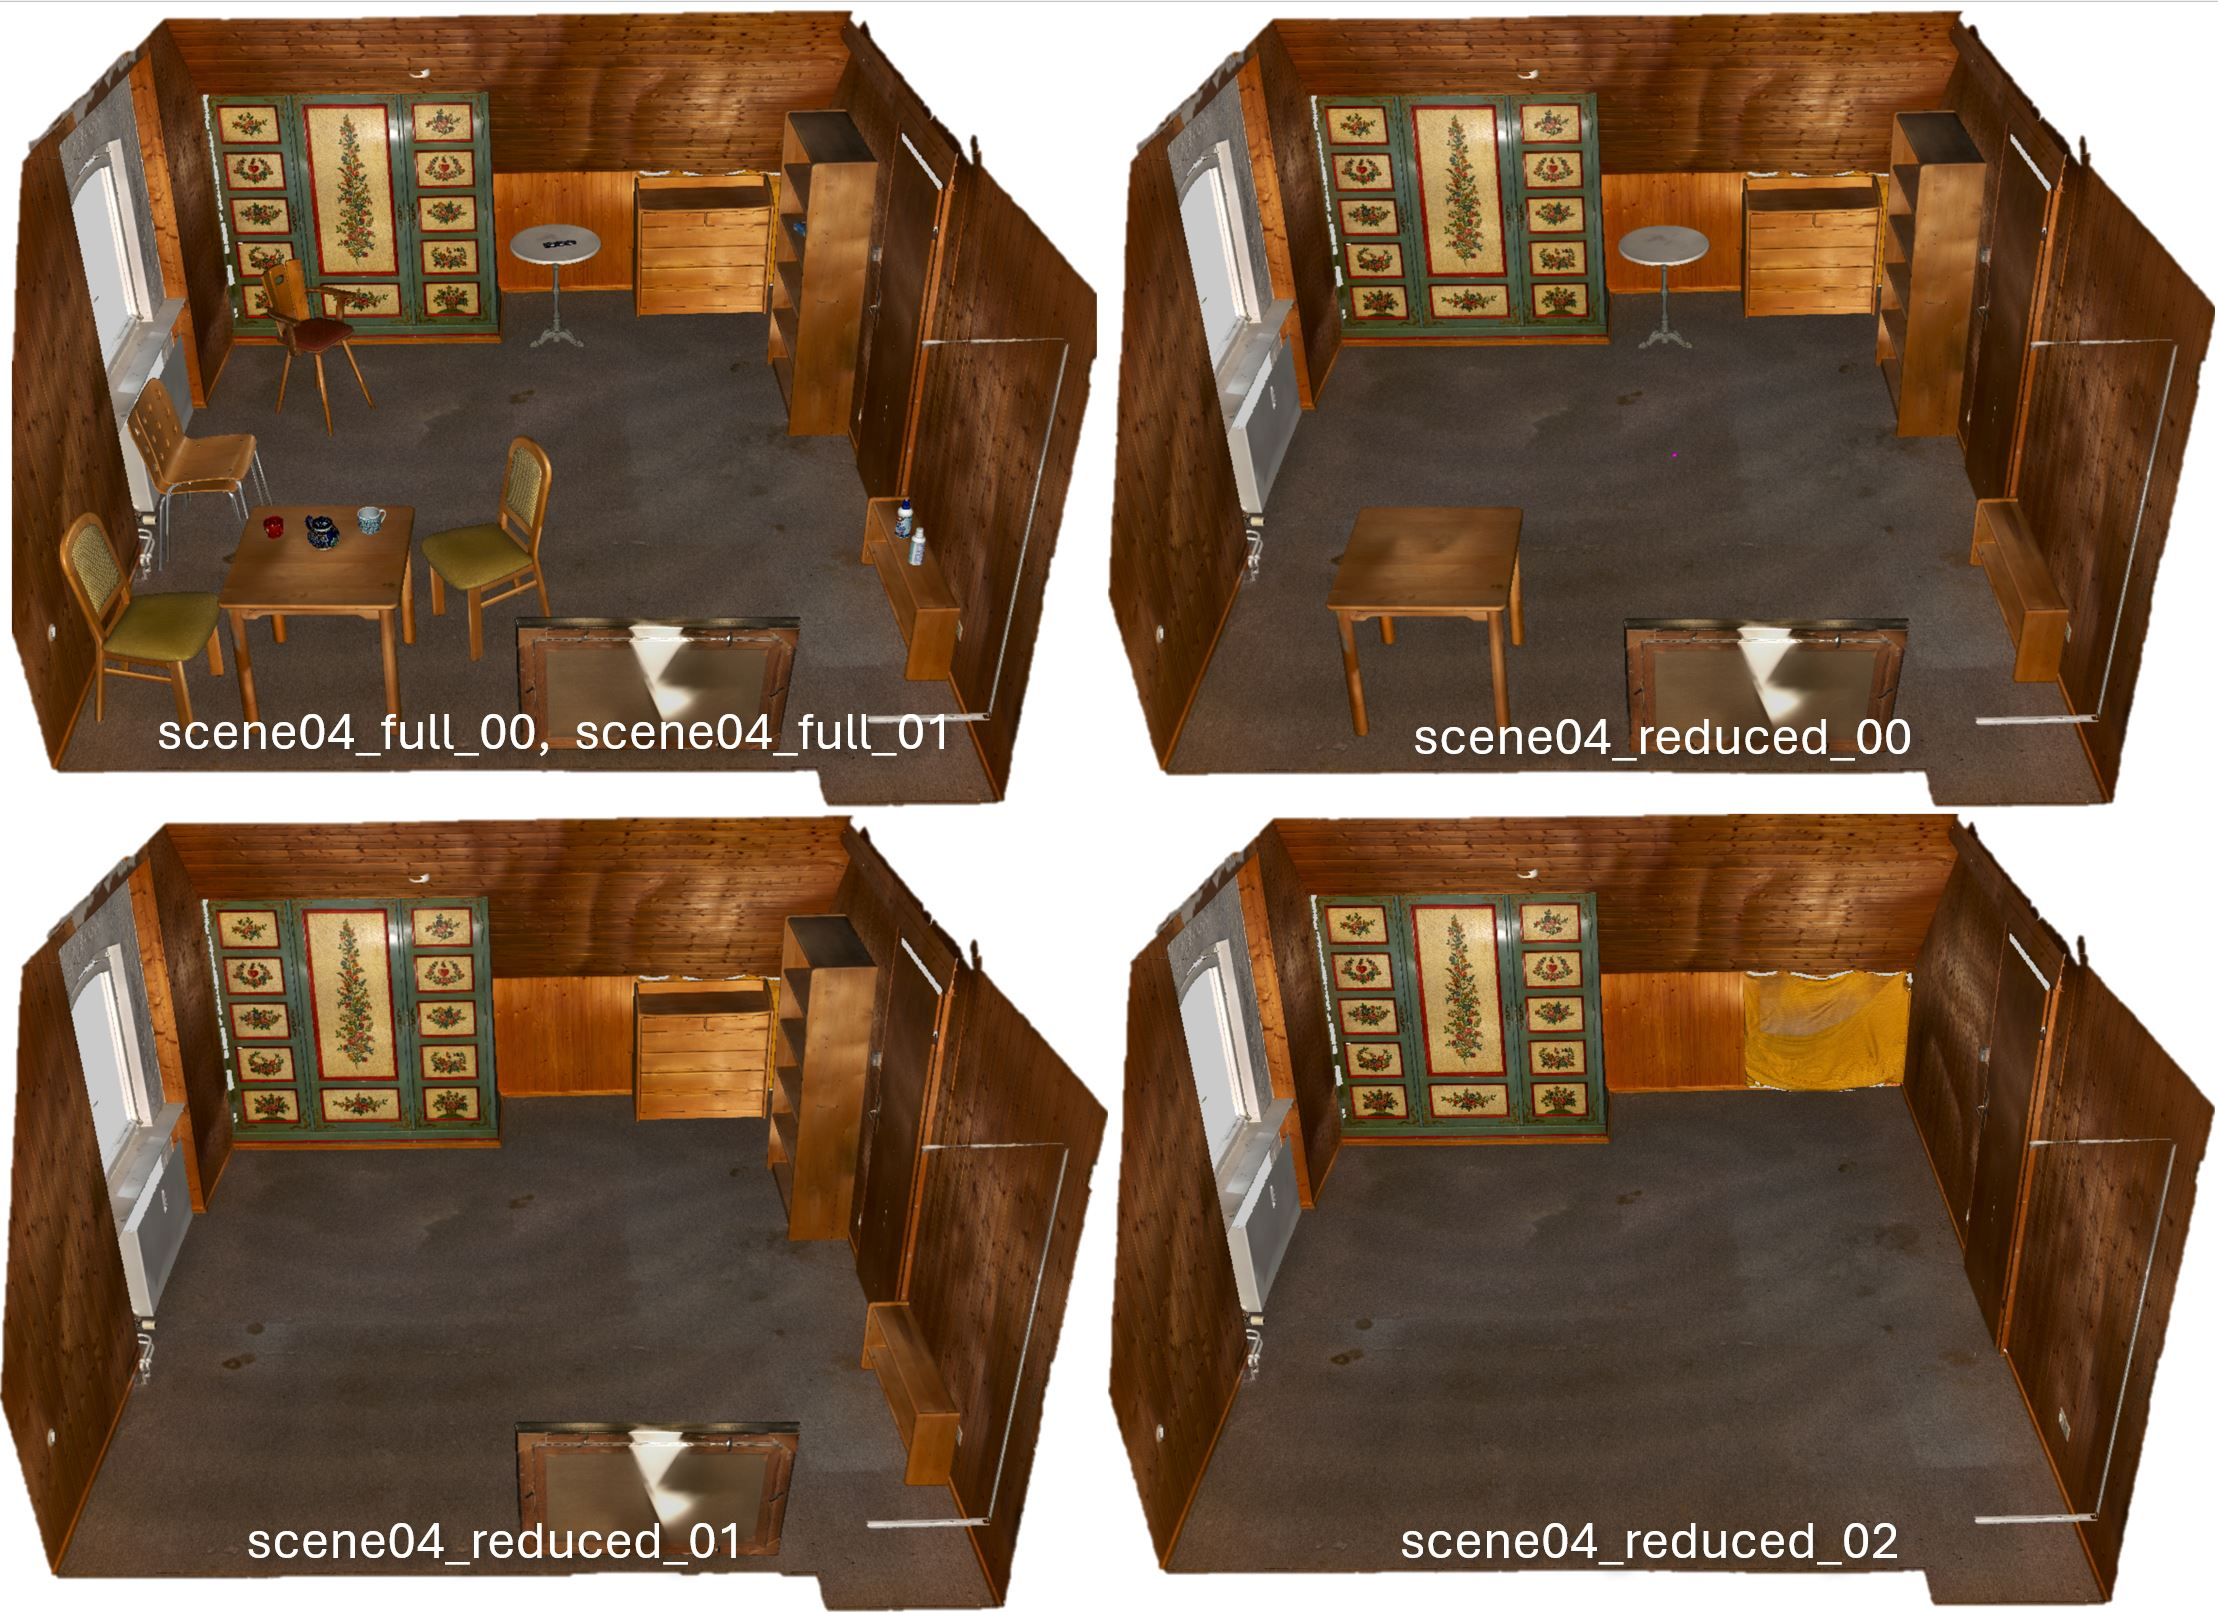}
    \caption{\textbf{Example of Reduced Scenes For Scene04.}}
    \label{fig:removal_example_s3}
\end{figure*}

\begin{figure*}[!t]
 \centering
    \includegraphics[width=\linewidth]{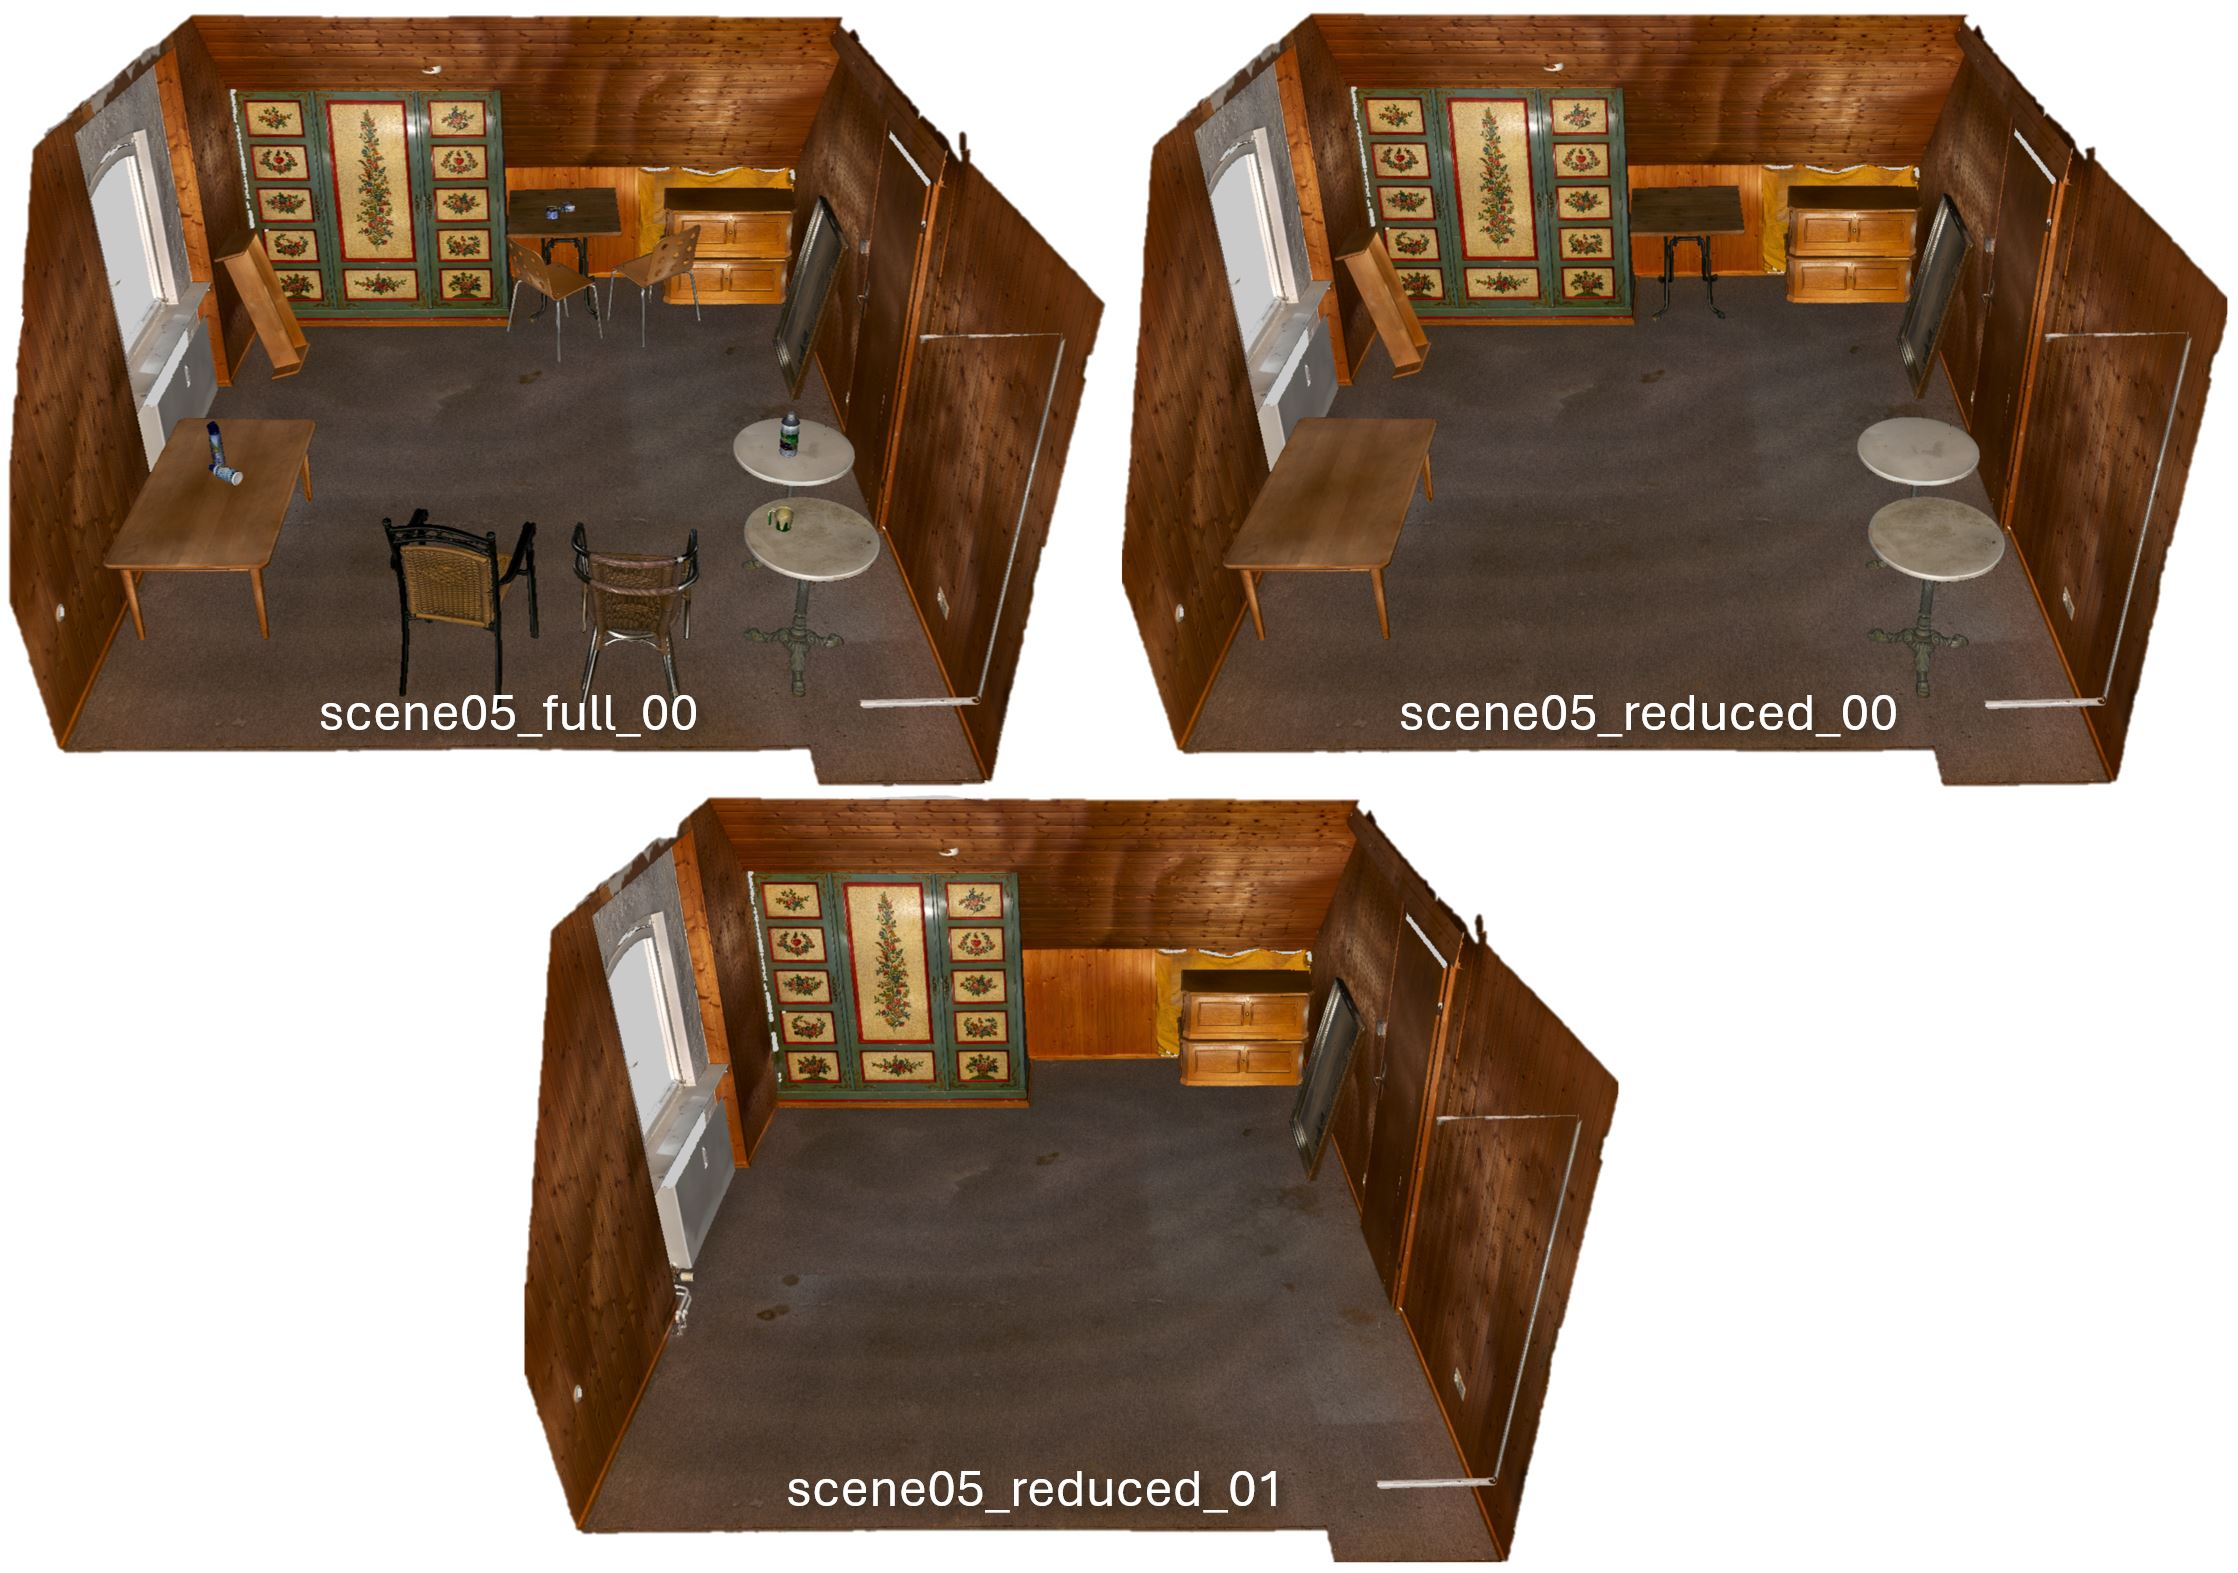}
    \caption{\textbf{Example of Reduced Scenes For Scene05.}}
    \label{fig:removal_example_s4}
\end{figure*}

\begin{figure*}[!t]
 \centering
    \includegraphics[width=\linewidth]{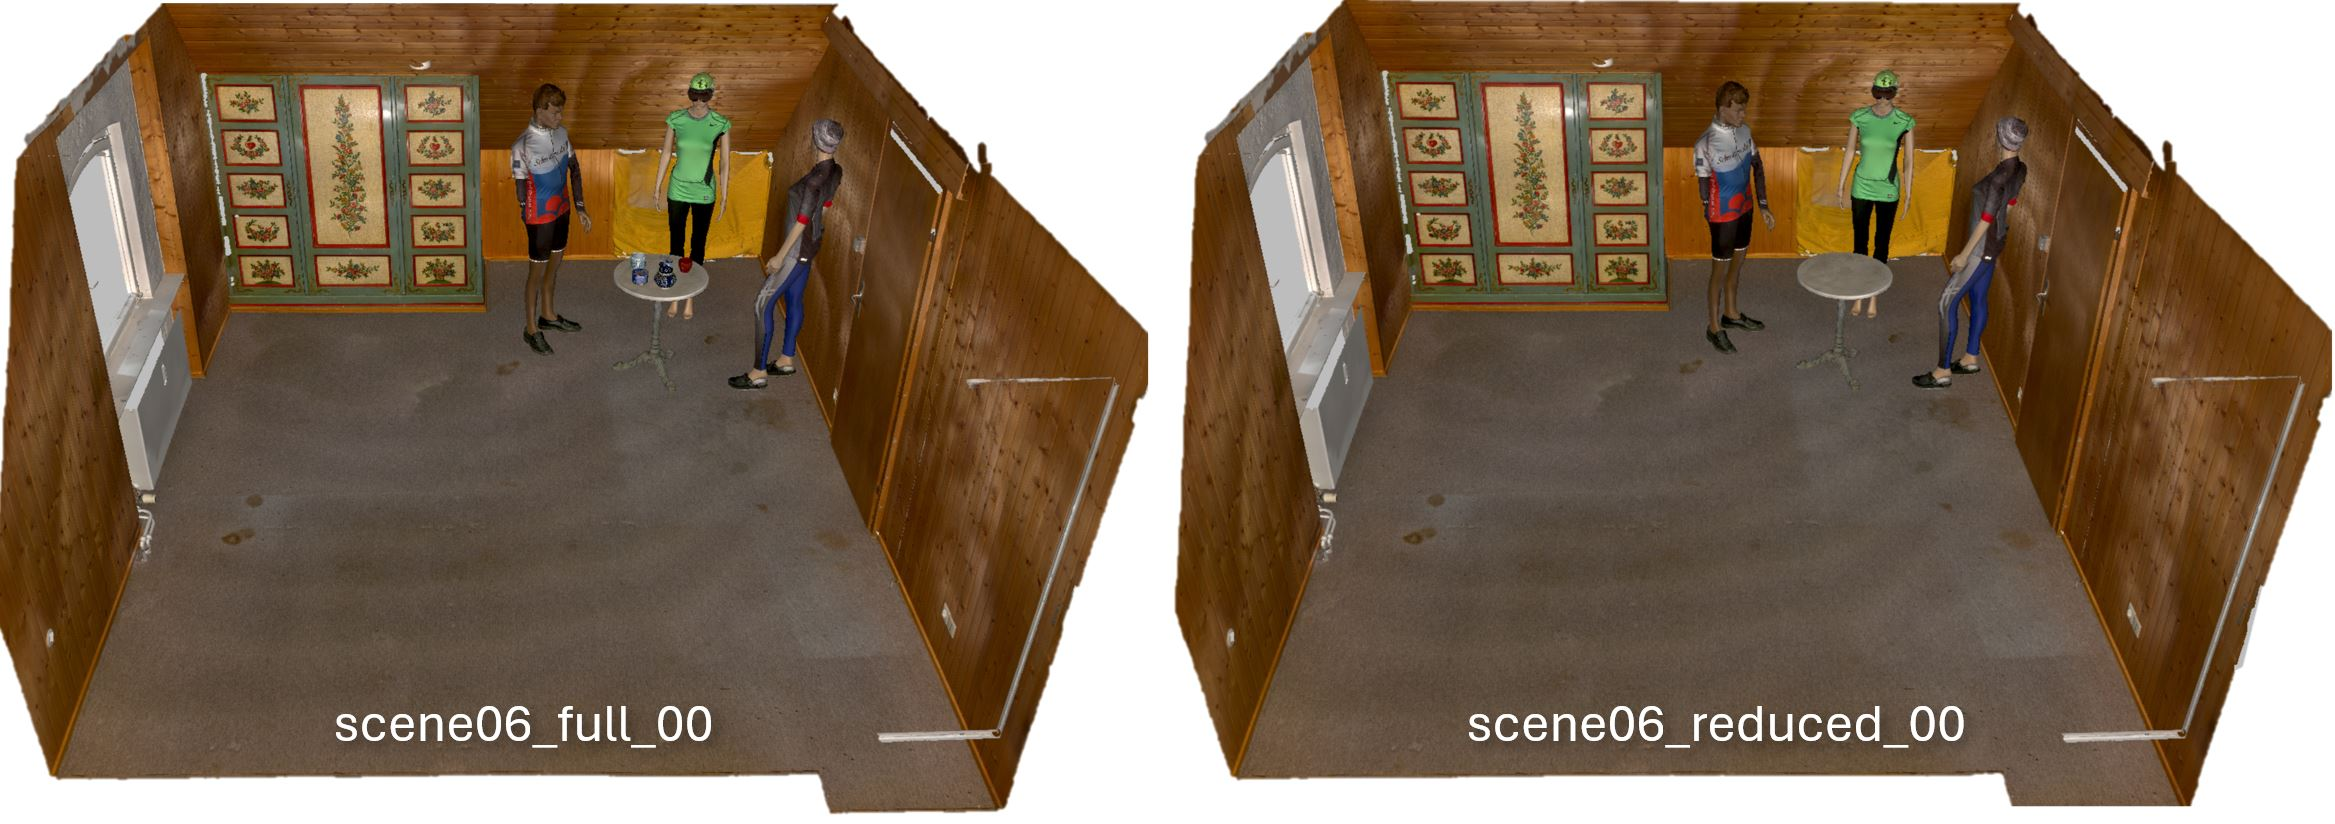}
    \caption{\textbf{Example of Reduced Scenes For Scene06.}}
    \label{fig:removal_example_s5}
\end{figure*}
\clearpage

\begin{figure*}[!t]
 \centering
    \includegraphics[width=\linewidth]{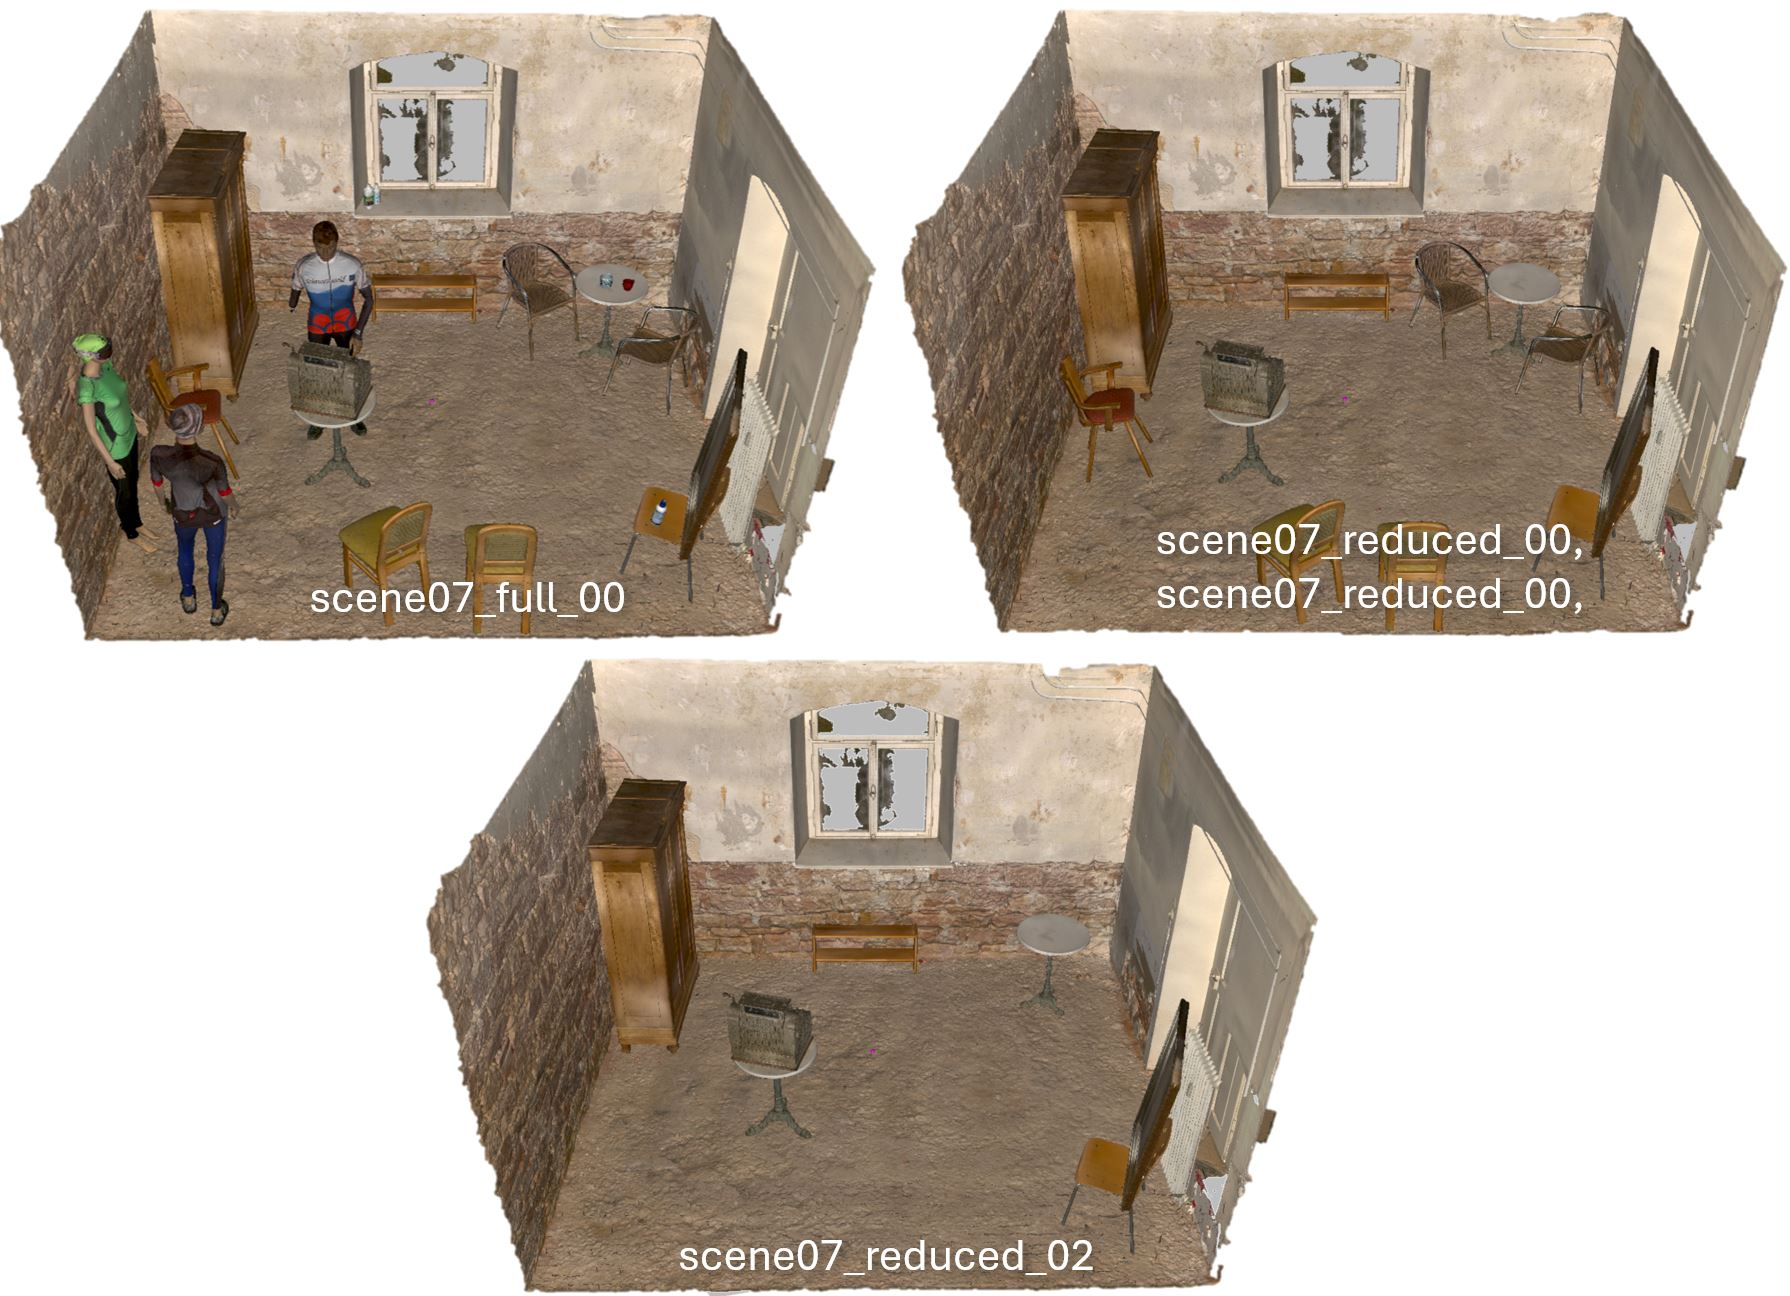}
    \caption{\textbf{Example of Reduced Scenes For Scene07.}}
    \label{fig:removal_example_s7}
\end{figure*}

\begin{figure*}[!t]
 \centering
    \includegraphics[width=\linewidth]{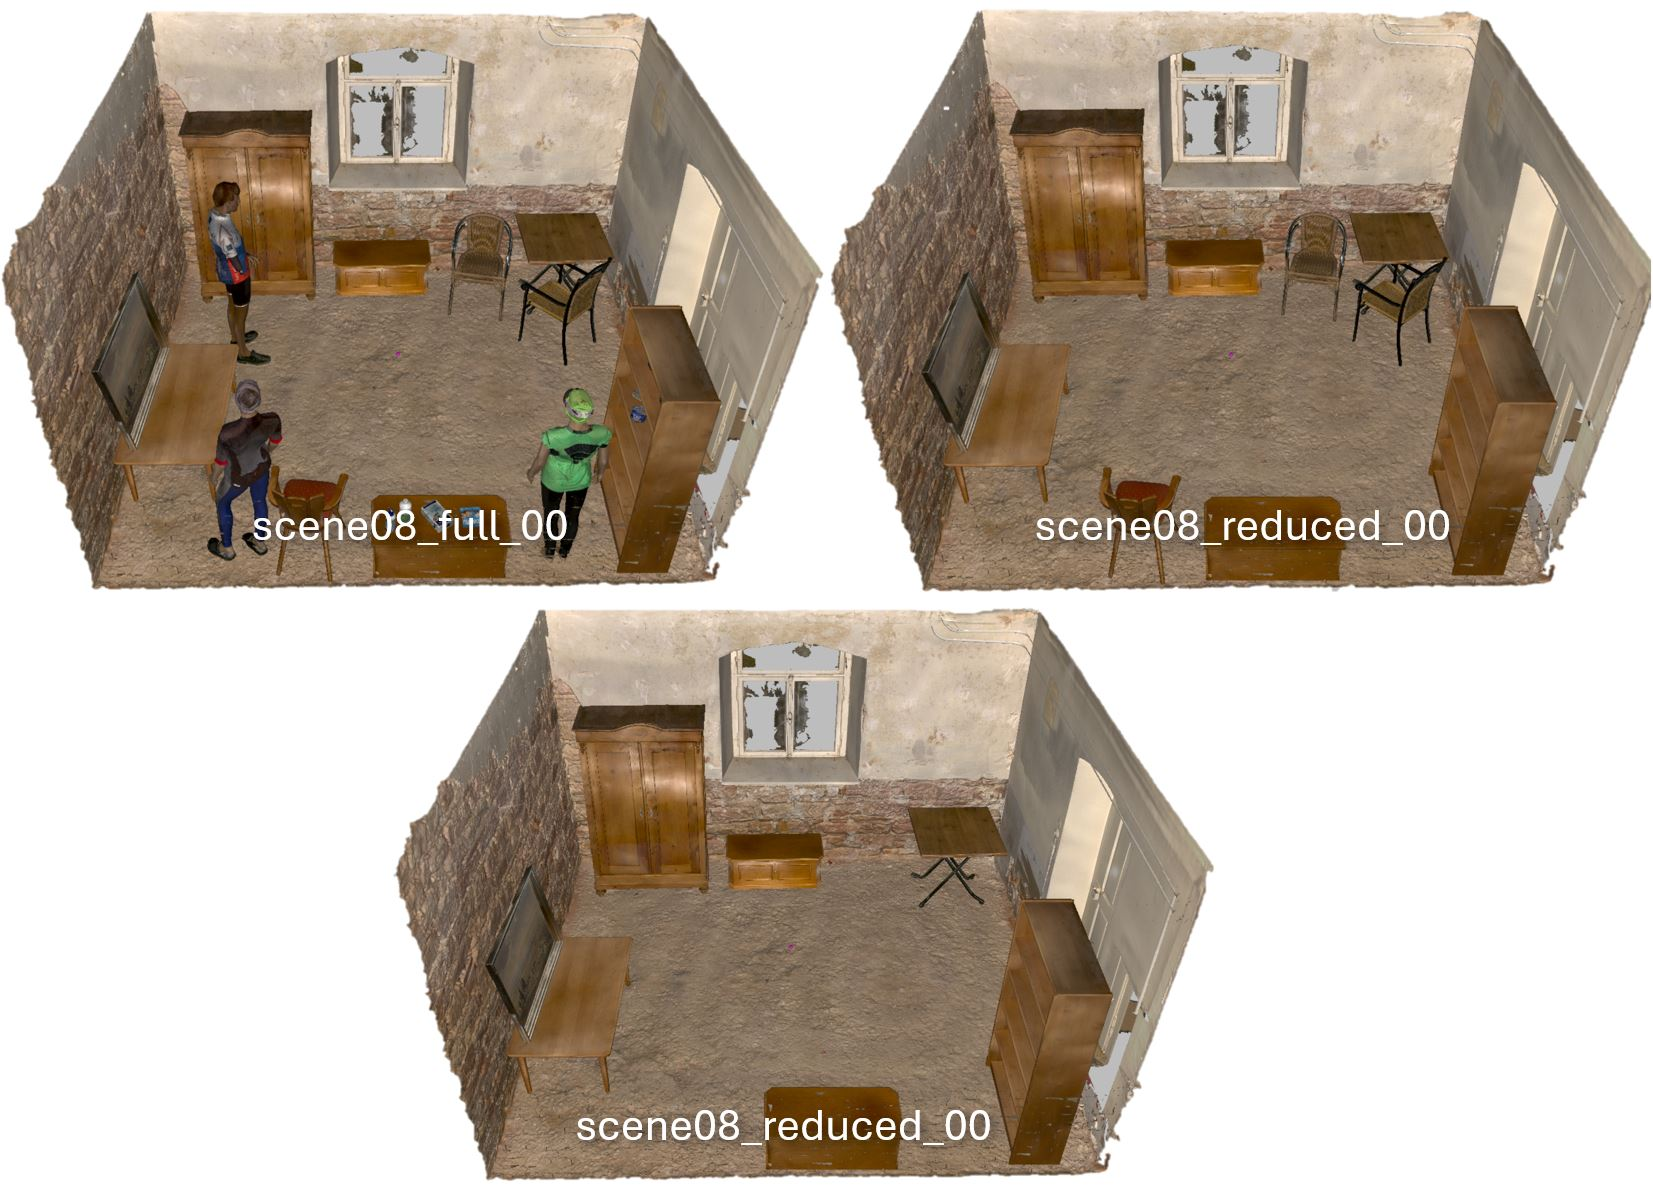}
    \caption{\textbf{Example of Reduced Scenes For Scene08.}}
    \label{fig:removal_example_s8}
\end{figure*}

\begin{figure*}[!t]
 \centering
    \includegraphics[width=\linewidth]{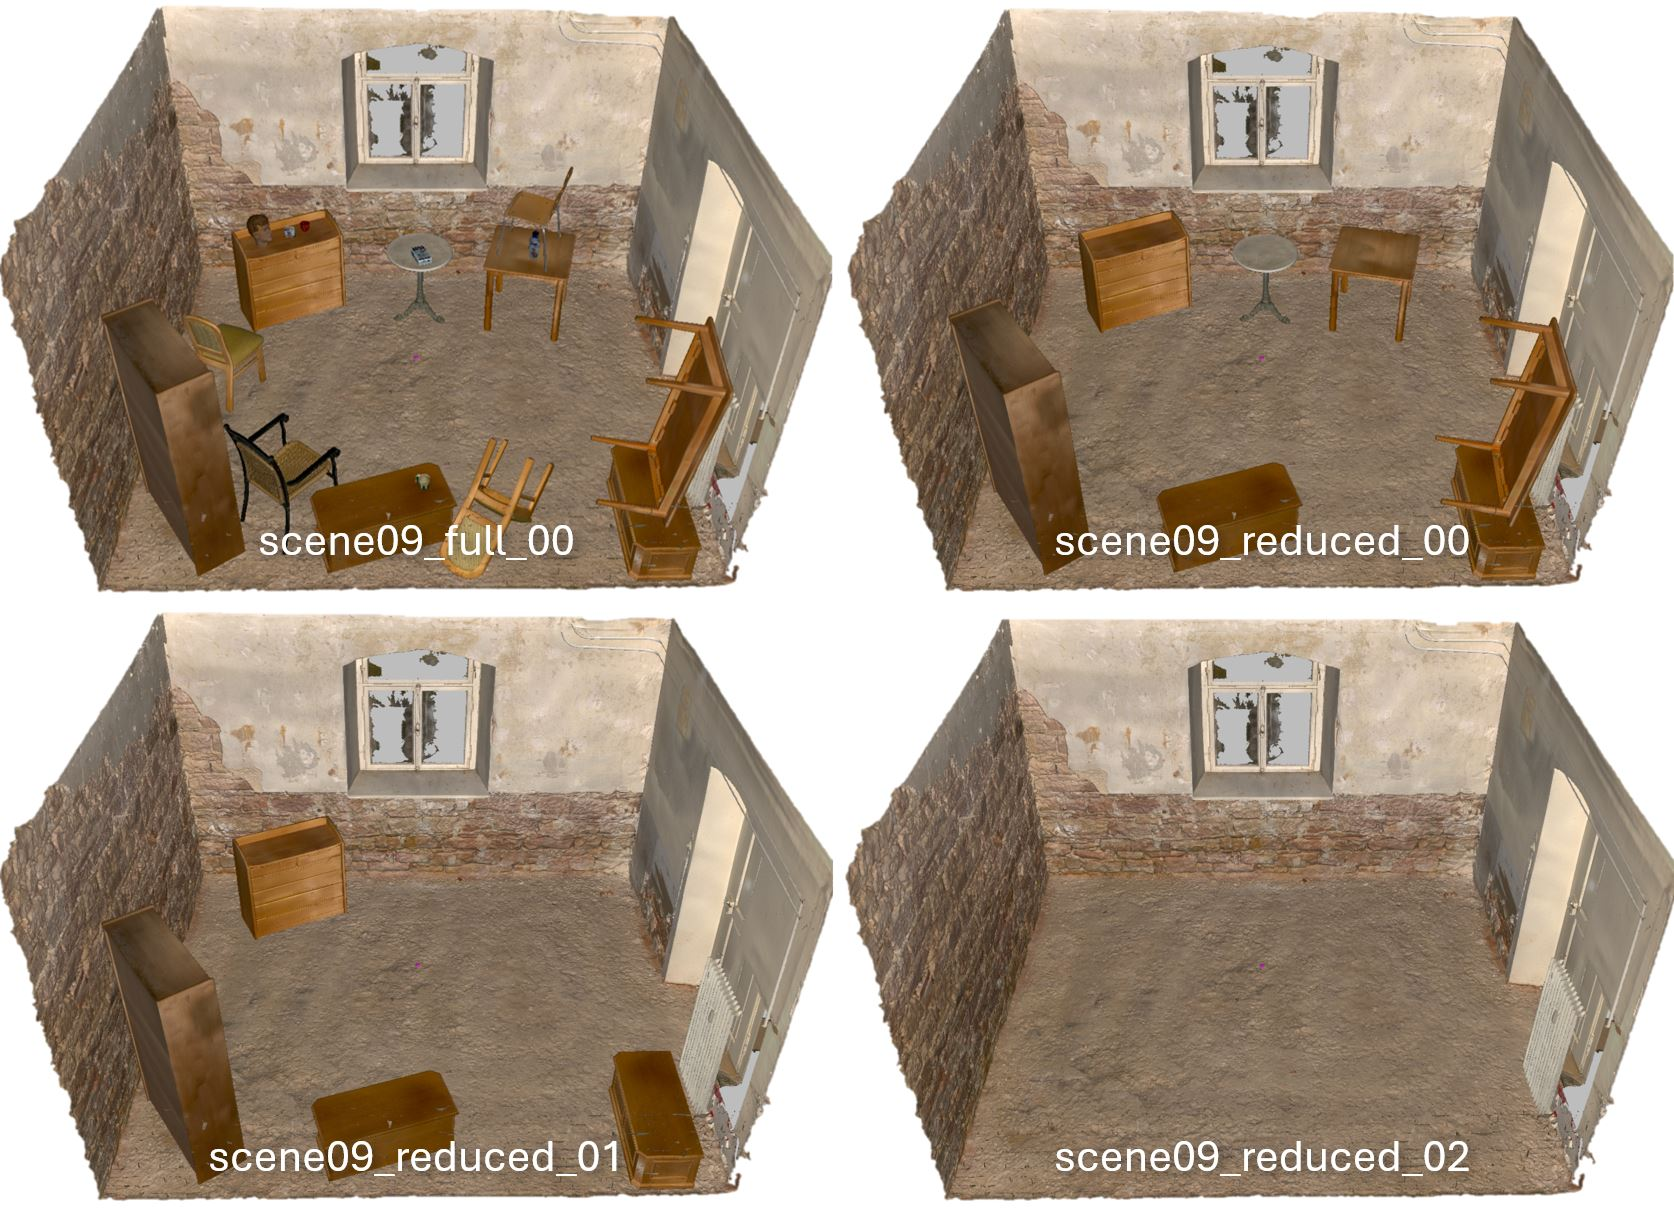}
    \caption{\textbf{Example of Reduced Scenes For Scene09.}}
    \label{fig:removal_example_s9}
\end{figure*}
\clearpage

\begin{figure*}[!t]
 \centering
    \includegraphics[width=\linewidth]{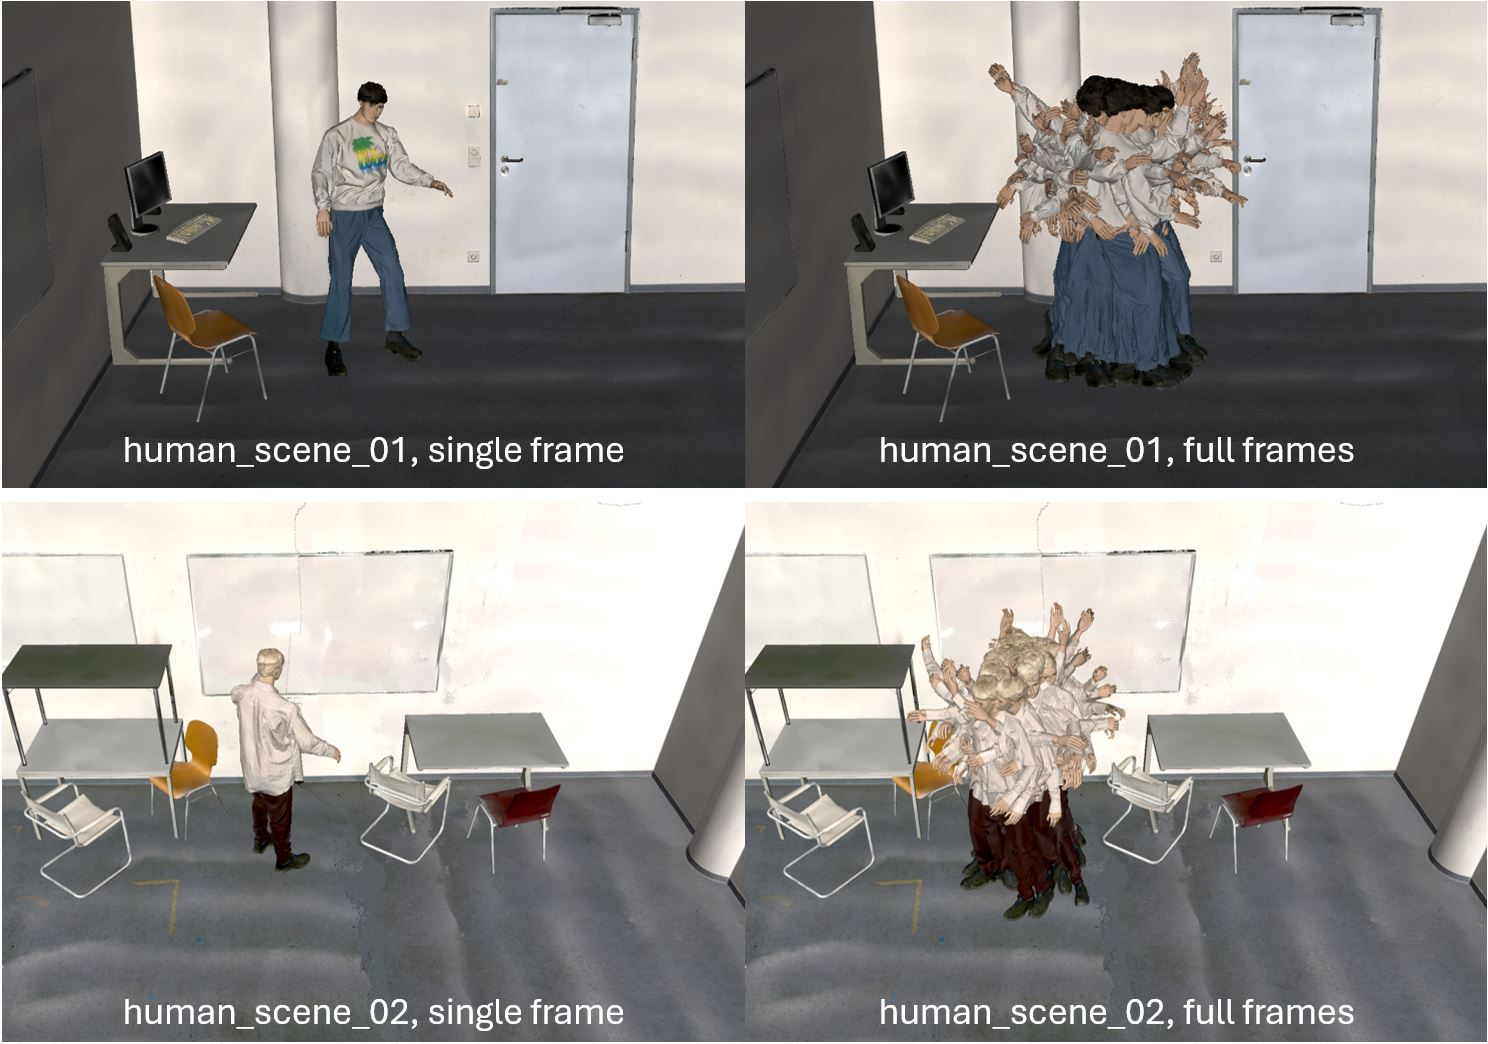}
    \caption{\textbf{Example of Human Dataset Scenes.}}
    \label{fig:human_scenes}
\end{figure*}

\begin{figure*}[!t]
 \centering
    \includegraphics[width=\linewidth]{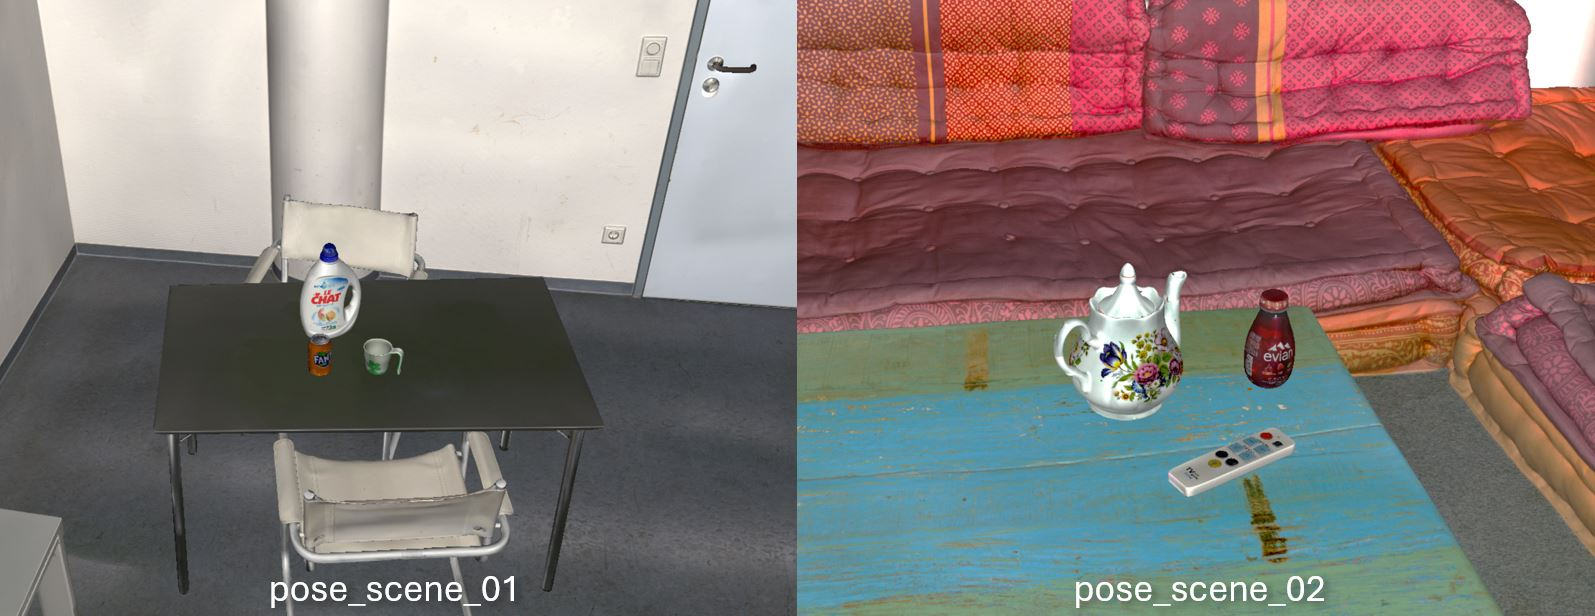}
    \caption{\textbf{Example of Pose Dataset Scenes.}}
    \label{fig:pose_scenes}
\end{figure*}
\clearpage
