# Supplementary material for: SCRREAM : SCan, Register, REnder And Map:A Framework for Annotating Accurate and Dense 3D Indoor Scenes with a Benchmark
Source: arXiv:2410.22715 source file (2025-01-06)
Supplement: Supplementary file 3 [file suppl_3_data_evaluation.tex]

\section{Dataset Comparison} \label{sec:suppl_data_evaluation}

In this section, we show more in-depth comparisons between the existing indoor datasets and our dataset using meshes of the scanned scenes. We choose the ScanNet++~\cite{yeshwanth2023scannet++} and Replica dataset~\cite{replica19arxiv} for comparison.

The ScanNet++ dataset is an improved version of ScanNet~\cite{dai2017scannet}. Instead of using a commercial depth sensor like its predecessor, ScanNet++ uses a LiDAR sensor that rotates and captures a more accurate 360° pointcloud of the scene. To be less dependent on the sensor's line-of-sight ScanNet++ captures the scene from multiple locations in the scene in order to improve the quality and completeness of the mesh. However, no post-processing is applied, such as hole filling, so that the final mesh still has many missing parts, limiting the use of the scene meshes as ground truth for rendering complete views. This is because for the areas with missing geometry the background is visible in the rendering instead of the foreground such that a metric using the incomplete mesh as ground truth will penalize a method that models the foreground object correctly. We show in Fig.~\ref{fig:scannet_vs_ours} that our dataset provides the full details on the office furniture such as the chairs, the trash bin, the monitor etc while ScanNet++ suffers from incomplete and missing parts in the mesh.

\begin{figure*}[!h]
 \centering
    \includegraphics[width=\linewidth]{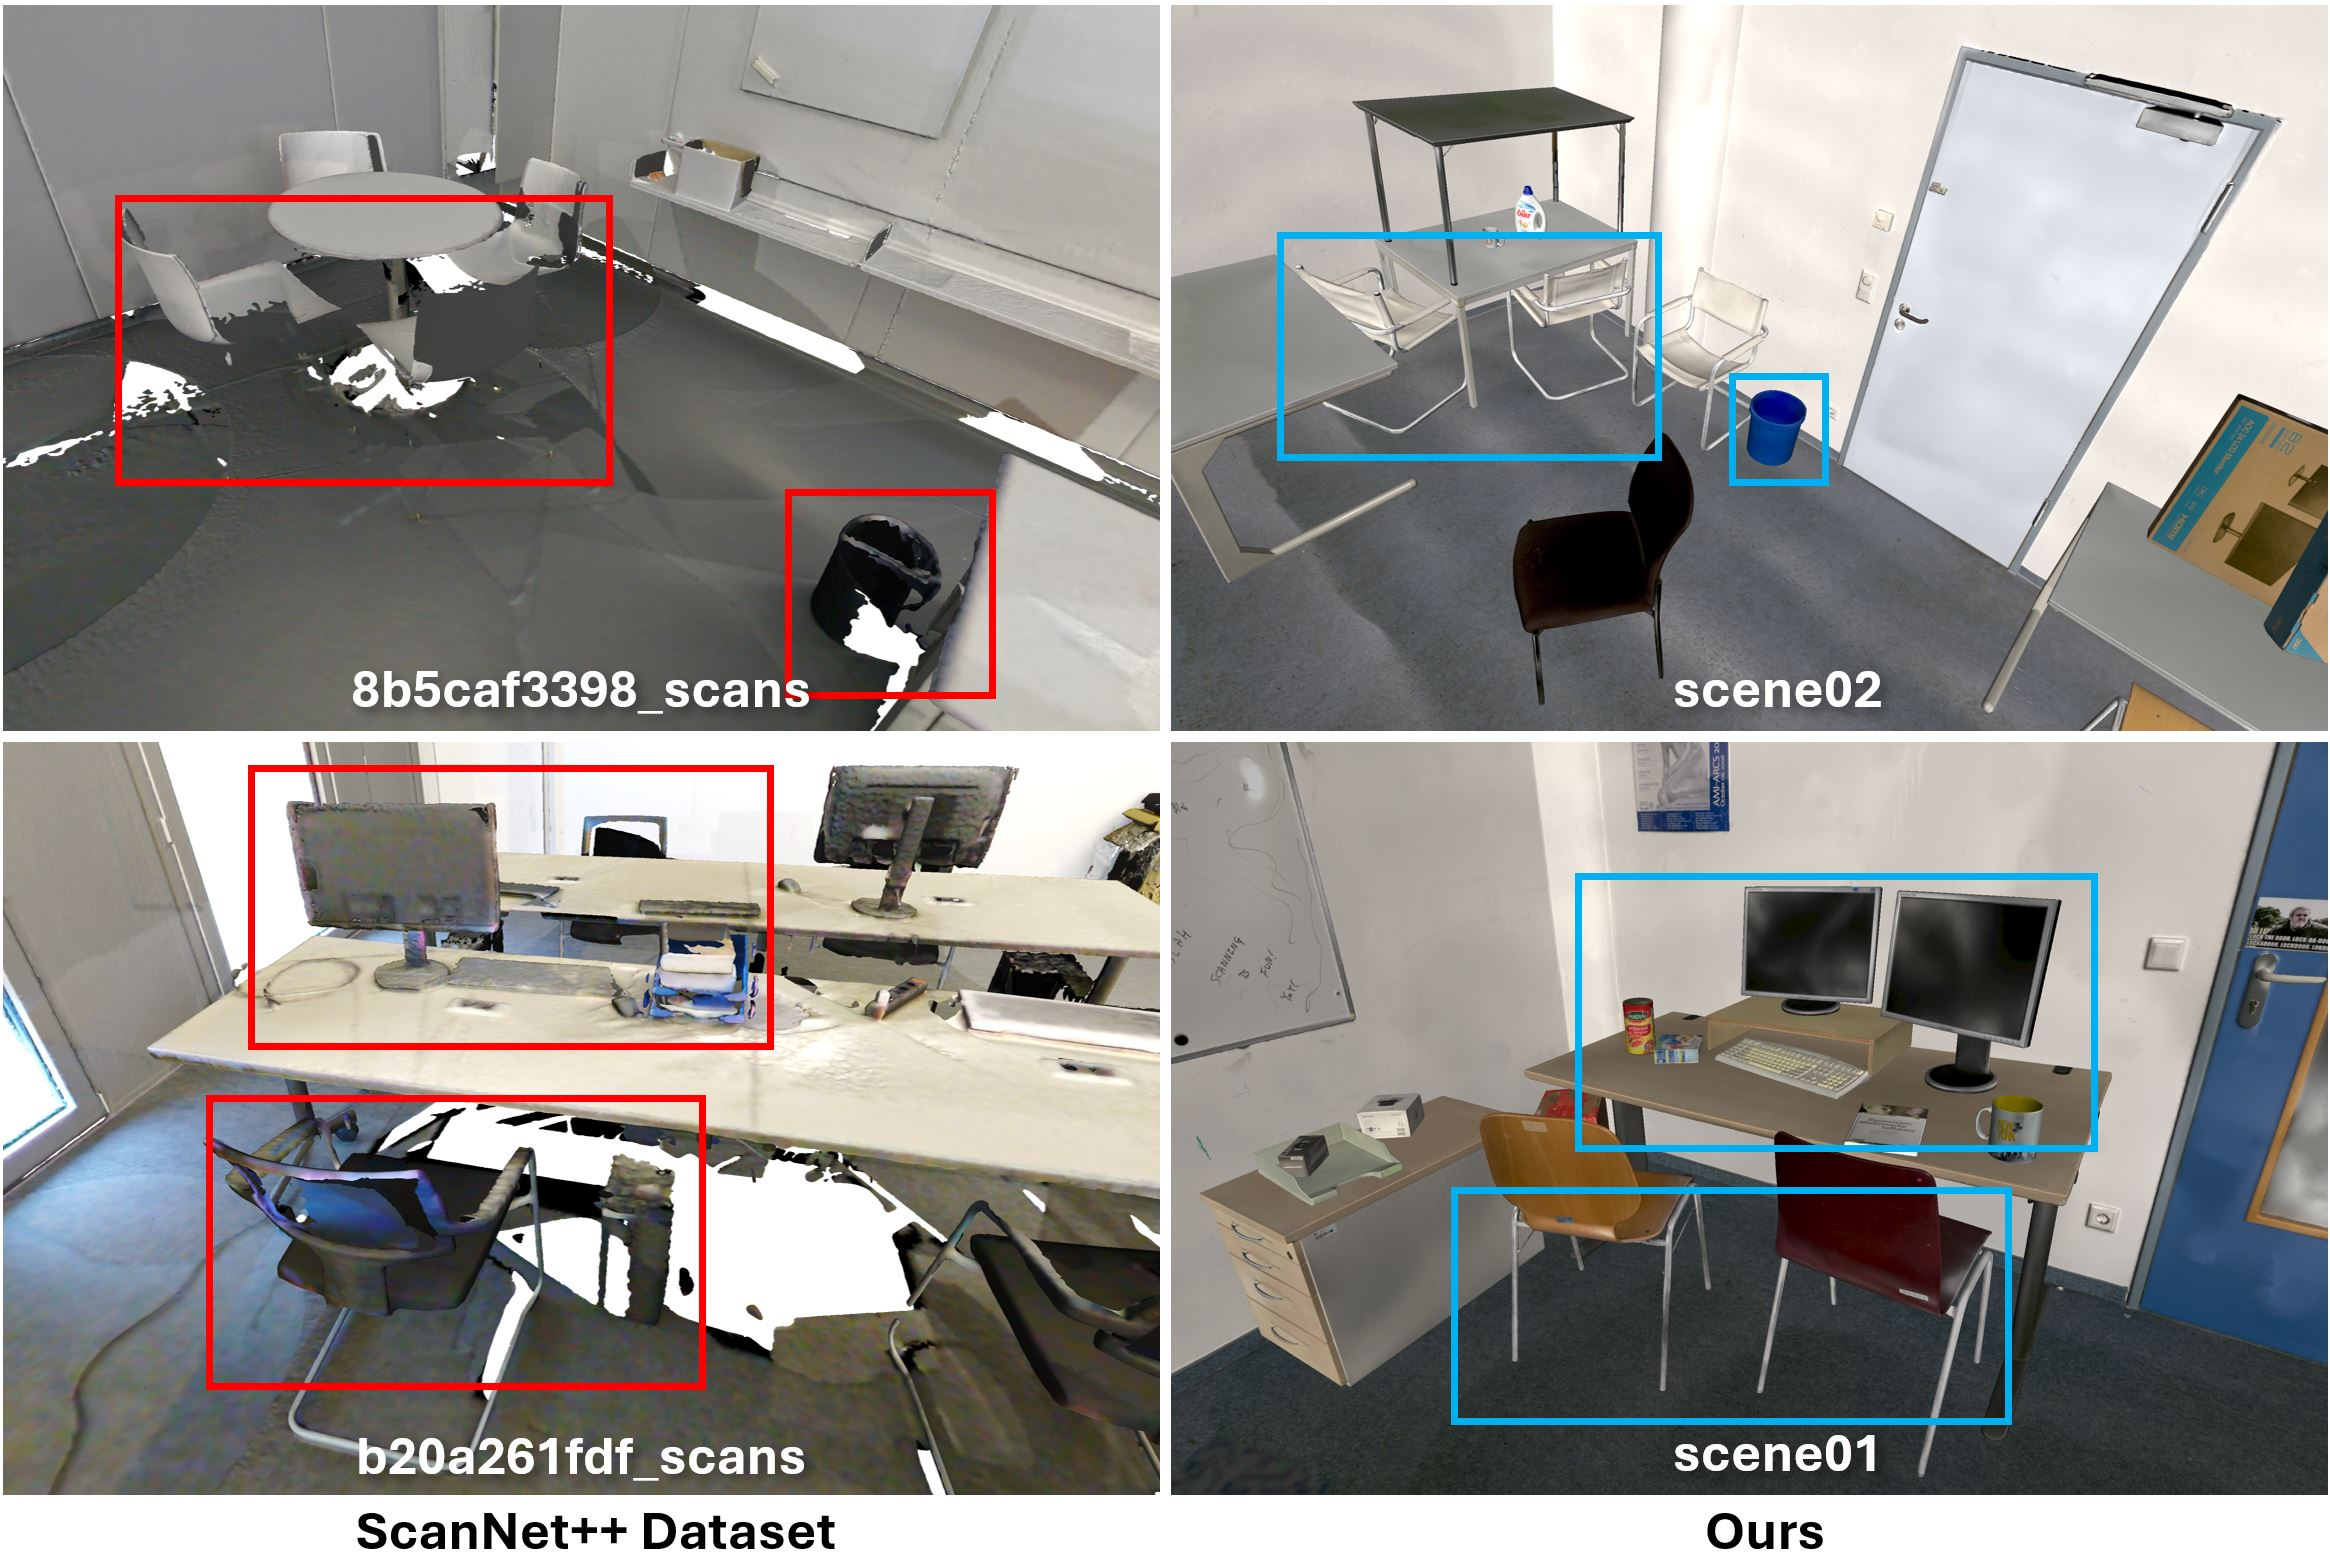}
    \caption{\textbf{ScanNet++ Dataset VS Ours.}}
    \label{fig:scannet_vs_ours}
\end{figure*}

\clearpage

Unlike ScanNet++, the Replica dataset scans the scene with a specially designed camera rig that contains multiple sensors to obtain the mesh in more detail. Also, after the scanning, a manual hole-filling process is used to complete the mesh if the missing area is part of a flat surface. For this reason, the meshes of the Replica dataset are much more complete compared to ScanNet++. However, we find that meshes in the Replica dataset in general are overly smoothed and lack details. Also there are parts missing on non-flat surfaces, such as the legs of a chair or the tab of the sink. In Fig.~\ref{fig:replica_vs_ours} we provide a comparison between the Replica dataset and our dataset. We show a kitchen scene from each dataset to demonstrate that compared with Replica our dataset contains all small details of the scene, such as the small handles of the kitchen cabinet (zoom in for more details). We also show that the legs of the chairs and table are missing in a living room scene from the Replica dataset, while our dataset contains these parts in a high quality. We also attach in detailed comparison of the datasets in our supplementary video file.

\begin{figure*}[!h]
 \centering
    \includegraphics[width=\linewidth]{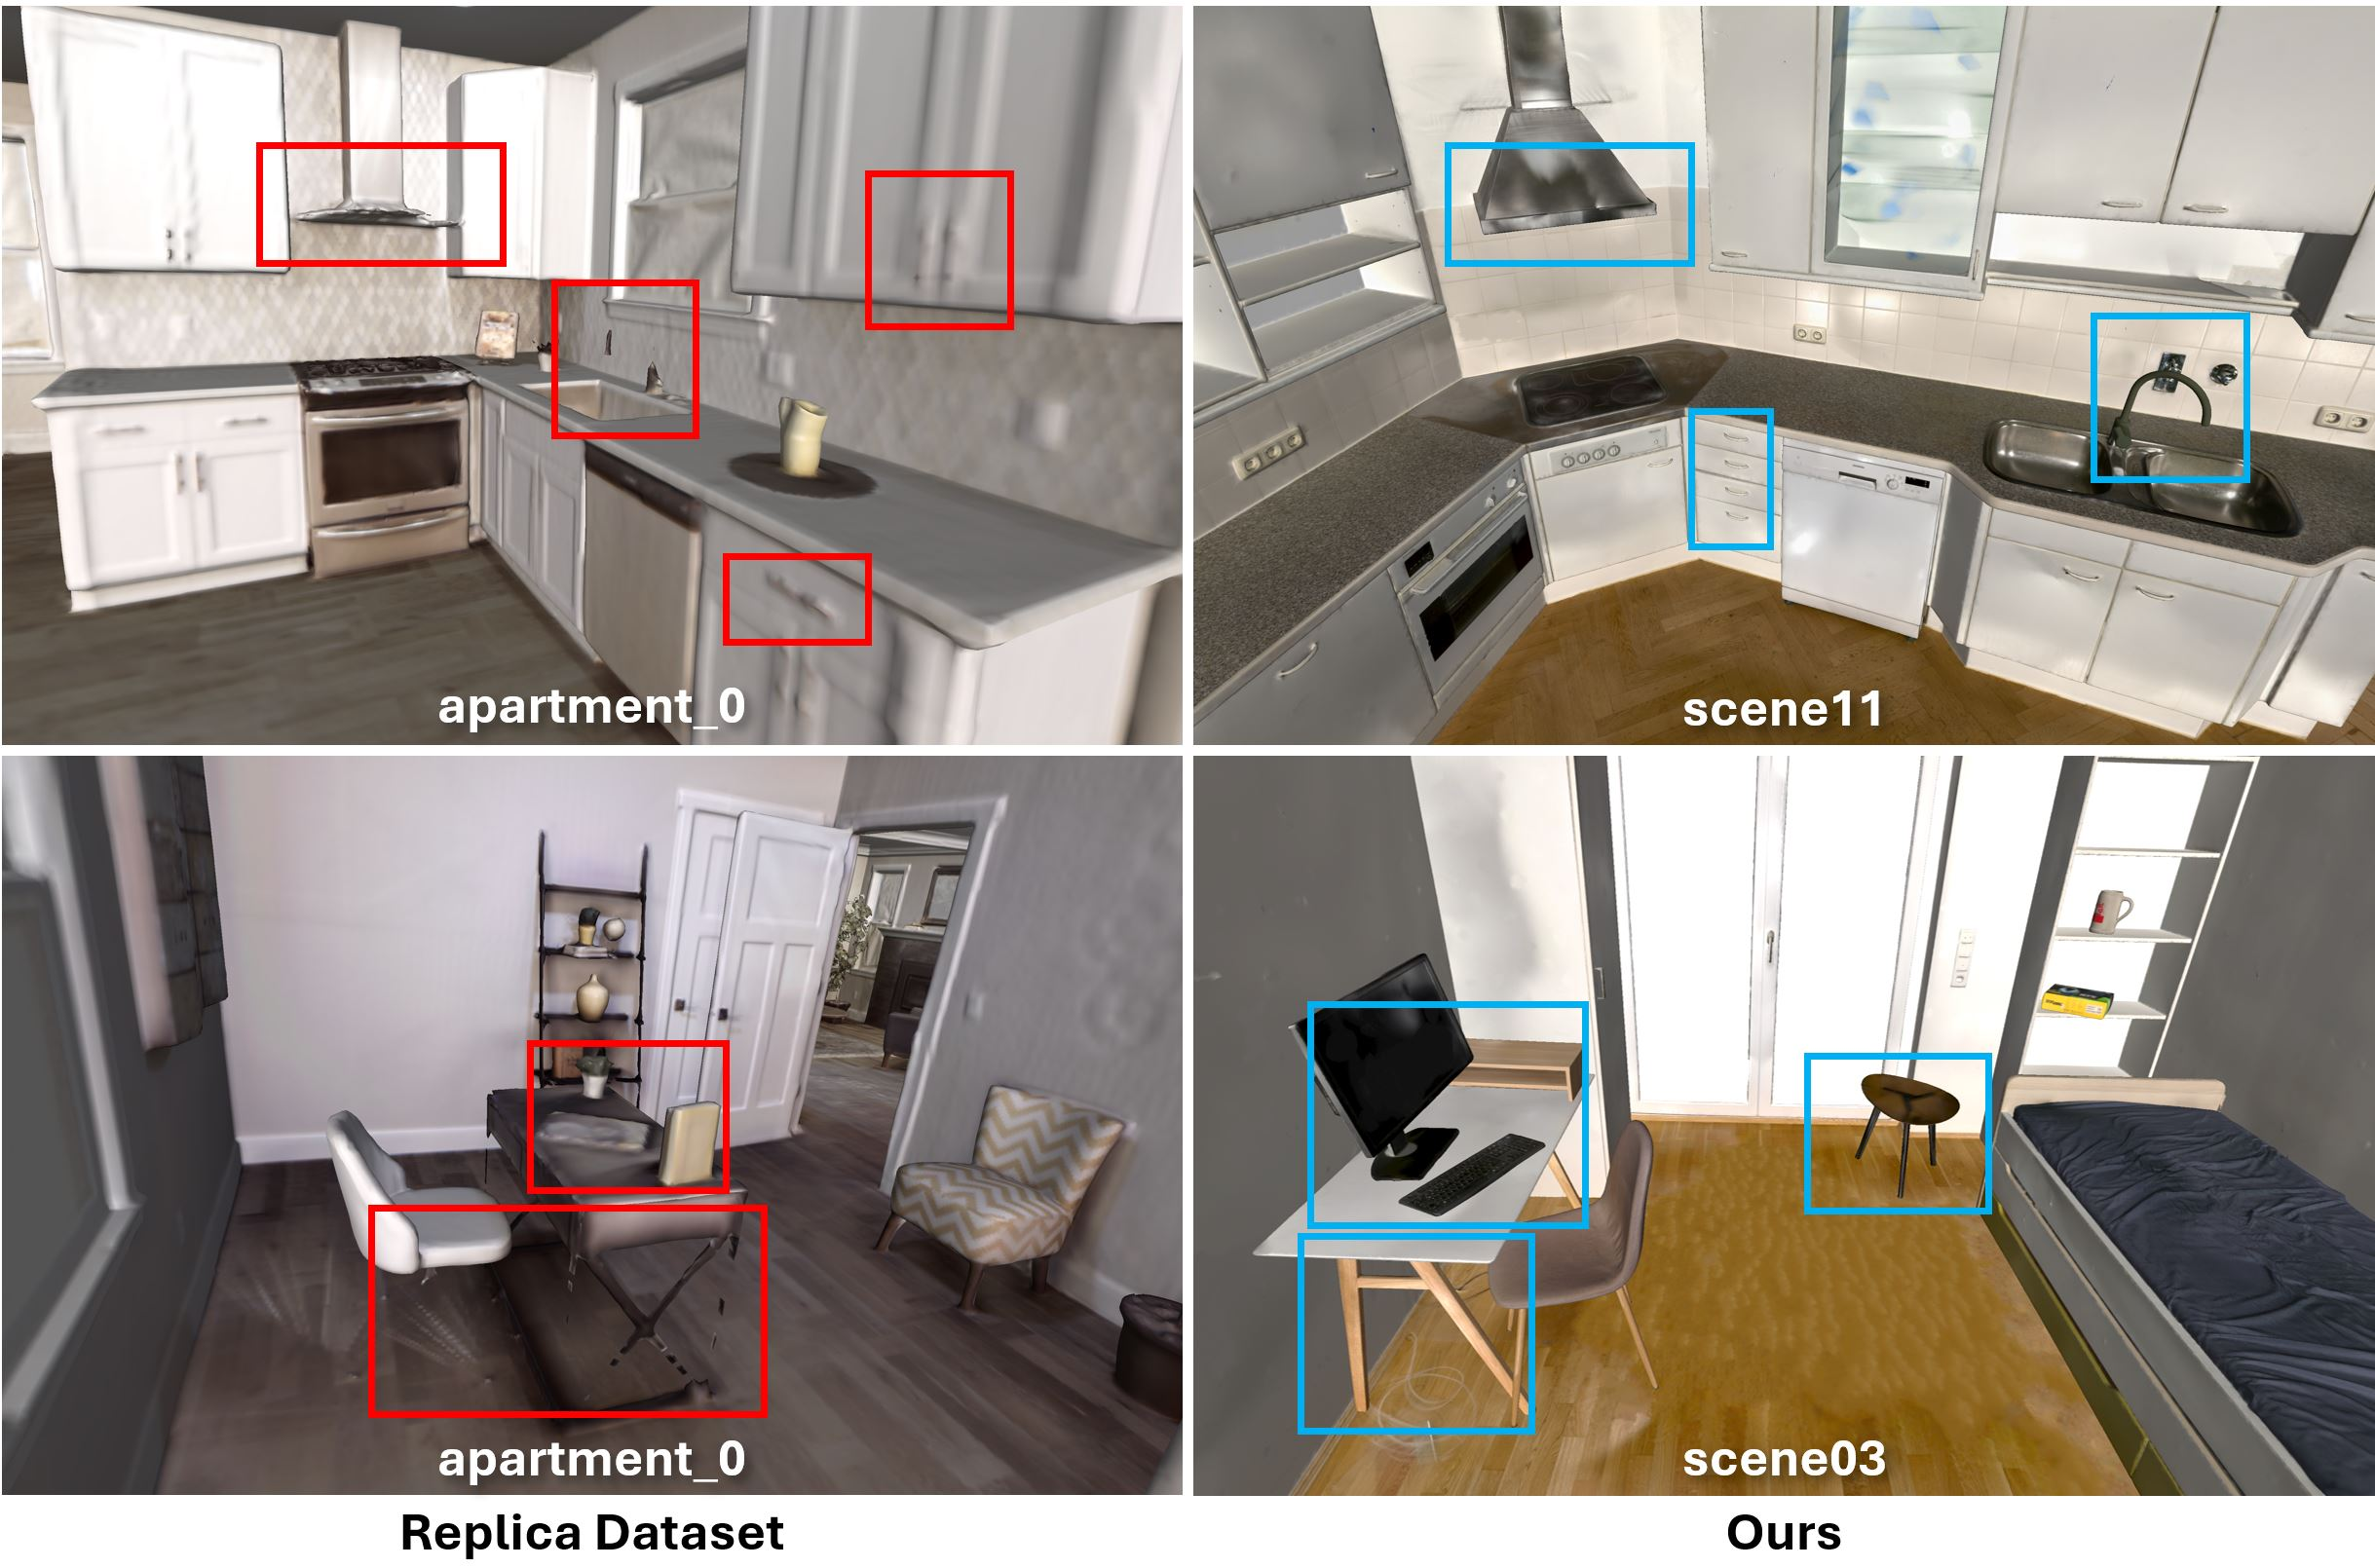}
    \caption{\textbf{Replica Dataset VS Ours.}}
    \label{fig:replica_vs_ours}
\end{figure*}

\clearpage
