# Supplementary material for: SCRREAM : SCan, Register, REnder And Map:A Framework for Annotating Accurate and Dense 3D Indoor Scenes with a Benchmark
Source: arXiv:2410.22715 source file (2025-01-06)
Supplement: Supplementary file 4 [file suppl_4_documentation.tex]

\section{Dataset Documentation} \label{sec:suppl_documentation}

Our dataset includes scene folders with 3 different conventions. Folders with the \texttt{"sceneXX"} convention contain data for the \texttt{Indoor Reconstruction and SLAM Dataset} and \texttt{Object Removal and Scene Editing Dataset}, folders with labelled \texttt{"human\_sceneXX"} contain the \texttt{Human Reconstruction Dataset} and folders named \texttt{"pose\_sceneXX"} contain the \texttt{6D Pose Estimation Dataset}. In this section, we explain the file structure of the dataset and describe the naming conventions for individual files in the folders. To access the dataset's download link as well as python code for data loading and visualization, please visit \url{https://github.com/Junggy/SCRREAM}.

\subsection{Indoor Reconstruction and SLAM Dataset and Object Removal and Scene Editing Dataset.} \label{subsec:indoor_recon}
Both the \texttt{Indoor Reconstruction and SLAM Dataset} and the \texttt{Object Removal and Scene Editing Dataset} follow the same format. The \texttt{"sceneXX"} folders contain 3 sub-folders: \texttt{"meshes"}, \texttt{"sceneXX\_full\_XX"} and \texttt{"sceneXX\_reduced\_XX"}. 

The \texttt{"meshes"} folder contains independent meshes of the full scene that are aligned w.r.t. world coordinate system as \texttt{"*.obj"} files. Therefore loading all meshes together shows the full scene in the world coordinate system. Each mesh file follows a naming convention of \texttt{"\{class\_name\}-\{instance\_name\}.obj"}. For example, a monitor object with of the old\_tall instance is named \texttt{"monitor-old\_tall.obj"}. This naming convention allows easy identification of both class and instance of the objects in the scene.

The \texttt{"sceneXX\_full\_XX"} and \texttt{"sceneXX\_reduced\_XX"} folders contain the data regarding the image sequences, such as \texttt{"camera\_pose"}, \texttt{"depth\_d435"}, \texttt{"depth\_gt"}, \texttt{"depth\_tof"}, \texttt{"instance"}, \texttt{"pol"}, \texttt{"rgb"}, \texttt{"sparse"}, \texttt{"intrinsics.txt"}, \texttt{"meta.txt"} and \texttt{"video.avi"}. The detailed folder layout is shown in Fig.~\ref{fig:indoor_scene_file_layout}. Both full scene and reduced scene have the same file structure. Metadata from \texttt{"meta.txt"} can be used to identify the removed objects in the reduced scenes.

\begin{figure*}[!b]
 \centering
    \includegraphics[width=\linewidth]{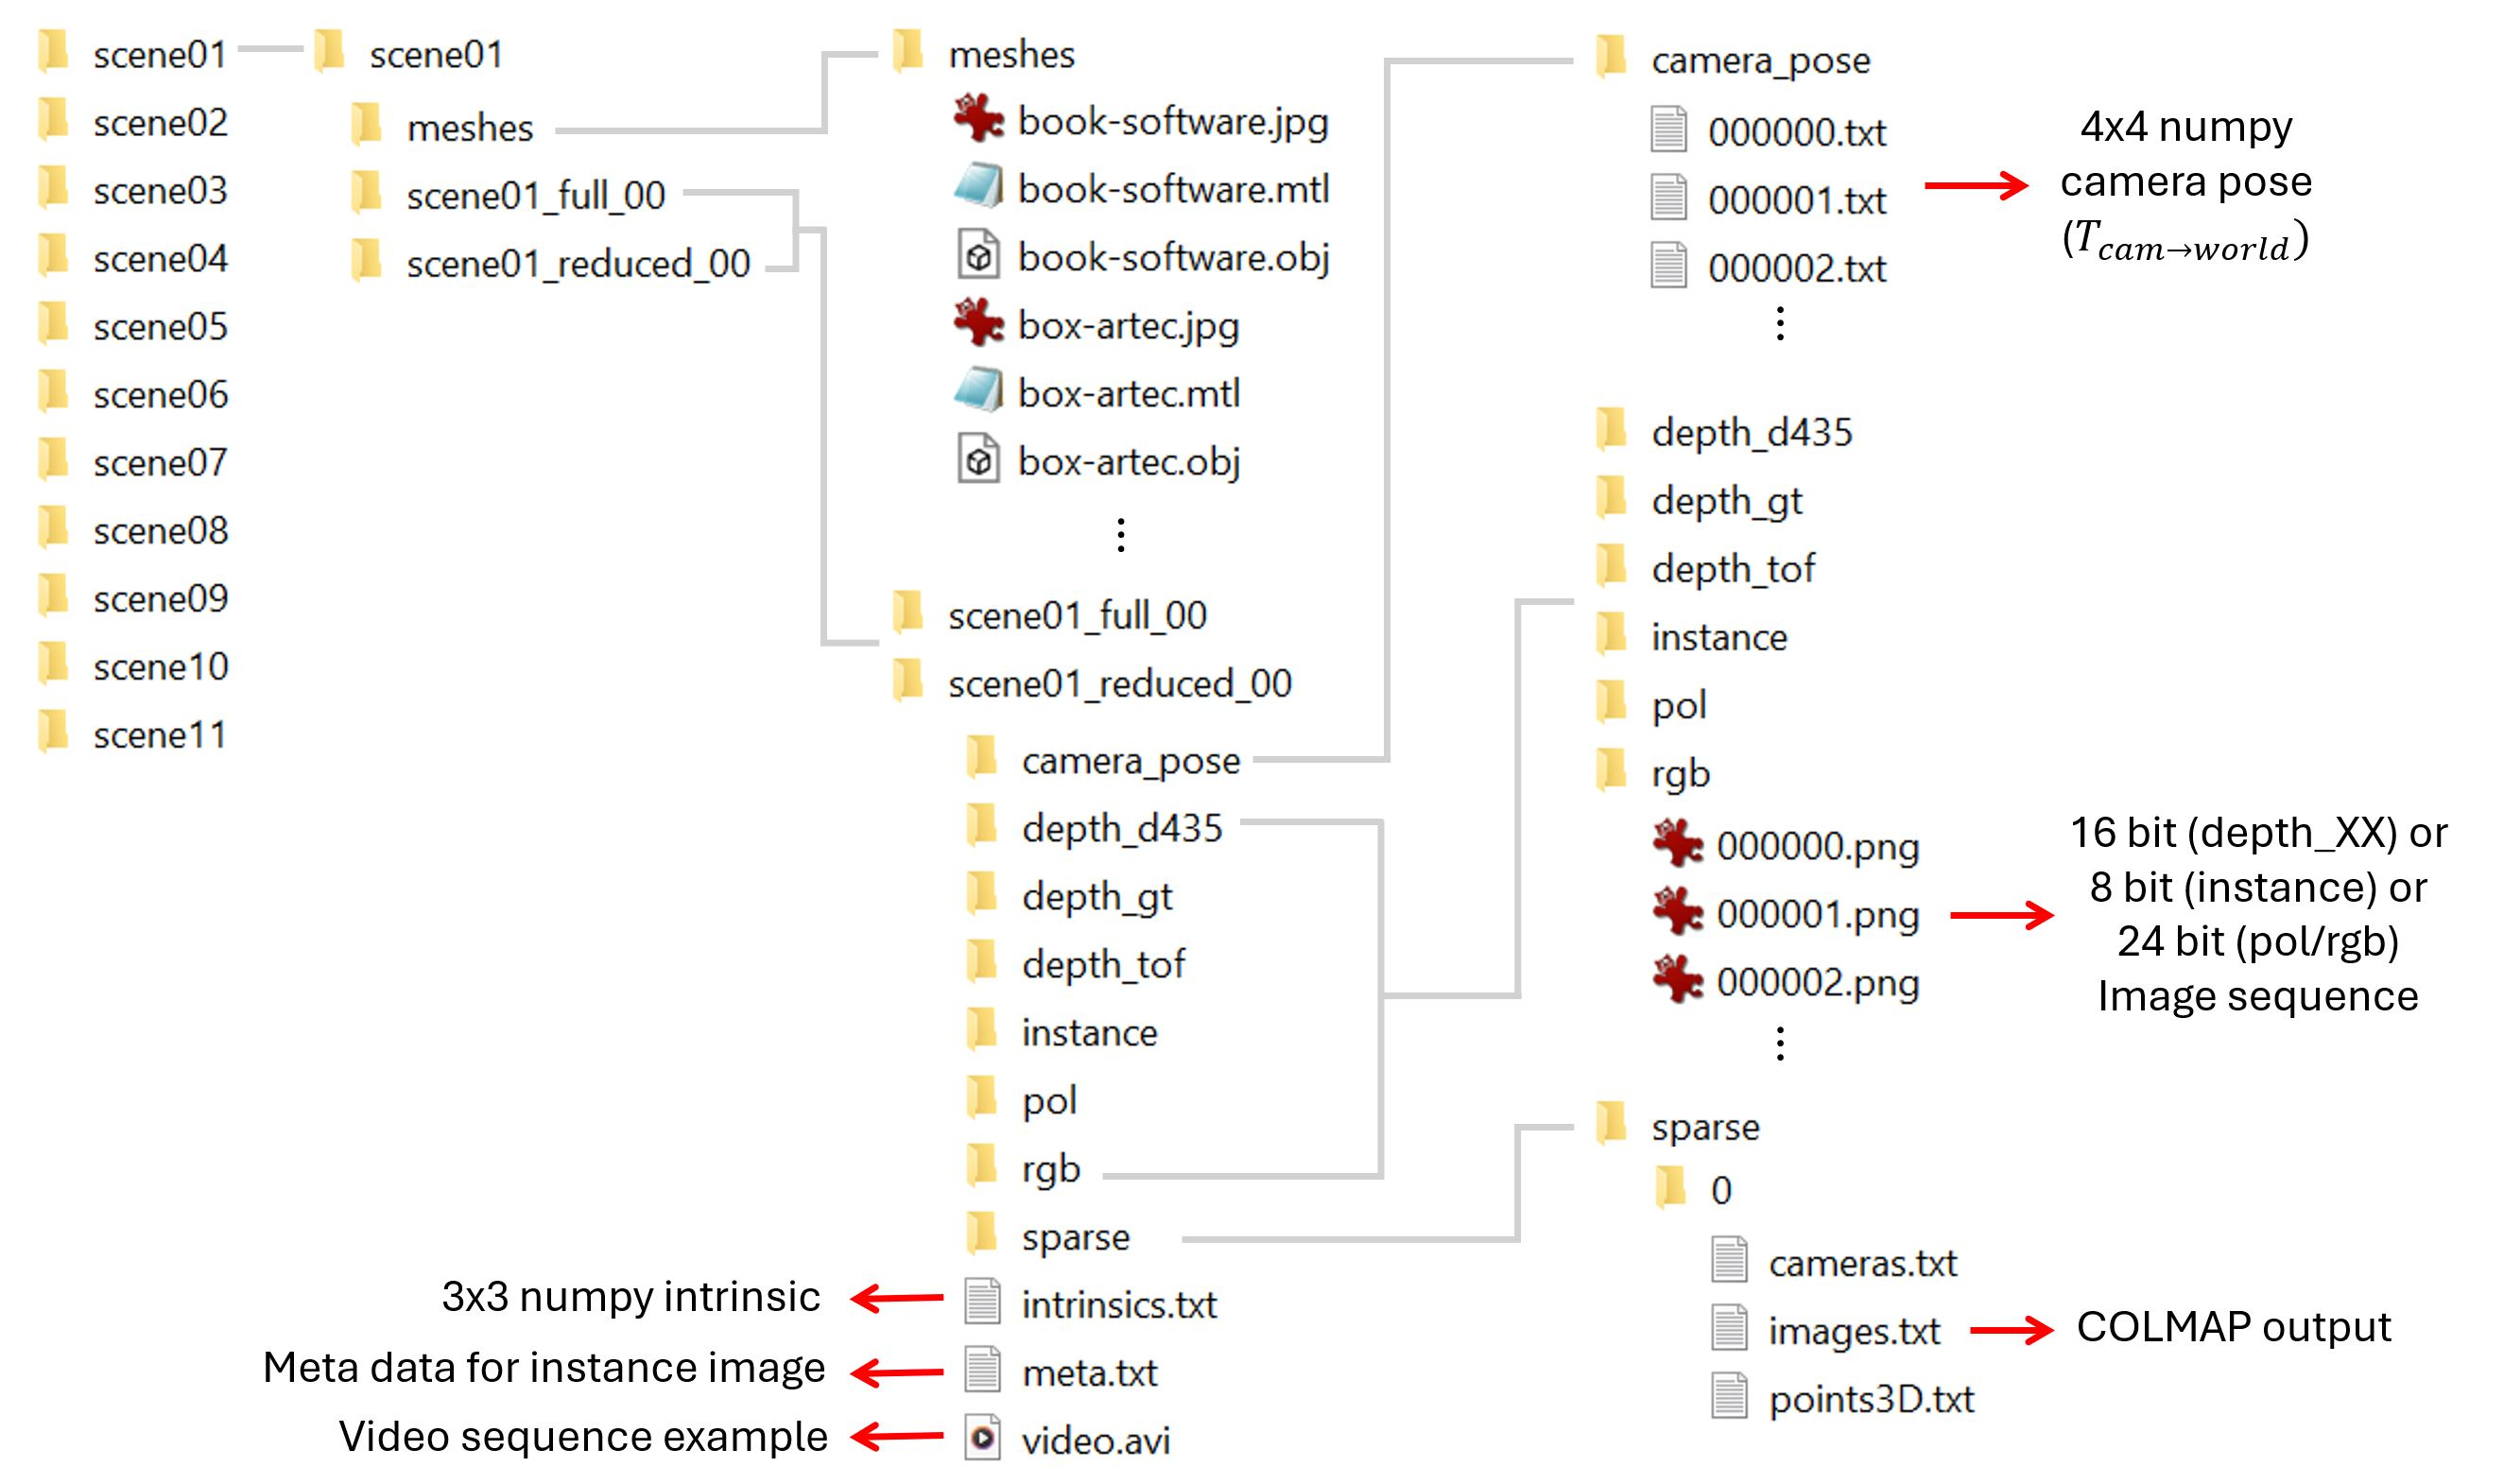}
    \caption{\textbf{File Structure of the Indoor Reconstruction and SLAM Dataset and Object Removal and Scene Editing Dataset.}}
    \label{fig:indoor_scene_file_layout}
\end{figure*}

The \texttt{"camera\_pose"} folder contains the camera pose for each image frame in the 4x4 matrix format saved as numpy matrix in a text file. The camera pose's definition is \(T_{cam->world}\), meaning that each frame's translation element refers to the camera center in the scene. The matrix can be loaded with the \texttt{"np.loadtxt"} function.

The \texttt{"depth\_d435"}, \texttt{"depth\_gt"}, \texttt{"depth\_tof"} folders contain the depth images for each image frame. Each depth image is saved as a 16bit image in \(mm\) units meaning that pixel value 1000 represents 1 meter. The depth images can be loaded in meter units by using opencv-python's \texttt{"cv2.imread"} function, \texttt{"cv2.imread("XXXXXX.png",-1).astype(np.uint16)/1000"}. Images from both the \texttt{"depth\_d435"} and \texttt{"depth\_tof"} folders are obtained from the real depth sensors and warped or aligned to the RGB image in a forward manner (e.g. forward-warping) using their own depth values, the extrinsic calibration matrix and RGB sensor's intrinsic matrix. Note that due to sensor noise, the warped depth are often not well aligned to the corresponding RGB image. Images in the \texttt{"depth\_gt"} folder are the ground truth depth maps that are rendered from the object meshes and camera poses and serve as absolute ground truth for the depth evaluation benchmark.

The \texttt{"instance"} folder contains the corresponding instance segmentation images for the given RGB frames. The segmentation is obtained by rendering the individual objects with a unique value using the camera pose and intrinsic matrix. The mapping between the pixel values and object instances is provided in the \texttt{"meta.txt"} file. We keep the same mapping between the full and reduced scenes for convenience. 

The \texttt{"meta.txt"} file contains the metadata that is mapping between the instance pixel values and the object meshes in the scene. Each line of metadata follows the convention of \texttt{"\{class\_name\} \{mesh\_name\} \{pixel\_value\}"}. For example if the pixel value of \texttt{"keyboard-grey\_old"} is 165 in the instance image, its written as \texttt{"keyboard keyboard-grey\_old 165"}. With this, one can convert the instance segmentation image into a class segmentation image. Note that this metadata shares the same mapping value per scene, for example \texttt{"room room-office 240"} is in the metadata from both \texttt{"scene01\_full\_00"} and \texttt{"scene01\_reduced\_00"}, while as \texttt{"keyboard-grey\_old"} is not present in \texttt{"scene01\_reduced\_00"}, the metadata does not contain \texttt{"keyboard keyboard-grey\_old 165"} (Fig.~\ref{fig:metadata_example}).

\begin{figure*}[!h]
 \centering
    \includegraphics[width=\linewidth]{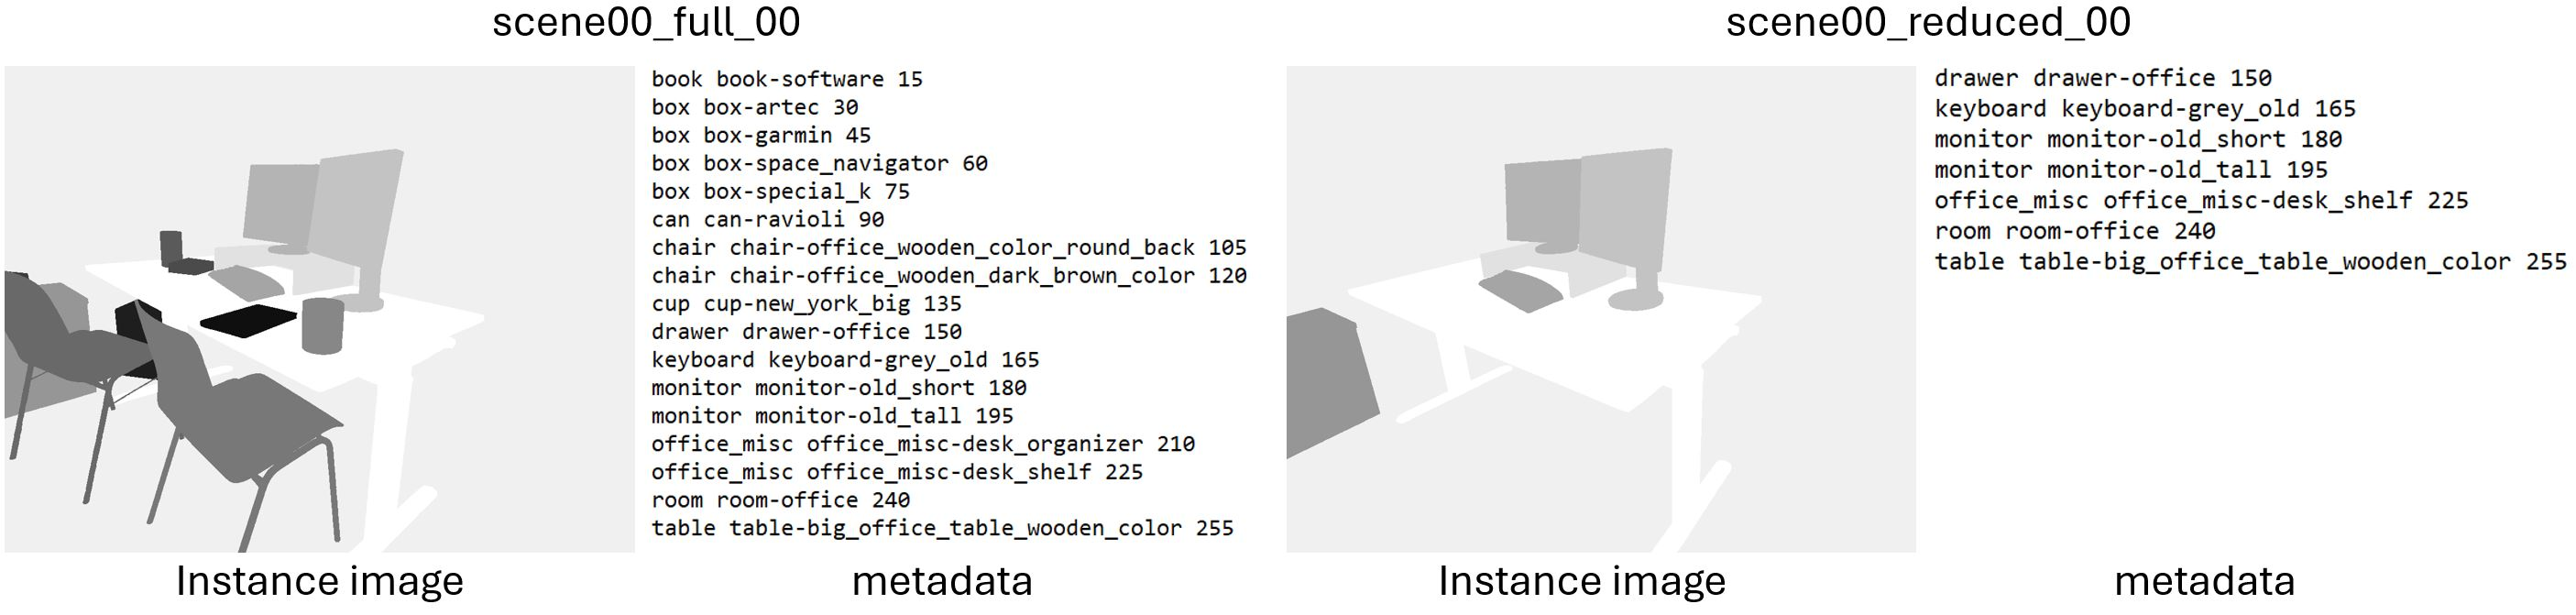}
    \caption{\textbf{Example of Instance Segmentation and Metadata Mapping for a Full and Reduced Scene.}}
    \label{fig:metadata_example}
\end{figure*}

The \texttt{"pol"} folder contains polarimetric images obtained from the Lucid Phoenix polarization camera. Polarimetric images are stored as 4 RGB images with 4 different polarization angles (0,45,90,135 degree) arranged in a clockwise manner starting from the left top side. All 4 images are un-distorted so that no distortion coefficient is needed and intrinsic matrix is saved in \texttt{"intrinsics.txt"}.

The \texttt{"rgb"} folder contains the RGB image sequence. The RGB images are obtained by averaging the 4 polarization images and share the same intrinsics as \texttt{"intrinsics.txt"}.

The \texttt{"sparse"} folder contains the COLMAP~\cite{colmap_1,colmap_2} output that is obtained by running COLMAP with the ground truth camera pose. We fix the camera poses to keep the scale unchanged. We specifically provide this folder to make our dataset compatible with 3D Gaussian Splatting~\cite{kerbl3Dgaussians} variants.

The \texttt{"video.avi"} is an example video that serves as qualitative evaluation of the camera trajectory as well as annotation quality. The video contains the visualization of depth maps and depth error and the instance image overlaid on the RGB image as shown in Fig.~\ref{fig:video_example}.

\begin{figure*}[!h]
 \centering
    \includegraphics[width=\linewidth]{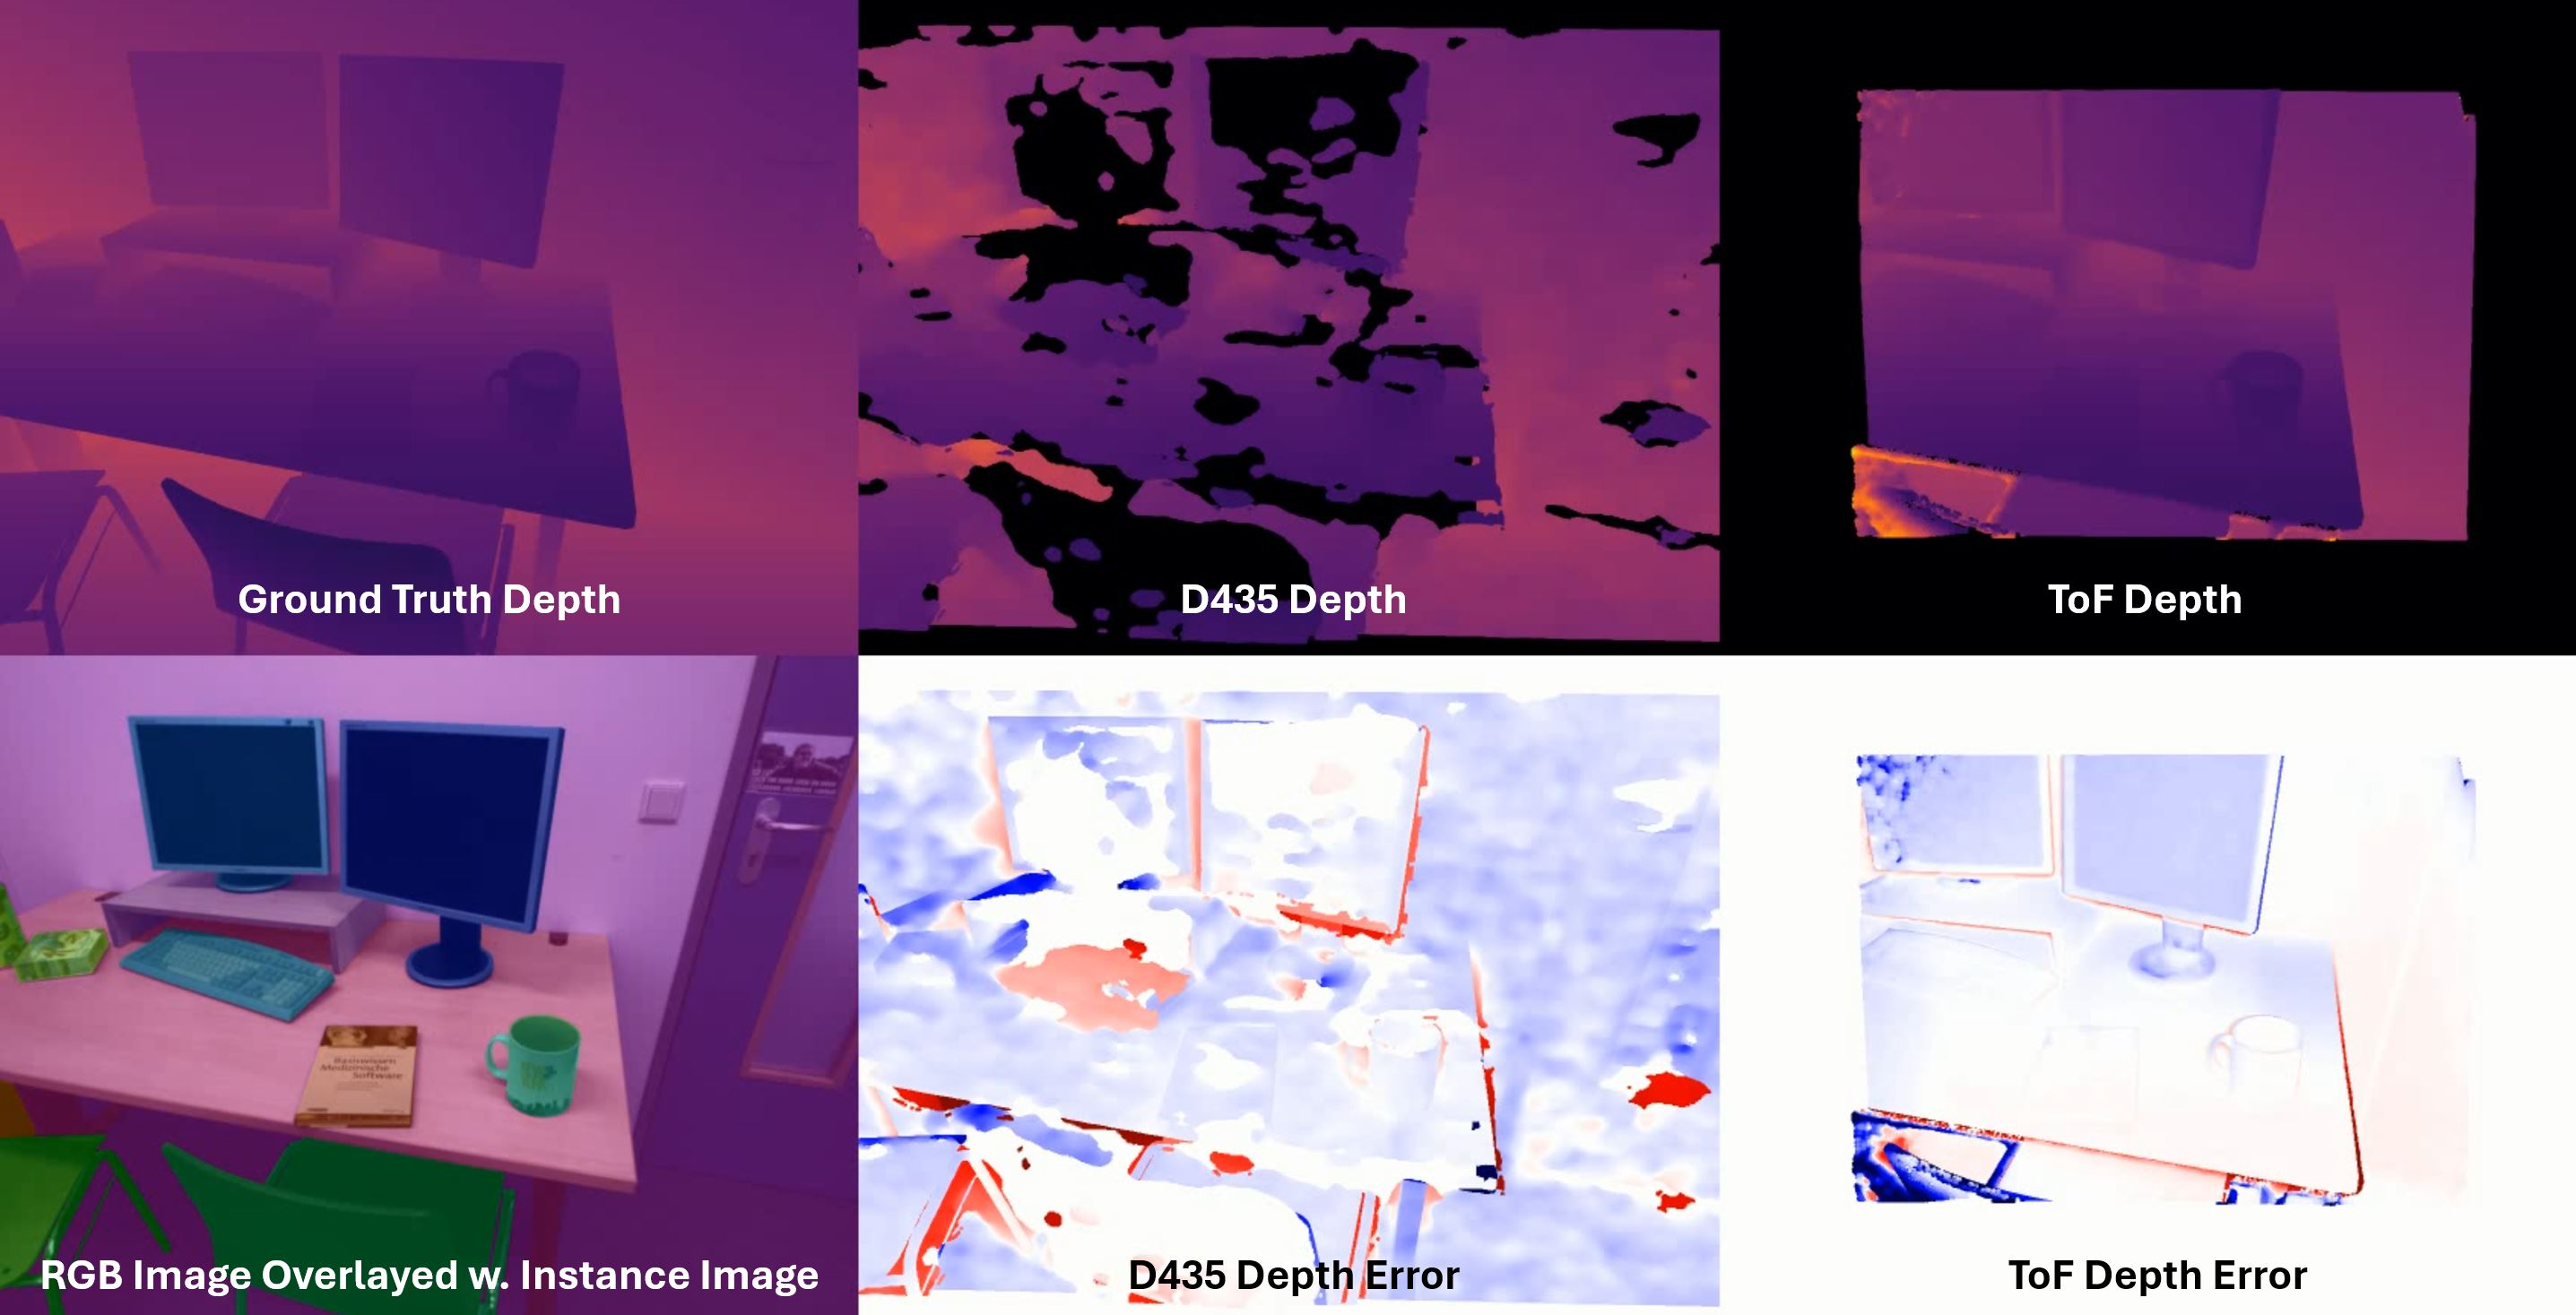}
    \caption{\textbf{Example of the \texttt{video.avi}} layout.}
    \label{fig:video_example}
\end{figure*}

%\textbf{Indoor Reconstruction and SLAM Dataset a} Indoor reconstruction and SLAM dataset follows name convention \texttt{sceneXX}

\subsection{Human Reconstruction Dataset} \label{subsec:human_recon}
The \texttt{Human Reconstruction Dataset} shares a similar file structure as the \texttt{Indoor Reconstruction and SLAM Dataset} and the \texttt{Object Removal and Scene Editing Dataset}. There a are few differences in the folder arrangement as well as file naming convention as 4 images are captured per human posture. See Fig.~\ref{fig:human_scene_layout} for an overview.

\begin{figure*}[!b]
 \centering
    \includegraphics[width=\linewidth]{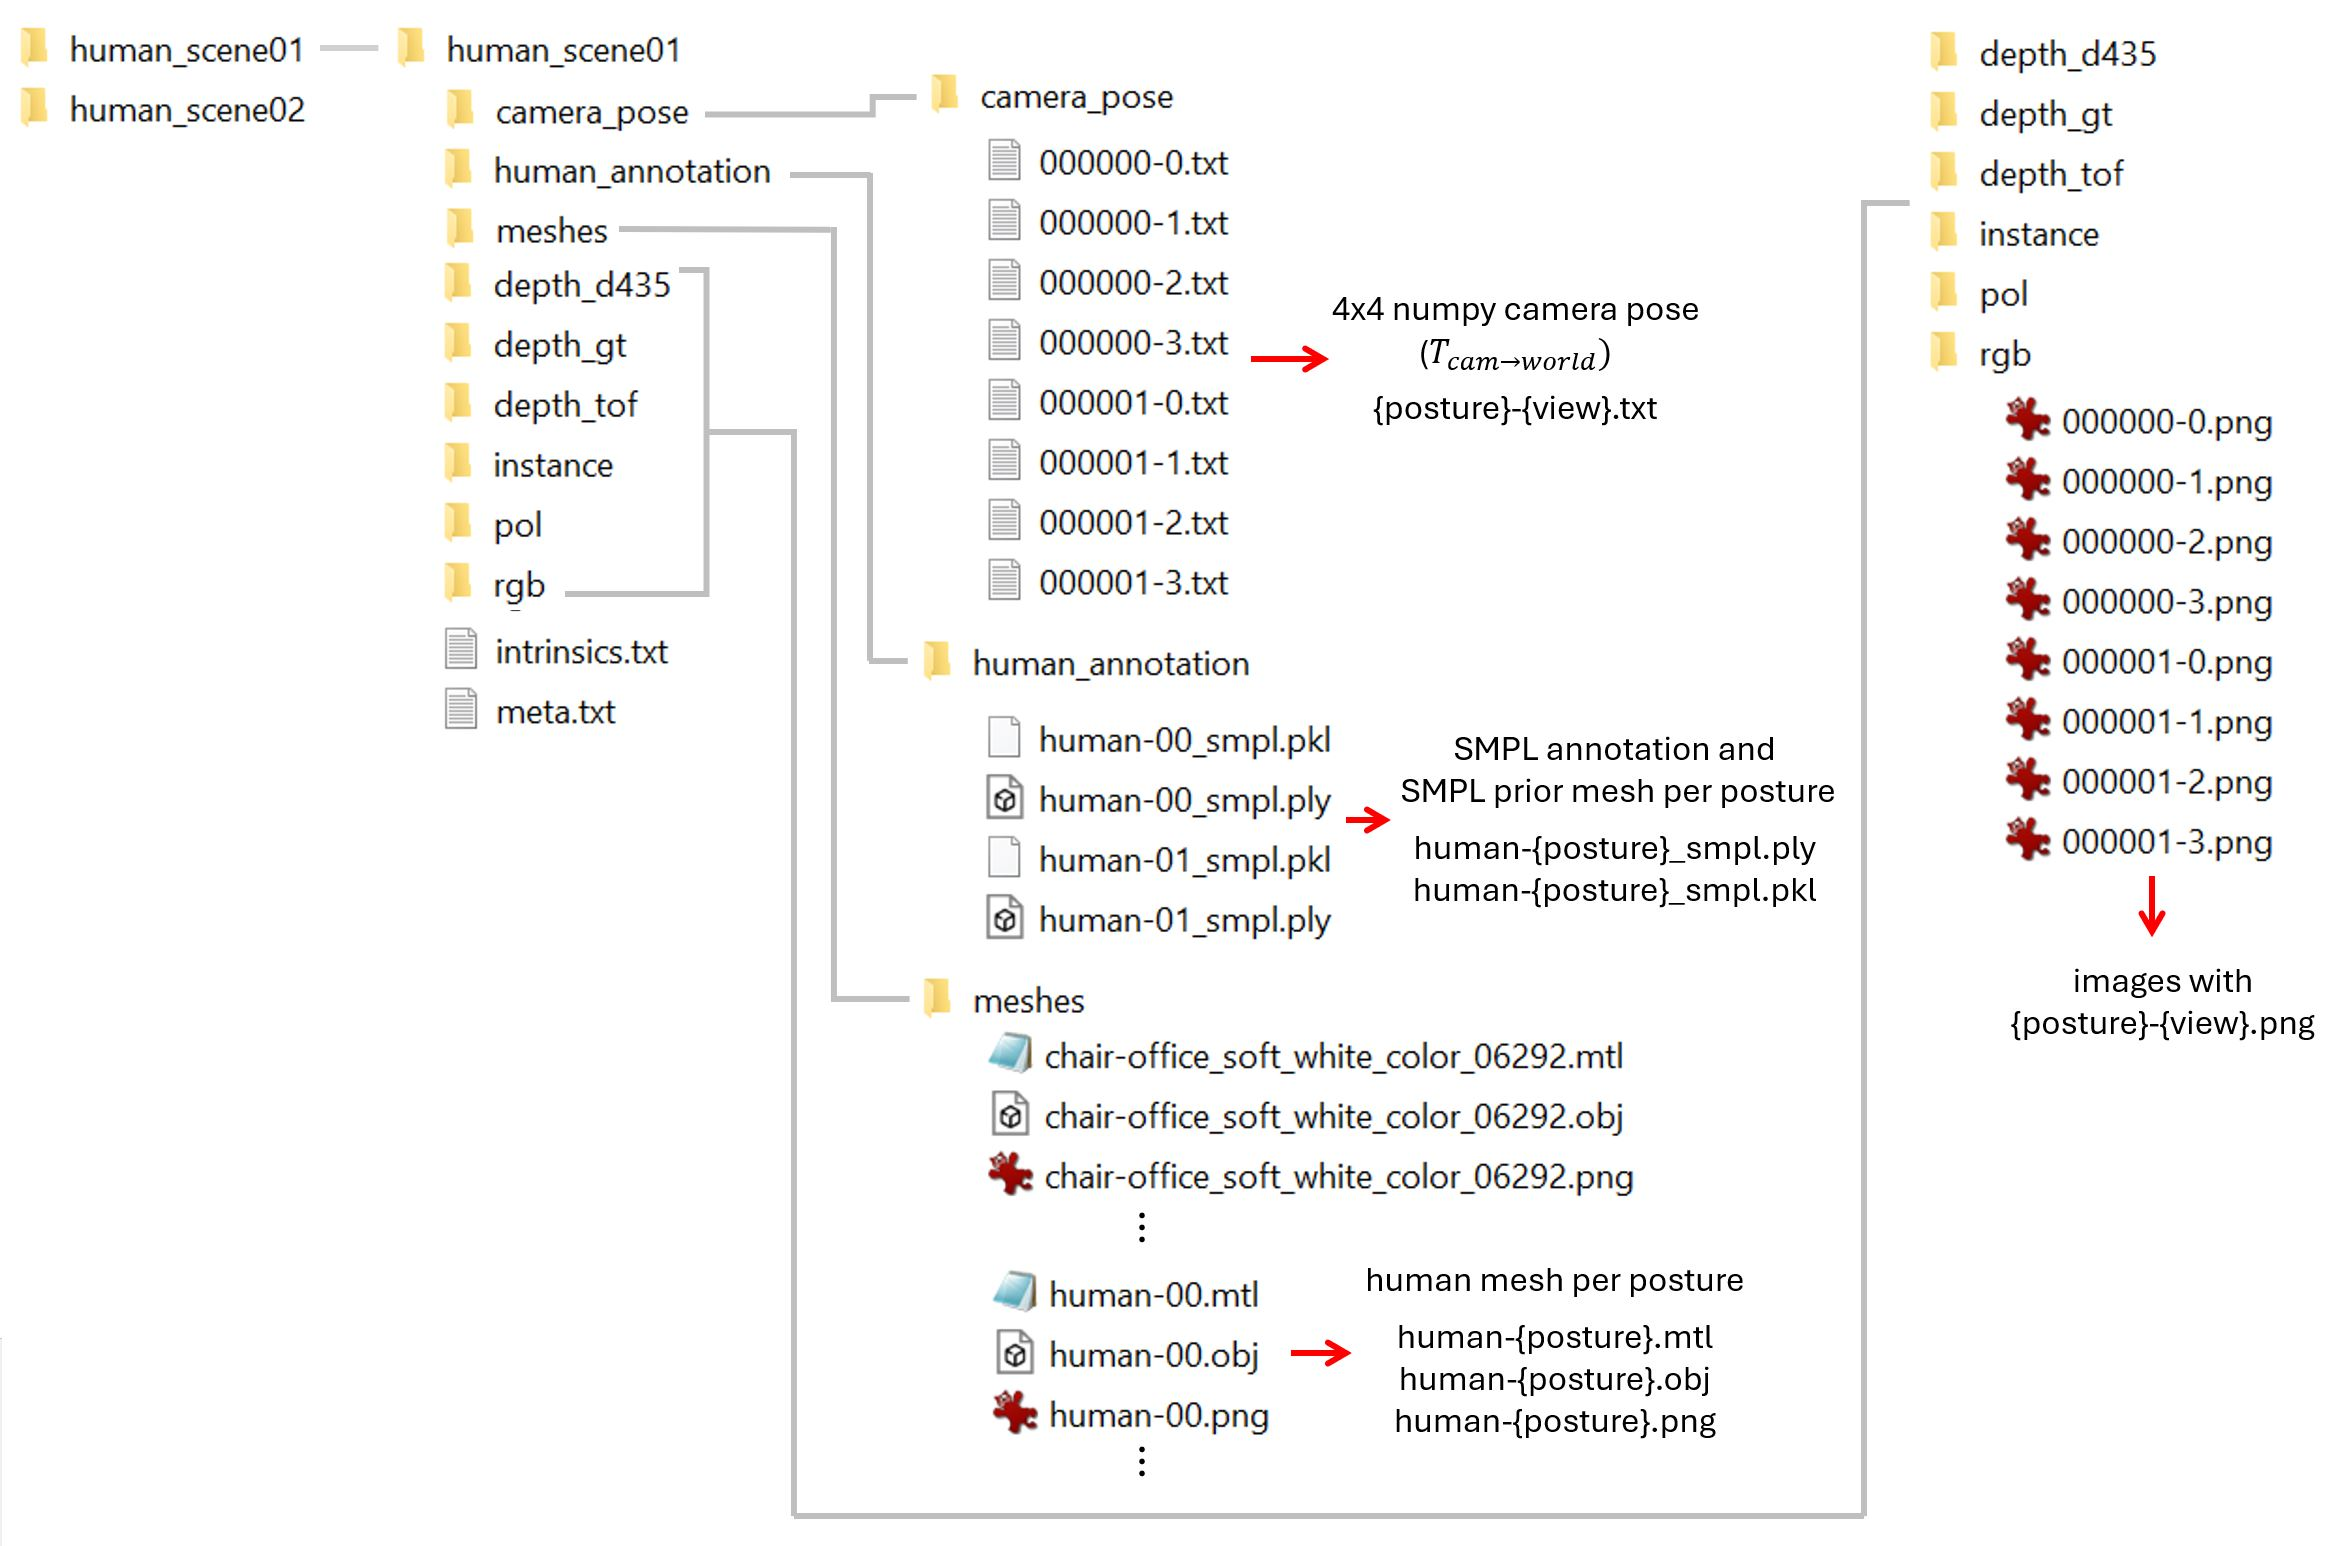}
    \caption{\textbf{File Structure of the Human Reconstruction Dataset.}}
    \label{fig:human_scene_layout}
\end{figure*}

The \texttt{"meshes"} folder contains the meshes of the scene as in the previous dataset setup. However, the folder contains all human meshes from different postures as well. We capture 45 postures for \texttt{"human\_scene\_01"} and 37 postures for  \texttt{"human\_scene\_02"}. Each human posture is scanned with the hand-held scanner in a high resolution and water-tight manner like the other objects meshes and we save the mesh with the naming convention \texttt{"human-\{posture\}.obj"}.

The \texttt{"human\_annotation"} folder contains SMPL~\cite{SMPL:2015} parameter annotations for each human posture. The \texttt{*.pkl"} files contain SMPL annotations as a python pickle file and the \texttt{*.ply"} files are the SMPL vertices / mesh generated from the pickle file. Both files follow the convention of \texttt{"human-\{posture\}\_smpl"} with extension of \texttt{*.pkl"} and \texttt{*.ply"}. The \texttt{*.pkl"}'s SMPL annotation follows the same convention as in~\cite{bhatnagar2020ipnet, bhatnagar2020loopreg} that contains a 72 channel vector for the \texttt{"pose"} (first 3 channels are for \texttt{"global\_orient"}, the remaining 69 channels are for the \texttt{"body\_pose"}), a 300 channel vector for the shape \texttt{"betas"} and a 3 channel vector for the translation \texttt{"trans"}.

The \texttt{"camera\_pose"} folder contains the camera pose for each image frame in the 4x4 matrix format as in the reconstruction and SLAM dataset. However, as the human dataset captures 4 multi-view images on single human posture, it contains 4 poses per posture. Camera poses files are saved with the convention \texttt{"\{posture\}-\{view\}.txt"}. 

All image files including depths, RGBs, instances are saved the same way as in the Reconstruction and SLAM dataset but saved with the same convention as for the camera poses due to the 4 multi-view images captured per human posture. All images follow the same convention of \texttt{"\{posture\}-\{view\}.png"}.

While \texttt{"meta.txt"} has the same mapping information as in the previous dataset setup, plus the humans with the convention of \texttt{"human 00 \{pixel\_value\}"}. For the humans no mesh name is provided in the middle as there are multiple human meshes per scene but all share the same pixel value in the instance images throughout the same scene. 

\subsection{6D Pose Estimation Dataset} \label{subsec:6d_pose}
The contents in the \texttt{"6D Pose Estimation Dataset"} share the same principle as in the \texttt{Indoor Reconstruction and SLAM Dataset} and \texttt{Object Removal and Scene Editing Dataset} for the image folders (\texttt{"depth\_d435"}, \texttt{"depth\_gt"}, \texttt{"depth\_tof"}, \texttt{"depth\_instance"}, \texttt{"pol"}, \texttt{"rgb"}), \texttt{"intrinsics.txt"} and \texttt{"meta.txt"} files, while it contains additional folders, such as \texttt{"pose\_meshes\_canonical"} and \texttt{"labels"} for the 6D pose annotation. An overview of the file structure is shown in Fig.~\ref{fig:pose_scene_layout}.

The \texttt{"pose\_meshes\_canonical"} folder contains the meshes of the target objects for the pose estimation in canonical orientation in contrast to the meshes in \texttt{"meshes"} in the other dataset format that are defined in world coordinates. The canonical meshes are self-centered (object center is in the center of it's bounding box) and follow specific orientation convention per class or category (Fig.~\ref{fig:mesh_canonical}, (a)), while the meshes from the previous dataset are centered and oriented according to their layout in the scene (Fig.~\ref{fig:mesh_canonical}, (b)). Although they have differences in their orientation, we follow the same naming convention as \texttt{"\{class\_name\}-\{instance\_name\}.obj"}.

The \texttt{"labels"} folder contains the 6D pose annotation information as a pickle file with the convention of \texttt{"\{frame\}\_label.pkl"}. We provide the pickle file in a similar format as the NOCS~\cite{nocs} dataset's labels. Each pickle file contains a python dictionary of the following keys : \texttt{"model\_list"}, \texttt{"instance\_ids"}, \texttt{"class\_ids"}, \texttt{"scales"}, \texttt{"rotations"}, \texttt{"translations"}, \texttt{"bboxes"}, \texttt{"gt\_scales"}. 

\begin{enumerate}
    \item \texttt{"model\_list"} is a python list containing a tuple of each object's name and pixel value in the instance image, such as \texttt{[(\{obj\_1\_name\}, \{instance\_value\_1\}),(\{obj\_2\_name\}, \{instance\_value\_2\}) ... ]}. 

    \item \texttt{"instance\_ids"} is a python list containing the instance value per object in the same order as \texttt{"model\_list"}, such as \texttt{[\{instance\_value\_1\}, \{instance\_value\_2\} ... ]}.

    \item \texttt{"class\_ids"} is a python list containing the mapping between the class name and a predefined class id in the same order,  such as \texttt{[\{class\_id\_1\}, \{class\_id\_2\} ... ]}.

    \item \texttt{"scales"} is a python list containing the diagonal length of each object in the same order, such as \texttt{[\{diag\_length\_1\}, \{diag\_length\_2\} ... ]}.

    \item \texttt{"rotation"} is a numpy array of shape \((n\_{objects}, 3, 3)\) that is an array of rotation matrices for each object stacked along the first dimension in the same order.

    \item \texttt{"translation"} is a numpy array of shape \((n\_{objects}, 3)\) that is an array of translation vectors for each object stacked along the first dimension in the same order.

    \item \texttt{"bboxes"} is a numpy array of shape \((n\_{objects}, 4)\) that is an array of 2D bounding box annotations in the format \texttt{[\{top\_left\_y\},\{top\_left\_x\},\{bottom\_right\_y\},\{bottom\_right\_x\}]} stacked along the first dimension in the same order.

    \item \texttt{"gt\_scales"} is a numpy array of shape \((n\_{objects}, 3)\) that is an array with the mesh size in the format \texttt{[\{size\_x\},\{size\_y\},\{size\_z\}]} stacked along the first dimension in the same order.
\end{enumerate}

% {'model_list': [('bottle-evian_red', 51), ('remote-tv_white_quelle', 102), ('teapot-big_white_floral', 255)], 'instance_ids': [51, 102, 255], 'class_ids': [2, 5, 6], 'scales': array([0.18288413, 0.1937201 , 0.37555959]), 'rotations': array([[[-0.3009299 , -0.21250548, -0.92966802],
%         [ 0.49253494, -0.86940493,  0.03929879],
%         [-0.81660917, -0.4460678 ,  0.36629631]],

%        [[-0.95551237, -0.22365636,  0.1922861 ],
%         [ 0.10425944, -0.8659523 , -0.48913862],
%         [ 0.27590955, -0.44733036,  0.85074642]],

%        [[-0.9792387 , -0.20270242, -0.00181857],
%         [ 0.1838896 , -0.88450892, -0.42875235],
%         [ 0.0853006 , -0.42018531,  0.90342023]]]), 'translations': array([[-0.11205502, -0.00193513,  0.69656178],
%        [ 0.11710977, -0.03201663,  0.78072799],
%        [ 0.05743918, -0.00991829,  0.55208297]]), 'bboxes': array([[368, 418, 517, 505],
%        [392, 714, 428, 762],
%        [298, 466, 591, 808]], dtype=int64), 'gt_scales': array([[0.075266, 0.148535, 0.075624],
%        [0.185642, 0.023059, 0.050327],
%        [0.255478, 0.220202, 0.165188]])}

The \texttt{"pose\_video.avi"} file contains the visualization of the pose annotation as 3D bounding boxes and rendered object masks on the RGB video for a qualitative evaluation of the pose annotation accuracy as well as camera trajectory coverage (Fig.~\ref{fig:mesh_canonical}).

\begin{figure*}[!t]
 \centering
    \includegraphics[width=\linewidth]{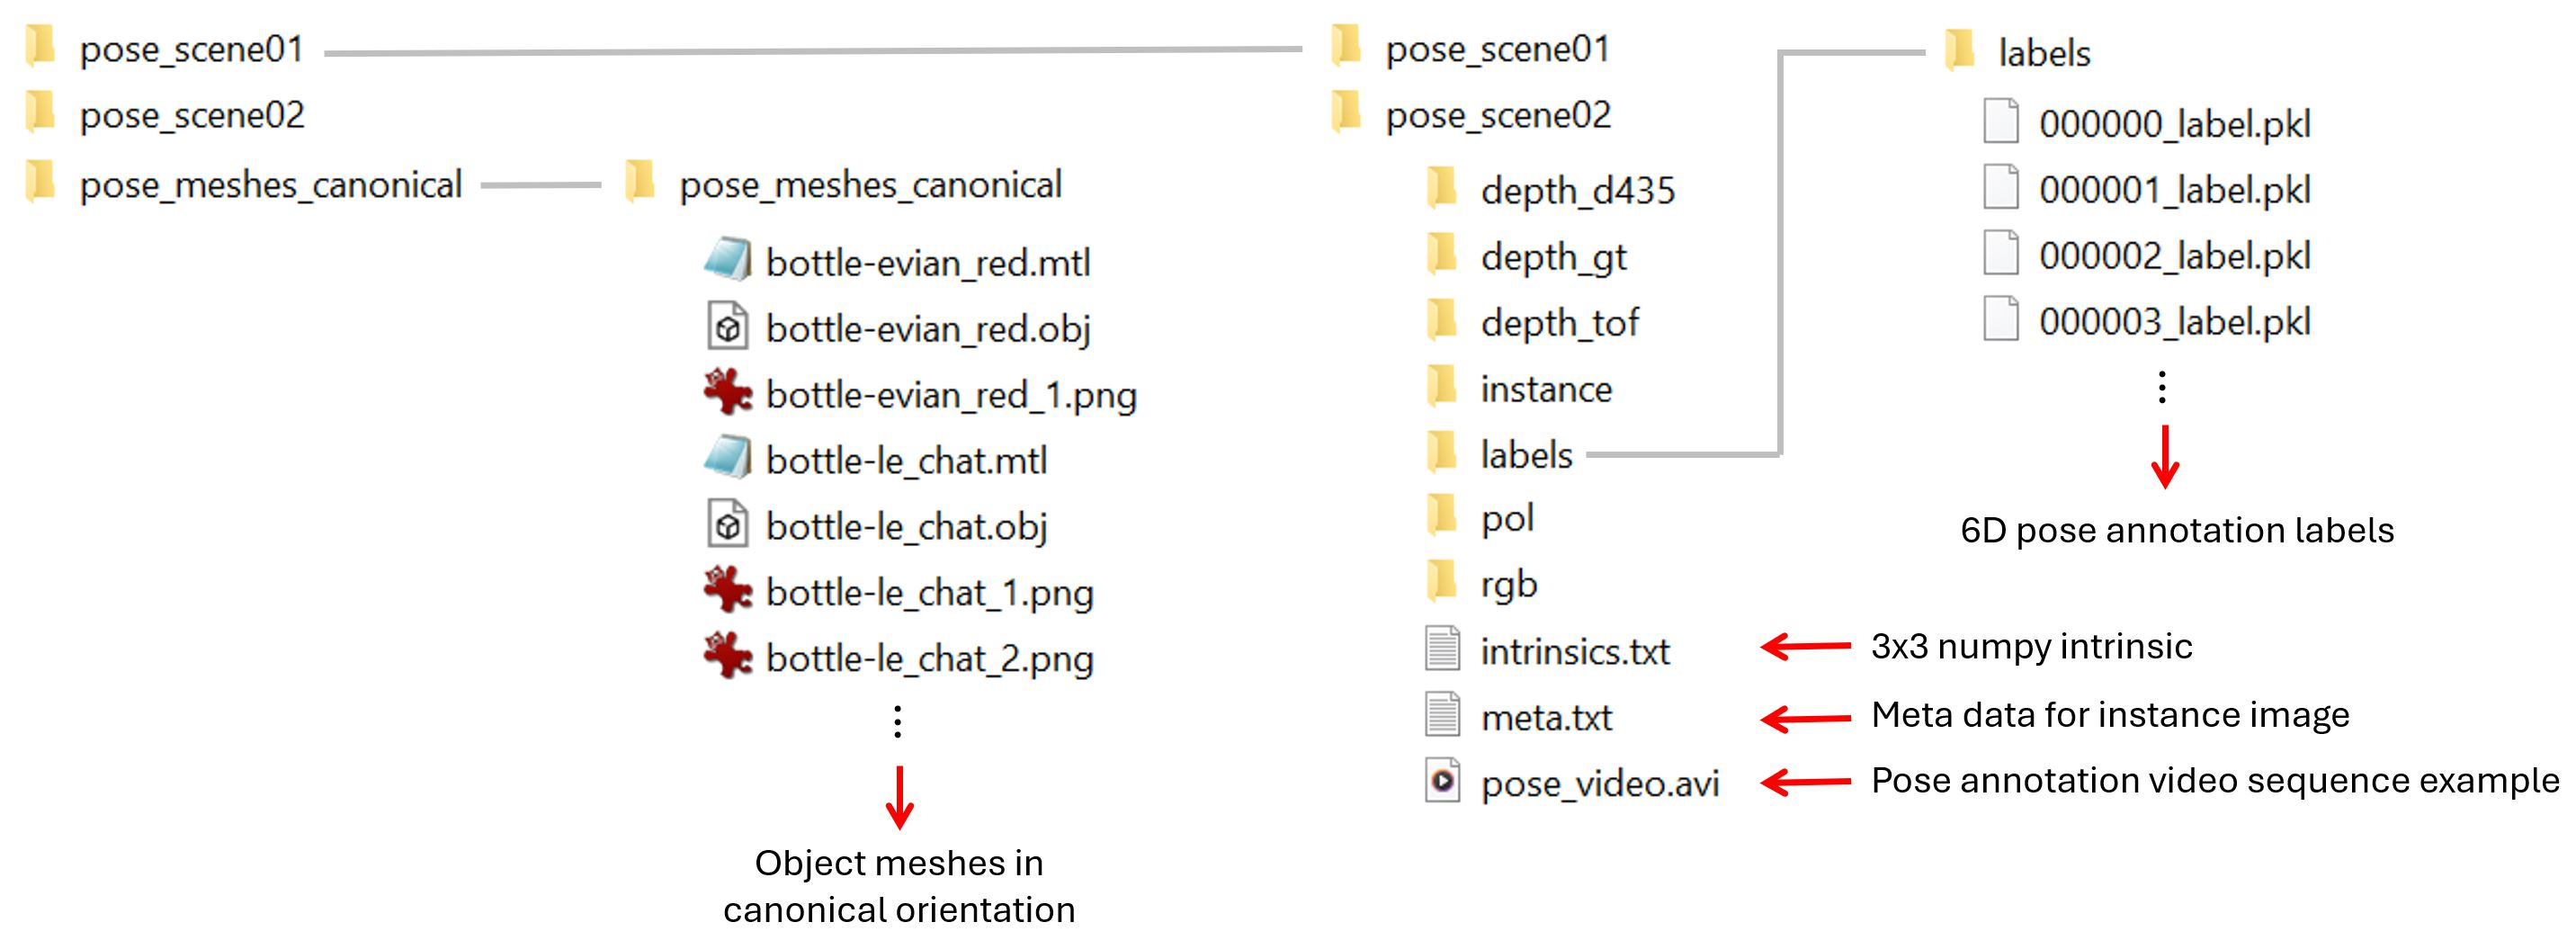}
    \caption{\textbf{File Structure of the 6D Pose Estimation Dataset.}}
    \label{fig:pose_scene_layout}
\end{figure*}

\begin{figure*}[!t]
 \centering
    \includegraphics[width=\linewidth]{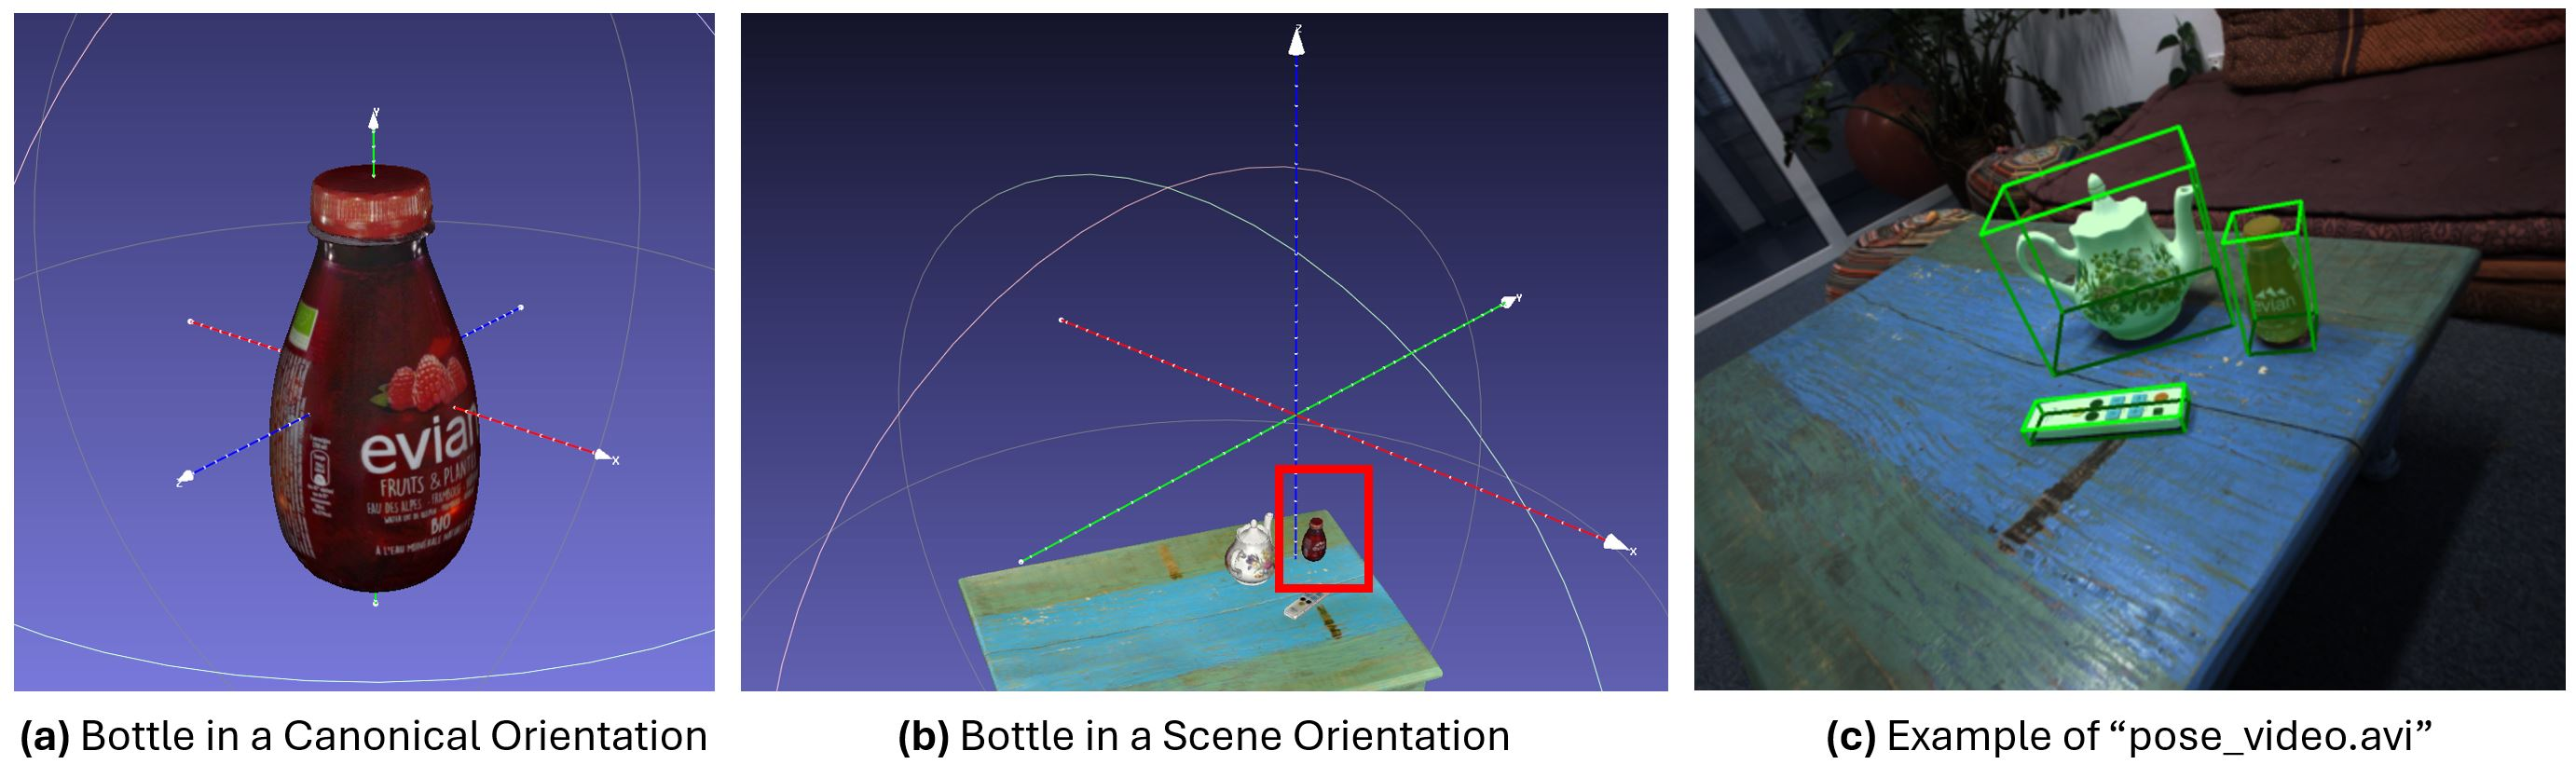}
    \caption{\textbf{Example of Meshes and \texttt{"pose\_video.avi"}.} The object in the canonical orientation is self centered and oriented according to a specific convention (i.e. standing with y-axis), while the object in the scene orientation is oriented according to the scene's layout. The meshes are visualized in Meshlab~\cite{meshlab}.}
    \label{fig:mesh_canonical}
\end{figure*}

\clearpage
