# Supplementary material for: SCRREAM : SCan, Register, REnder And Map:A Framework for Annotating Accurate and Dense 3D Indoor Scenes with a Benchmark
Source: arXiv:2410.22715 source file (2025-01-06)
Supplement: Supplementary file 5 [file suppl_6_license.tex]

\section{Licenses of Codes Used in Benchmarks} \label{sec:suppl_license}

% \begin{table}[]
% \centering
% \resizebox{0.5\textwidth}{!}{
% \setlength{\tabcolsep}{10pt}
% \begin{tabular}{c|ccccccc}
% \hline
% Methods &
% \rotatebox[origin=c]{90}{\small NICE-SLAM} &
% \rotatebox[origin=c]{90}{\small CO-SLAM}   & 
% \rotatebox[origin=c]{90}{\small Gaussian-SLAM} & 
% \rotatebox[origin=c]{90}{\small NeRF(Depth)-Facto} & 
% \rotatebox[origin=c]{90}{\small Zip-NeRF} &
% \rotatebox[origin=c]{90}{\small Gaussian-Spatting}  & 
% \rotatebox[origin=c]{90}{\small Mip-Splatting}    \\ \hline

% License &

% \rotatebox[origin=c]{90}{\small Apache-2.0} &
% \rotatebox[origin=c]{90}{\small Apache-2.0} &
% \rotatebox[origin=c]{90}{\small MIT}        & 
% \rotatebox[origin=c]{90}{\small Apache-2.0} &
% \rotatebox[origin=c]{90}{\small Apache-2.0} & 
% \rotatebox[origin=c]{90}{\small Own by Inria, MPII} & 
% \rotatebox[origin=c]{90}{\small Own by Inria, MPII} \\ \hline
% \end{tabular}

% }
% \end{table}

In this section, we show licenses of codes that are used in the benchmark for NVS (Tab.~\ref{tab:license_nvs}) and SLAM (Tab.~\ref{tab:license_slam}). Note that our dataset uses the \textbf{MIT License}.

\begin{table}[!h]
\centering
\caption{\textbf{License Information of the NVS code Used in the Benchmark.}}
\resizebox{0.98\textwidth}{!}{
\setlength{\tabcolsep}{6pt}
\begin{tabular}{c|cccc}
\hline
Methods &  NeRF(Depth)-Facto~\cite{tancik2023nerfstudio} & Zip-NeRF~\cite{barron2023zipnerf} & Gaussian-Spatting~\cite{kerbl3Dgaussians}  & Mip-Splatting~\cite{Yu2023MipSplatting}  \\ \hline
License &  Apache-2.0        & Apache-2.0 & Inria and MPII & Inria and MPII \\ \hline
\end{tabular}
\label{tab:license_nvs}
}
\end{table}

\begin{table}[!h]
\centering
\caption{\textbf{License Information of the SLAM code Used in the Benchmark.}}
\resizebox{0.75\textwidth}{!}{
\setlength{\tabcolsep}{7pt}

\begin{tabular}{c|ccc}
\hline
Methods & NICE-SLAM~\cite{Zhu2022niceslam}  & CO-SLAM~\cite{wang2023coslam}    & Gaussian-SLAM~\cite{yugay2023gaussianslam}  \\ \hline
License & Apache-2.0 & Apache-2.0 & MIT            \\ \hline
\end{tabular}
\label{tab:license_slam}
}
\end{table}
