# Supplementary material for: SCRREAM : SCan, Register, REnder And Map:A Framework for Annotating Accurate and Dense 3D Indoor Scenes with a Benchmark
Source: arXiv:2410.22715 source file (2025-01-06)
Supplement: Supplementary file 6 [file suppl_5_baseline.tex]

\section{Full Benchmarks} \label{sec:suppl_benchmark}

In this section, we show the benchmark results of NVS and SLAM for each scene separately.

\subsection{Novel View Synthesis}

In this study, the poor performance of NeRFacto~\cite{tancik2023nerfstudio} in both RGB and depth quality demonstrates the limitations in the model's ability to learn fine details and accurate geometry. In contrast, Gaussian-Splatting~\cite{kerbl3Dgaussians}, Mip-Splatting~\cite{Yu2023MipSplatting}, and Zip-NeRF~\cite{barron2023zipnerf} demonstrate superior performance in RGB image reconstruction. These methods prioritize visual fidelity, resulting in high-quality image outputs. However, the lack of geometric constraints in these models means that while they excel in producing visually appealing images, they fall short in accurately capturing and reconstructing depth information. Focusing on depth estimation, Depth-Facto~\cite{tancik2023nerfstudio} (AS) and Depth-Facto~\cite{tancik2023nerfstudio} (ToF) stand out for their exemplary performance in depth estimation metrics. These methods leverage the integration of multi-modal sensor data, which acts as an additional constraint, enhancing their ability to accurately predict depth. The utilization of both AS and ToF sensor data demonstrates the significant advantage of incorporating diverse and complementary data sources, leading to improved depth estimation performance.

\begin{table}[h]
\centering
\caption{\textbf{NVS Benchmark for scene01}}
\resizebox{0.95\textwidth}{!}{
\setlength{\tabcolsep}{5pt}
\begin{tabular}{l|ccc|cccccc}
\hline
Evaluation         & \multicolumn{3}{c|}{RGB} & \multicolumn{6}{c}{Depth}                     \T\B\\ \hline
Method             & PSNR\(\uparrow\)   & SSIM\(\uparrow\) & LPIPS\(\downarrow\)  & RSME\(\downarrow\) & Abs Rel\(\downarrow\) & Sqr Rel\(\downarrow\) & <1.25\(^{1}\uparrow\) & <1.25\(^{2}\uparrow\) & <1.25\(^{3}\uparrow\) \T\B\\ \hline
NeRFacto~\cite{tancik2023nerfstudio}          & 22.346 &  0.801 & 0.258 &  0.814 & 0.414 &   0.529 & 0.564 & 0.728 & 0.807 \T\B\\
Depth-Facto~\cite{tancik2023nerfstudio} (AS)& 25.313 &  0.828 & 0.244 &  0.224 & 0.086 &   0.068 & 0.939 & 0.956 & 0.964 \T\B\\
Depth-Facto~\cite{tancik2023nerfstudio}  (ToF)& 25.267 &  0.827 & 0.242 &  0.300 & 0.090 &   0.099 & 0.908 & 0.928 & 0.941 \T\B\\
Zip-NeRF~\cite{barron2023zipnerf}             & 29.548 &  0.832 & 0.142 &  0.322 & 0.177 &   0.075 & 0.647 & 0.955 & 0.972 \T\B\\ \hline
Gaussian-Splatting~\cite{kerbl3Dgaussians}    & 28.282 &  0.848 & 0.279 &  0.322 & 0.133 &   0.068 & 0.777 & 0.904 & 0.952 \T\B\\
Mip-Splatting~\cite{Yu2023MipSplatting}       & 28.384 &  0.848 & 0.278 &  0.309 & 0.122 &   0.061 & 0.803 & 0.925 & 0.956 \T\B\\ \hline
\end{tabular}
}
\label{tab:nvs_benchmark1}
\end{table}

\begin{table}[h]
\centering
\caption{\textbf{NVS Benchmark for scene02}}
\resizebox{0.95\textwidth}{!}{
\setlength{\tabcolsep}{5pt}
\begin{tabular}{l|ccc|cccccc}
\hline
Evaluation         & \multicolumn{3}{c|}{RGB} & \multicolumn{6}{c}{Depth}                     \T\B\\ \hline
Method             & PSNR\(\uparrow\)   & SSIM\(\uparrow\) & LPIPS\(\downarrow\)  & RSME\(\downarrow\) & Abs Rel\(\downarrow\) & Sqr Rel\(\downarrow\) & <1.25\(^{1}\uparrow\) & <1.25\(^{2}\uparrow\) & <1.25\(^{3}\uparrow\) \T\B\\ \hline
NeRFacto~\cite{tancik2023nerfstudio}          & 24.011 &  0.808 & 0.300 &  1.243 & 0.528 &   0.951 & 0.493 & 0.635 & 0.763 \T\B\\
Depth-Facto~\cite{tancik2023nerfstudio} (AS)& 26.062 &  0.835 & 0.283 &  0.228 & 0.092 &   0.027 & 0.981 & 0.995 & 0.999 \T\B\\
Depth-Facto~\cite{tancik2023nerfstudio}  (ToF)& 26.251 &  0.838 & 0.275 &  0.739 & 0.192 &   0.372 & 0.855 & 0.870 & 0.898 \T\B\\
Zip-NeRF~\cite{barron2023zipnerf}             & 32.278 &  0.812 & 0.190 &  0.374 & 0.173 &   0.074 & 0.640 & 0.941 & 0.994 \T\B\\ \hline
Gaussian-Splatting~\cite{kerbl3Dgaussians}    & 29.616 &  0.842 & 0.322 &  0.483 & 0.195 &   0.144 & 0.683 & 0.852 & 0.899 \T\B\\
Mip-Splatting~\cite{Yu2023MipSplatting}       & 29.230 &  0.842 & 0.323 &  0.531 & 0.218 &   0.164 & 0.610 & 0.824 & 0.884 \T\B\\ \hline
\end{tabular}
}
\label{tab:nvs_benchmark2}
\end{table}

\begin{table}[!h]
\centering
\caption{\textbf{NVS Benchmark for scene03}}
\resizebox{0.95\textwidth}{!}{
\setlength{\tabcolsep}{5pt}
\begin{tabular}{l|ccc|cccccc}
\hline
Evaluation         & \multicolumn{3}{c|}{RGB} & \multicolumn{6}{c}{Depth}                     \T\B\\ \hline
Method             & PSNR\(\uparrow\)   & SSIM\(\uparrow\) & LPIPS\(\downarrow\)  & RSME\(\downarrow\) & Abs Rel\(\downarrow\) & Sqr Rel\(\downarrow\) & <1.25\(^{1}\uparrow\) & <1.25\(^{2}\uparrow\) & <1.25\(^{3}\uparrow\) \T\B\\ \hline
NeRFacto~\cite{tancik2023nerfstudio}          & 20.823 & 0.808 & 0.277 & 2.093 & 1.482 & 3.664 & 0.129 & 0.224 & 0.312 \T\B\\
Depth-Facto~\cite{tancik2023nerfstudio} (AS)& 24.227 & 0.869 & 0.207 & 0.500 & 0.199 & 0.341 & 0.915 & 0.939 & 0.956 \T\B\\
Depth-Facto~\cite{tancik2023nerfstudio}  (ToF)& 24.524 & 0.875 & 0.236 & 0.960 & 0.366 & 0.816 & 0.777 & 0.805 & 0.827 \T\B\\
Zip-NeRF~\cite{barron2023zipnerf}             & 33.581 & 0.905 & 0.117 & 0.368 & 0.187 & 0.086 & 0.616 & 0.910 & 0.969 \T\B\\ \hline
Gaussian-Splatting~\cite{kerbl3Dgaussians}    & 28.928 & 0.920 & 0.274 & 0.531 & 0.253 & 0.173 & 0.452 & 0.788 & 0.902 \T\B\\
Mip-Splatting~\cite{Yu2023MipSplatting}       & 29.304 & 0.920 & 0.273 & 0.527 & 0.257 & 0.170 & 0.444 & 0.760 & 0.903 \T\B\\ \hline
\end{tabular}
}
\label{tab:nvs_benchmark03}
\end{table}

\clearpage

\begin{table}[!h]
\centering
\caption{\textbf{NVS Benchmark for scene04, sequence00}}
\resizebox{0.95\textwidth}{!}{
\setlength{\tabcolsep}{5pt}
\begin{tabular}{l|ccc|cccccc}
\hline
Evaluation         & \multicolumn{3}{c|}{RGB} & \multicolumn{6}{c}{Depth}                     \T\B\\ \hline
Method             & PSNR\(\uparrow\)   & SSIM\(\uparrow\) & LPIPS\(\downarrow\)  & RSME\(\downarrow\) & Abs Rel\(\downarrow\) & Sqr Rel\(\downarrow\) & <1.25\(^{1}\uparrow\) & <1.25\(^{2}\uparrow\) & <1.25\(^{3}\uparrow\) \T\B\\ \hline
NeRFacto~\cite{tancik2023nerfstudio}          & 21.880 &  0.775 & 0.284 &  1.102 & 0.485 &   0.740 & 0.431 & 0.655 & 0.815 \T\B\\
Depth-Facto~\cite{tancik2023nerfstudio} (AS)& 22.803 &  0.791 & 0.247 &  0.262 & 0.088 &   0.036 & 0.950 & 0.979 & 0.993 \T\B\\
Depth-Facto~\cite{tancik2023nerfstudio}  (ToF)& 23.060 &  0.800 & 0.246 &  0.306 & 0.062 &   0.055 & 0.932 & 0.958 & 0.977 \T\B\\
Zip-NeRF~\cite{barron2023zipnerf}             & 24.267 &  0.783 & 0.232 &  0.602 & 0.244 &   0.208 & 0.510 & 0.825 & 0.914 \T\B\\ \hline
Gaussian-Splatting~\cite{kerbl3Dgaussians}    & 20.037 &  0.758 & 0.379 &  1.002 & 0.393 &   0.494 & 0.321 & 0.519 & 0.653 \T\B\\
Mip-Splatting~\cite{Yu2023MipSplatting}       & 20.605 &  0.766 & 0.370 &  1.032 & 0.412 &   0.508 & 0.271 & 0.485 & 0.615 \T\B\\ \hline
\end{tabular}
}
\label{tab:nvs_benchmark4-0}
\end{table}

\begin{table}[!h]
\centering
\caption{\textbf{NVS Benchmark for scene04, sequence01}}
\resizebox{0.95\textwidth}{!}{
\setlength{\tabcolsep}{5pt}
\begin{tabular}{l|ccc|cccccc}
\hline
Evaluation         & \multicolumn{3}{c|}{RGB} & \multicolumn{6}{c}{Depth}                     \T\B\\ \hline
Method             & PSNR\(\uparrow\)   & SSIM\(\uparrow\) & LPIPS\(\downarrow\)  & RSME\(\downarrow\) & Abs Rel\(\downarrow\) & Sqr Rel\(\downarrow\) & <1.25\(^{1}\uparrow\) & <1.25\(^{2}\uparrow\) & <1.25\(^{3}\uparrow\) \T\B\\ \hline
NeRFacto~\cite{tancik2023nerfstudio}          & 23.323 & 0.771 & 0.324 & 1.216 & 0.723 & 1.089 & 0.269 & 0.428 & 0.662 \T\B\\
Depth-Facto~\cite{tancik2023nerfstudio} (AS)& 25.453 & 0.803 & 0.292 & 0.268 & 0.084 & 0.062 & 0.951 & 0.962 & 0.982 \T\B\\
Depth-Facto~\cite{tancik2023nerfstudio}  (ToF)& 25.370 & 0.804 & 0.288 & 0.284 & 0.067 & 0.069 & 0.933 & 0.949 & 0.967 \T\B\\
Zip-NeRF~\cite{barron2023zipnerf}             & 25.046 & 0.765 & 0.344 & 0.781 & 0.441 & 0.498 & 0.352 & 0.546 & 0.610 \T\B\\ \hline
Gaussian-Splatting~\cite{kerbl3Dgaussians}    & 23.207 & 0.784 & 0.374 & 0.691 & 0.340 & 0.303 & 0.374 & 0.589 & 0.714 \T\B\\
Mip-Splatting~\cite{Yu2023MipSplatting}       & 23.008 & 0.782 & 0.378 & 0.711 & 0.359 & 0.327 & 0.356 & 0.559 & 0.676  \T\B\\ \hline
\end{tabular}
}
\label{tab:nvs_benchmark4-1}
\end{table}

\begin{table}[!h]
\centering
\caption{\textbf{NVS Benchmark for scene05}}
\resizebox{0.95\textwidth}{!}{
\setlength{\tabcolsep}{5pt}
\begin{tabular}{l|ccc|cccccc}
\hline
Evaluation         & \multicolumn{3}{c|}{RGB} & \multicolumn{6}{c}{Depth}                     \T\B\\ \hline
Method             & PSNR\(\uparrow\)   & SSIM\(\uparrow\) & LPIPS\(\downarrow\)  & RSME\(\downarrow\) & Abs Rel\(\downarrow\) & Sqr Rel\(\downarrow\) & <1.25\(^{1}\uparrow\) & <1.25\(^{2}\uparrow\) & <1.25\(^{3}\uparrow\) \T\B\\ \hline
NeRFacto~\cite{tancik2023nerfstudio}          & 20.897 & 0.755 & 0.371 & 1.175 & 0.672 & 1.025 & 0.340 & 0.500 & 0.688 \T\B\\
Depth-Facto~\cite{tancik2023nerfstudio} (AS)& 23.172 & 0.786 & 0.360 & 0.141 & 0.059 & 0.016 & 0.975 & 0.984 & 0.993 \T\B\\
Depth-Facto~\cite{tancik2023nerfstudio}  (ToF)& 23.038 & 0.785 & 0.357 & 0.202 & 0.058 & 0.057 & 0.941 & 0.960 & 0.971 \T\B\\
Zip-NeRF~\cite{barron2023zipnerf}             & 24.206 & 0.770 & 0.364 & 0.633 & 0.348 & 0.325 & 0.410 & 0.654 & 0.735 \T\B\\ \hline
Gaussian-Splatting~\cite{kerbl3Dgaussians}    & 25.627 & 0.817 & 0.345 & 0.482 & 0.224 & 0.160 & 0.590 & 0.791 & 0.879 \T\B\\
Mip-Splatting~\cite{Yu2023MipSplatting}       & 25.177 & 0.814 & 0.345 & 0.472 & 0.222 & 0.158 & 0.604 & 0.801 & 0.880 \T\B\\ \hline
\end{tabular}
}
\label{tab:nvs_benchmark5}
\end{table}

\begin{table}[!h]
\centering
\caption{\textbf{NVS Benchmark for scene06}}
\resizebox{0.95\textwidth}{!}{
\setlength{\tabcolsep}{5pt}
\begin{tabular}{l|ccc|cccccc}
\hline
Evaluation         & \multicolumn{3}{c|}{RGB} & \multicolumn{6}{c}{Depth}                     \T\B\\ \hline
Method             & PSNR\(\uparrow\)   & SSIM\(\uparrow\) & LPIPS\(\downarrow\)  & RSME\(\downarrow\) & Abs Rel\(\downarrow\) & Sqr Rel\(\downarrow\) & <1.25\(^{1}\uparrow\) & <1.25\(^{2}\uparrow\) & <1.25\(^{3}\uparrow\) \T\B\\ \hline
NeRFacto~\cite{tancik2023nerfstudio}          & 23.050 & 0.809 & 0.262 & 0.921 & 0.420 & 0.663 & 0.599 & 0.789 & 0.864 \T\B\\
Depth-Facto~\cite{tancik2023nerfstudio} (AS)& 24.118 & 0.813 & 0.269 & 0.126 & 0.035 & 0.008 & 0.988 & 0.997 & 0.999 \T\B\\
Depth-Facto~\cite{tancik2023nerfstudio}  (ToF)& 24.106 & 0.812 & 0.267 & 0.098 & 0.019 & 0.008 & 0.988 & 0.994 & 0.997 \T\B\\
Zip-NeRF~\cite{barron2023zipnerf}             & 26.724 & 0.818 & 0.224 & 0.403 & 0.203 & 0.116 & 0.623 & 0.890 & 0.937 \T\B\\ \hline
Gaussian-Splatting~\cite{kerbl3Dgaussians}    & 26.992 & 0.833 & 0.269 & 0.386 & 0.141 & 0.081 & 0.793 & 0.948 & 0.979 \T\B\\
Mip-Splatting~\cite{Yu2023MipSplatting}       & 26.992 & 0.833 & 0.269 & 0.386 & 0.141 & 0.081 & 0.793 & 0.948 & 0.979 \T\B\\ \hline
\end{tabular}
}
\label{tab:nvs_benchmark6}
\end{table}

\begin{table}[!h]
\centering
\caption{\textbf{NVS Benchmark for scene07}}
\resizebox{0.95\textwidth}{!}{
\setlength{\tabcolsep}{5pt}
\begin{tabular}{l|ccc|cccccc}
\hline
Evaluation         & \multicolumn{3}{c|}{RGB} & \multicolumn{6}{c}{Depth}                     \T\B\\ \hline
Method             & PSNR\(\uparrow\)   & SSIM\(\uparrow\) & LPIPS\(\downarrow\)  & RSME\(\downarrow\) & Abs Rel\(\downarrow\) & Sqr Rel\(\downarrow\) & <1.25\(^{1}\uparrow\) & <1.25\(^{2}\uparrow\) & <1.25\(^{3}\uparrow\) \T\B\\ \hline
NeRFacto~\cite{tancik2023nerfstudio}          & 22.820 & 0.672 & 0.528 & 0.954 & 0.401 & 0.584 & 0.567 & 0.745 & 0.855 \T\B\\
Depth-Facto~\cite{tancik2023nerfstudio} (AS)& 23.560 & 0.677 & 0.514 & 0.149 & 0.055 & 0.014 & 0.991 & 0.995 & 0.997 \T\B\\
Depth-Facto~\cite{tancik2023nerfstudio}  (ToF)& 23.530 & 0.679 & 0.517 & 0.166 & 0.028 & 0.025 & 0.979 & 0.987 & 0.992 \T\B\\
Zip-NeRF~\cite{barron2023zipnerf}             & 23.559 & 0.646 & 0.459 & 0.737 & 0.376 & 0.379 & 0.273 & 0.626 & 0.748 \T\B\\ \hline
Gaussian-Splatting~\cite{kerbl3Dgaussians}    & 24.457 & 0.693 & 0.417 & 0.521 & 0.210 & 0.148 & 0.588 & 0.834 & 0.916 \T\B\\
Mip-Splatting~\cite{Yu2023MipSplatting}       & 24.258 & 0.693 & 0.416 & 0.530 & 0.212 & 0.153 & 0.592 & 0.829 & 0.912 \T\B\\ \hline
\end{tabular}
}
\label{tab:nvs_benchmark7}
\end{table}

\clearpage

\begin{table}[!h]
\centering
\caption{\textbf{NVS Benchmark for scene08}}
\resizebox{0.95\textwidth}{!}{
\setlength{\tabcolsep}{5pt}
\begin{tabular}{l|ccc|cccccc}
\hline
Evaluation         & \multicolumn{3}{c|}{RGB} & \multicolumn{6}{c}{Depth}                     \T\B\\ \hline
Method             & PSNR\(\uparrow\)   & SSIM\(\uparrow\) & LPIPS\(\downarrow\)  & RSME\(\downarrow\) & Abs Rel\(\downarrow\) & Sqr Rel\(\downarrow\) & <1.25\(^{1}\uparrow\) & <1.25\(^{2}\uparrow\) & <1.25\(^{3}\uparrow\) \T\B\\ \hline
NeRFacto~\cite{tancik2023nerfstudio}          & 23.803 & 0.619 & 0.535 & 0.908 & 0.430 & 0.567 & 0.505 & 0.710 & 0.855 \T\B\\
Depth-Facto~\cite{tancik2023nerfstudio} (AS)& 24.849 & 0.629 & 0.517 & 0.121 & 0.048 & 0.009 & 0.988 & 0.995 & 0.999 \T\B\\
Depth-Facto~\cite{tancik2023nerfstudio}  (ToF)& 24.913 & 0.632 & 0.513 & 0.097 & 0.023 & 0.008 & 0.983 & 0.992 & 0.998 \T\B\\
Zip-NeRF~\cite{barron2023zipnerf}             & 26.584 & 0.629 & 0.367 & 0.304 & 0.153 & 0.060 & 0.735 & 0.971 & 0.983 \T\B\\ \hline
Gaussian-Splatting~\cite{kerbl3Dgaussians}    & 25.140 & 0.639 & 0.416 & 0.389 & 0.153 & 0.084 & 0.720 & 0.908 & 0.961 \T\B\\
Mip-Splatting~\cite{Yu2023MipSplatting}       & 25.214 & 0.640 & 0.415 & 0.385 & 0.149 & 0.082 & 0.732 & 0.907 & 0.960 \T\B\\ \hline
\end{tabular}
}
\label{tab:nvs_benchmark8}
\end{table}

\begin{table}[!h]
\centering
\caption{\textbf{NVS Benchmark for scene09}}
\resizebox{0.95\textwidth}{!}{
\setlength{\tabcolsep}{5pt}
\begin{tabular}{l|ccc|cccccc}
\hline
Evaluation         & \multicolumn{3}{c|}{RGB} & \multicolumn{6}{c}{Depth}                     \T\B\\ \hline
Method             & PSNR\(\uparrow\)   & SSIM\(\uparrow\) & LPIPS\(\downarrow\)  & RSME\(\downarrow\) & Abs Rel\(\downarrow\) & Sqr Rel\(\downarrow\) & <1.25\(^{1}\uparrow\) & <1.25\(^{2}\uparrow\) & <1.25\(^{3}\uparrow\) \T\B\\ \hline
NeRFacto~\cite{tancik2023nerfstudio}          & 22.594 & 0.601 & 0.583 & 1.067 & 0.616 & 0.923 & 0.425 & 0.596 & 0.715 \T\B\\
Depth-Facto~\cite{tancik2023nerfstudio} (AS)& 23.273 & 0.610 & 0.571 & 0.097 & 0.037 & 0.006 & 0.990 & 0.996 & 0.999 \T\B\\
Depth-Facto~\cite{tancik2023nerfstudio}  (ToF)& 23.029 & 0.607 & 0.572 & 0.128 & 0.030 & 0.021 & 0.974 & 0.983 & 0.986 \T\B\\
Zip-NeRF~\cite{barron2023zipnerf}             & 23.734 & 0.603 & 0.433 & 0.484 & 0.270 & 0.175 & 0.406 & 0.766 & 0.884 \T\B\\ \hline
Gaussian-Splatting~\cite{kerbl3Dgaussians}    & 24.038 & 0.626 & 0.427 & 0.364 & 0.160 & 0.084 & 0.709 & 0.898 & 0.958 \T\B\\
Mip-Splatting~\cite{Yu2023MipSplatting}       & 24.091 & 0.627 & 0.428 & 0.364 & 0.160 & 0.086 & 0.704 & 0.891 & 0.954\T\B\\ \hline
\end{tabular}
}
\label{tab:nvs_benchmark9}
\end{table}

\begin{table}[!h]
\centering
\caption{\textbf{NVS Benchmark for scene10}}
\resizebox{0.95\textwidth}{!}{
\setlength{\tabcolsep}{5pt}
\begin{tabular}{l|ccc|cccccc}
\hline
Evaluation         & \multicolumn{3}{c|}{RGB} & \multicolumn{6}{c}{Depth}                     \T\B\\ \hline
Method             & PSNR\(\uparrow\)   & SSIM\(\uparrow\) & LPIPS\(\downarrow\)  & RSME\(\downarrow\) & Abs Rel\(\downarrow\) & Sqr Rel\(\downarrow\) & <1.25\(^{1}\uparrow\) & <1.25\(^{2}\uparrow\) & <1.25\(^{3}\uparrow\) \T\B\\ \hline
NeRFacto~\cite{tancik2023nerfstudio}          & 23.024 & 0.903 & 0.191 & 1.727 & 0.620 & 1.839 & 0.542 & 0.704 & 0.771 \T\B\\
Depth-Facto~\cite{tancik2023nerfstudio} (AS)& 23.685 & 0.908 & 0.203 & 0.190 & 0.067 & 0.017 & 0.991 & 0.999 & 1.000 \T\B\\
Depth-Facto~\cite{tancik2023nerfstudio}  (ToF)& 23.705 & 0.909 & 0.194 & 0.163 & 0.030 & 0.016 & 0.980 & 0.993 & 0.998\T\B\\
Zip-NeRF~\cite{barron2023zipnerf}             & 36.385 & 0.942 & 0.119 & 0.343 & 0.137 & 0.052 & 0.769 & 0.993 & 1.000 \T\B\\ \hline
Gaussian-Splatting~\cite{kerbl3Dgaussians}    & 26.637 & 0.928 & 0.231 & 0.450 & 0.143 & 0.099 & 0.770 & 0.923 & 0.963 \T\B\\
Mip-Splatting~\cite{Yu2023MipSplatting}       & 26.648 & 0.929 & 0.229 & 0.431 & 0.138 & 0.091 & 0.774 & 0.928 & 0.968\T\B\\ \hline
\end{tabular}
}
\label{tab:nvs_benchmark10}
\end{table}

\begin{table}[!h]
\centering
\caption{\textbf{NVS Benchmark for scene11}}
\resizebox{0.95\textwidth}{!}{
\setlength{\tabcolsep}{5pt}
\begin{tabular}{l|ccc|cccccc}
\hline
Evaluation         & \multicolumn{3}{c|}{RGB} & \multicolumn{6}{c}{Depth}                     \T\B\\ \hline
Method             & PSNR\(\uparrow\)   & SSIM\(\uparrow\) & LPIPS\(\downarrow\)  & RSME\(\downarrow\) & Abs Rel\(\downarrow\) & Sqr Rel\(\downarrow\) & <1.25\(^{1}\uparrow\) & <1.25\(^{2}\uparrow\) & <1.25\(^{3}\uparrow\) \T\B\\ \hline
NeRFacto~\cite{tancik2023nerfstudio}          & 23.166 & 0.829 & 0.212 & 1.716 & 0.950 & 2.207 & 0.287 & 0.450 & 0.601 \T\B\\
Depth-Facto~\cite{tancik2023nerfstudio} (AS)& 27.510 & 0.889 & 0.178 & 0.330 & 0.122 & 0.102 & 0.958 & 0.977 & 0.983 \T\B\\
Depth-Facto~\cite{tancik2023nerfstudio}  (ToF)& 27.695 & 0.886 & 0.174 & 0.589 & 0.151 & 0.246 & 0.858 & 0.894 & 0.928 \T\B\\
Zip-NeRF~\cite{barron2023zipnerf}             & 33.866 & 0.894 & 0.121 & 0.563 & 0.242 & 0.217 & 0.574 & 0.821 & 0.895 \T\B\\ \hline
Gaussian-Splatting~\cite{kerbl3Dgaussians}    & 28.360 & 0.928 & 0.199 & 0.691 & 0.273 & 0.249 & 0.474 & 0.715 & 0.828 \T\B\\
Mip-Splatting~\cite{Yu2023MipSplatting}       & 28.299 & 0.929 & 0.200 & 0.715 & 0.289 & 0.266 & 0.439 & 0.669 & 0.804\T\B\\ \hline
\end{tabular}
}
\label{tab:nvs_benchmark11}
\end{table}

\clearpage

\subsection{SLAM}
This benchmark compares several SLAM methods: NICE-SLAM~\cite{Zhu2022niceslam}, CO-SLAM~\cite{wang2023coslam}, and Gaussian-SLAM~\cite{yugay2023gaussianslam}, evaluated using Ground Truth (GT) data, AS (Active Stereo) sensor data, and TOF (Time of Flight) sensor data, highlighting the significant impact of sensor quality on SLAM performance.

NICE-SLAM achieves high-quality scene reconstruction by optimizing a hierarchical representation using pre-trained geometric priors~\cite{peng2020convolutional}. However, it struggles with hole-filling. CO-SLAM further improves map completion by integrating smoothness and coherence priors into coordinate encodings~\cite{Müller_Mcwilliams_Rousselle_Gross_Novák_2019}. On the other hand, Gaussian-SLAM efficiently seeds new Gaussians for newly explored areas and optimizes them online by organizing the scene into independently optimized sub-maps.

When using ground truth data, Gaussian-SLAM excels in both tracking and mapping performance, indicating a strong algorithm highly dependent on input quality. With the AS sensor, all SLAM methods exhibit some performance degradation due to the constant random noise in the depth sensor. Gaussian-SLAM shows substantial deterioration in both tracking and reconstruction performance, especially in scenes with motion blur, resulting in a higher ATE and reduced map completeness. However, CO-SLAM and NICE-SLAM demonstrate better resilience to the noisy depth input from the AS sensor, maintaining relatively higher map accuracy and completeness.

The TOF sensor data further challenges the SLAM methods since the depth quality is influenced by rapid motion. Gaussian-SLAM struggles significantly, even failing in \texttt{scene07} due to unreliable photometric and geometric consistency. Its performance drops dramatically across all metrics. Conversely, leveraging hybrid scene representations, NICE-SLAM and CO-SLAM show better robustness towards the noisy depth input, with CO-SLAM maintaining higher map completion rates.

\begin{table}[!h]
\centering
\caption{\textbf{SLAM Benchmarks for scene01.}}
\resizebox{0.85\textwidth}{!}{
\setlength{\tabcolsep}{10pt}
\begin{tabular}{lc|c|ccc}
\hline
\multicolumn{2}{c|}{Evaluation}                                                  & Tracking & \multicolumn{3}{c}{Mapping} \T\B\\ \hline
\multicolumn{1}{l|}{Methods}                        & \multicolumn{1}{l|}{Depth} & ATE\(\downarrow\) [cm]      & Acc\(\downarrow\) [cm]   & Comp\(\downarrow\) [cm]  & Comp Ratio\(\uparrow\) [\%]  \T\B\\ \hline
\multicolumn{1}{l|}{\multirow{3}{*}{NICE-SLAM~\cite{Zhu2022niceslam}}}          & GT & 1.22 & 1.47 & 2.51 & 88.97 \T\B\\
\multicolumn{1}{l|}{}                                                           & AS  & 7.39 & 10.18 & 4.69 & 66.18 \T\B\\
\multicolumn{1}{l|}{}                                                           & ToF   & 7.39 & 17.01 & 7.03 & 65.34 \T\B\\ \hline
\multicolumn{1}{l|}{\multirow{3}{*}{CO-SLAM~\cite{wang2023coslam}}}             & GT & 3.22 & 1.48 & 1.46 & 96.06 \T\B\\
\multicolumn{1}{l|}{}                                                           & AS & 9.18 & 6.29 & 3.40 & 78.19 \T\B\\
\multicolumn{1}{l|}{}                                                           & ToF  & 7.61 & 9.54 & 4.54 & 77.12 \T\B\\ \hline
\multicolumn{1}{l|}{\multirow{3}{*}{Gaussian-SLAM~\cite{yugay2023gaussianslam}}}& GT & 0.86 & 0.65 & 0.76 & 99.64 \T\B\\
\multicolumn{1}{l|}{}                                                           & AS  & 9.18 & 21.53 & 3.73 & 74.62 \T\B\\
\multicolumn{1}{l|}{}                                                           & ToF  & 4.96 & 21.92 & 3.73 & 74.42  \T\B\\ \hline
\end{tabular}
}
\label{tab:slam_benchmark1}
\end{table}

\begin{table}[!h]
\centering
\caption{\textbf{SLAM Benchmarks for scene02.}}
\resizebox{0.85\textwidth}{!}{
\setlength{\tabcolsep}{10pt}
\begin{tabular}{lc|c|ccc}
\hline
\multicolumn{2}{c|}{Evaluation}                                                  & Tracking & \multicolumn{3}{c}{Mapping} \T\B\\ \hline
\multicolumn{1}{l|}{Methods}                        & \multicolumn{1}{l|}{Depth} & ATE\(\downarrow\) [cm]      & Acc\(\downarrow\) [cm]   & Comp\(\downarrow\) [cm]  & Comp Ratio\(\uparrow\) [\%]  \T\B\\ \hline
\multicolumn{1}{l|}{\multirow{3}{*}{NICE-SLAM~\cite{Zhu2022niceslam}}}          & GT & 7.33 & 2.93 & 4.25 & 78.41 \T\B\\
\multicolumn{1}{l|}{}                                                           & AS  & 18.14 & 15.31 & 7.91 & 43.72 \T\B\\
\multicolumn{1}{l|}{}                                                           & ToF & 5.15 & 18.20 & 6.84 & 69.02 \T\B\\ \hline
\multicolumn{1}{l|}{\multirow{3}{*}{CO-SLAM~\cite{wang2023coslam}}}             & GT & 3.50 & 1.49 & 1.54 & 97.04 \T\B\\
\multicolumn{1}{l|}{}                                                           & AS  & 13.27 & 27.33 & 13.95 & 36.21 \T\B\\
\multicolumn{1}{l|}{}                                                           & ToF  & 5.62 & 37.77 & 4.30 & 80.71 \T\B\\ \hline
\multicolumn{1}{l|}{\multirow{3}{*}{Gaussian-SLAM~\cite{yugay2023gaussianslam}}}& GT & 1.83 & 1.15 & 1.16 & 99.06 \T\B\\
\multicolumn{1}{l|}{}                                                           & AS & 17.50 & 25.75 & 10.50 & 33.48 \T\B\\
\multicolumn{1}{l|}{}                                                           & ToF & 29.81 & 43.69 & 7.01 & 56.81  \T\B\\ \hline
\end{tabular}
}
\label{tab:slam_benchmark2}
\end{table}

\begin{table}[!h]
\centering
\caption{\textbf{SLAM Benchmarks for scene03.}}
\resizebox{0.85\textwidth}{!}{
\setlength{\tabcolsep}{10pt}
\begin{tabular}{lc|c|ccc}
\hline
\multicolumn{2}{c|}{Evaluation}                                                  & Tracking & \multicolumn{3}{c}{Mapping} \T\B\\ \hline
\multicolumn{1}{l|}{Methods}                        & \multicolumn{1}{l|}{Depth} & ATE\(\downarrow\) [cm]      & Acc\(\downarrow\) [cm]   & Comp\(\downarrow\) [cm]  & Comp Ratio\(\uparrow\) [\%]  \T\B\\ \hline
\multicolumn{1}{l|}{\multirow{3}{*}{NICE-SLAM~\cite{Zhu2022niceslam}}}          & GT     & 1.64 & 2.58 & 6.11 & 84.44\T\B\\
\multicolumn{1}{l|}{}                                                           & AS & 21.79 & 60.90 & 18.71 & 34.50\T\B\\
\multicolumn{1}{l|}{}                                                           & ToF  & 8.19 & 31.26 & 12.70 & 61.87 \T\B\\ \hline
\multicolumn{1}{l|}{\multirow{3}{*}{CO-SLAM~\cite{wang2023coslam}}}             & GT    & 5.55 & 2.53 & 1.21 & 98.07 \T\B\\
\multicolumn{1}{l|}{}                                                           & AS  & 18.32 & 55.16 & 13.43 & 39.49 \T\B\\
\multicolumn{1}{l|}{}                                                           & ToF   & 18.73 & 76.67 & 6.81 & 64.79 \T\B\\ \hline
\multicolumn{1}{l|}{\multirow{3}{*}{Gaussian-SLAM~\cite{yugay2023gaussianslam}}}& GT & 5.35 & 4.64 & 1.35 & 96.98 \T\B\\
\multicolumn{1}{l|}{}                                                           & AS & 13.02 & 120.85 & 7.66 & 49.35 \T\B\\
\multicolumn{1}{l|}{}                                                           & ToF  & 13.25 & 59.84 & 4.87 & 68.95\T\B\\ \hline
\end{tabular}
}
\label{tab:slam_benchmark3}
\end{table}

\begin{table}[!h]
\centering
\caption{\textbf{SLAM Benchmarks for scene04, sequence00.}}
\resizebox{0.85\textwidth}{!}{
\setlength{\tabcolsep}{10pt}
\begin{tabular}{lc|c|ccc}
\hline
\multicolumn{2}{c|}{Evaluation}                                                  & Tracking & \multicolumn{3}{c}{Mapping} \T\B\\ \hline
\multicolumn{1}{l|}{Methods}                        & \multicolumn{1}{l|}{Depth} & ATE\(\downarrow\) [cm]      & Acc\(\downarrow\) [cm]   & Comp\(\downarrow\) [cm]  & Comp Ratio\(\uparrow\) [\%]  \T\B\\ \hline
\multicolumn{1}{l|}{\multirow{3}{*}{NICE-SLAM~\cite{Zhu2022niceslam}}}          & GT & 9.89 & 3.77 & 9.83 & 62.29\T\B\\
\multicolumn{1}{l|}{}                                                           & AS & 45.89 & 22.20 & 17.31 & 26.03 \T\B\\
\multicolumn{1}{l|}{}                                                           & ToF   & 45.70 & 20.25 & 35.38 & 23.51 \T\B\\ \hline
\multicolumn{1}{l|}{\multirow{3}{*}{CO-SLAM~\cite{wang2023coslam}}}             & GT & 4.48 & 2.01 & 1.66 & 98.27 \T\B\\
\multicolumn{1}{l|}{}                                                           & AS  & 14.97 & 30.16 & 14.08 & 28.24 \T\B\\
\multicolumn{1}{l|}{}                                                           & ToF   & 13.94 & 97.31 & 12.54 & 31.56 \T\B\\ \hline
\multicolumn{1}{l|}{\multirow{3}{*}{Gaussian-SLAM~\cite{yugay2023gaussianslam}}}& GT & 2.44 & 1.41 & 1.26 & 99.17 \T\B\\
\multicolumn{1}{l|}{}                                                           & AS & 10.43 & 22.32 & 12.12 & 30.15 \T\B\\
\multicolumn{1}{l|}{}                                                           & ToF  & 60.36 & 33.70 & 16.93 & 29.58 \T\B\\ \hline
\end{tabular}
}
\label{tab:slam_benchmark4-0}
\end{table}

\begin{table}[!h]
\centering
\caption{\textbf{SLAM Benchmarks for scene04, sequence01.}}
\resizebox{0.85\textwidth}{!}{
\setlength{\tabcolsep}{10pt}
\begin{tabular}{lc|c|ccc}
\hline
\multicolumn{2}{c|}{Evaluation}                                                  & Tracking & \multicolumn{3}{c}{Mapping} \T\B\\ \hline
\multicolumn{1}{l|}{Methods}                        & \multicolumn{1}{l|}{Depth} & ATE\(\downarrow\) [cm]      & Acc\(\downarrow\) [cm]   & Comp\(\downarrow\) [cm]  & Comp Ratio\(\uparrow\) [\%]  \T\B\\ \hline
\multicolumn{1}{l|}{\multirow{3}{*}{NICE-SLAM~\cite{Zhu2022niceslam}}}          & GT & 11.24 & 2.29 & 5.88 & 78.57\T\B\\
\multicolumn{1}{l|}{}                                                           & AS  & 14.29 & 27.84 & 12.68 & 38.01\T\B\\
\multicolumn{1}{l|}{}                                                           & ToF  & 14.13 & 20.95 & 10.18 & 48.43 \T\B\\ \hline
\multicolumn{1}{l|}{\multirow{3}{*}{CO-SLAM~\cite{wang2023coslam}}}             & GT & 8.02 & 2.21 & 2.13 & 94.37 \T\B\\
\multicolumn{1}{l|}{}                                                           & AS  & 13.74 & 67.72 & 15.30 & 26.15 \T\B\\
\multicolumn{1}{l|}{}                                                           & ToF   & 13.86 & 56.85 & 6.50 & 55.97 \T\B\\ \hline
\multicolumn{1}{l|}{\multirow{3}{*}{Gaussian-SLAM~\cite{yugay2023gaussianslam}}}& GT & 2.53 & 1.51 & 1.28 & 99.68 \T\B\\
\multicolumn{1}{l|}{}                                                           & AS & 35.27 & 24.03 & 9.92 & 37.61 \T\B\\
\multicolumn{1}{l|}{}                                                           & ToF  & 60.36 & 33.70 & 16.93 & 29.58 \T\B\\ \hline
\end{tabular}
}
\label{tab:slam_benchmark3-1}
\end{table}

\begin{table}[!h]
\centering
\caption{\textbf{SLAM Benchmarks for scene05.}}
\resizebox{0.85\textwidth}{!}{
\setlength{\tabcolsep}{10pt}
\begin{tabular}{lc|c|ccc}
\hline
\multicolumn{2}{c|}{Evaluation}                                                  & Tracking & \multicolumn{3}{c}{Mapping} \T\B\\ \hline
\multicolumn{1}{l|}{Methods}                        & \multicolumn{1}{l|}{Depth} & ATE\(\downarrow\) [cm]      & Acc\(\downarrow\) [cm]   & Comp\(\downarrow\) [cm]  & Comp Ratio\(\uparrow\) [\%]  \T\B\\ \hline
\multicolumn{1}{l|}{\multirow{3}{*}{NICE-SLAM~\cite{Zhu2022niceslam}}}          & GT & 15.24 & 9.34 & 11.66 & 50.29\T\B\\
\multicolumn{1}{l|}{}                                                           & AS  & 19.65 & 11.01 & 8.28 & 51.53\T\B\\
\multicolumn{1}{l|}{}                                                           & ToF  & 22.48 & 24.04 & 15.53 & 33.80 \T\B\\ \hline
\multicolumn{1}{l|}{\multirow{3}{*}{CO-SLAM~\cite{wang2023coslam}}}             & GT & 5.64 & 2.93 & 2.78 & 87.64 \T\B\\
\multicolumn{1}{l|}{}                                                           & AS  & 16.37 & 19.19 & 8.26 & 49.41 \T\B\\
\multicolumn{1}{l|}{}                                                           & ToF   & 25.66 & 58.58 & 12.83 & 51.28 \T\B\\ \hline
\multicolumn{1}{l|}{\multirow{3}{*}{Gaussian-SLAM~\cite{yugay2023gaussianslam}}}& GT & 17.90 & 2.92 & 2.78 & 87.63 \T\B\\
\multicolumn{1}{l|}{}                                                           & AS & 15.02 & 19.25 & 8.27 & 49.43 \T\B\\
\multicolumn{1}{l|}{}                                                           & ToF  & 18.39 & 58.71 & 12.77 & 51.30 \T\B\\ \hline
\end{tabular}
}
\label{tab:slam_benchmark5}
\end{table}

\begin{table}[!h]
\centering
\caption{\textbf{SLAM Benchmarks for scene06.}}
\resizebox{0.85\textwidth}{!}{
\setlength{\tabcolsep}{10pt}
\begin{tabular}{lc|c|ccc}
\hline
\multicolumn{2}{c|}{Evaluation}                                                  & Tracking & \multicolumn{3}{c}{Mapping} \T\B\\ \hline
\multicolumn{1}{l|}{Methods}                        & \multicolumn{1}{l|}{Depth} & ATE\(\downarrow\) [cm]      & Acc\(\downarrow\) [cm]   & Comp\(\downarrow\) [cm]  & Comp Ratio\(\uparrow\) [\%]  \T\B\\ \hline
\multicolumn{1}{l|}{\multirow{3}{*}{NICE-SLAM~\cite{Zhu2022niceslam}}}          & GT & 1.52 & 0.91 & 6.64 & 81.58\T\B\\
\multicolumn{1}{l|}{}                                                           & AS  & 76.70 & 14.34 & 9.07 & 53.28\T\B\\
\multicolumn{1}{l|}{}                                                           & ToF  & 114.70 & 27.12 & 13.33 & 40.22 \T\B\\ \hline
\multicolumn{1}{l|}{\multirow{3}{*}{CO-SLAM~\cite{wang2023coslam}}}             & GT & 3.23 & 1.10 & 1.10 & 99.16 \T\B\\
\multicolumn{1}{l|}{}                                                           & AS  & 8.05 & 12.59 & 4.21 & 71.79 \T\B\\
\multicolumn{1}{l|}{}                                                           & ToF   & 5.76 & 106.43 & 6.92 & 69.69 \T\B\\ \hline
\multicolumn{1}{l|}{\multirow{3}{*}{Gaussian-SLAM~\cite{yugay2023gaussianslam}}}& GT & 1.26	& 0.77 & 0.79 & 99.92 \T\B\\
\multicolumn{1}{l|}{}                                                           & AS & 6.24 & 19.84 & 4.44 & 66.16 \T\B\\
\multicolumn{1}{l|}{}                                                           & ToF  & 6.26 & 65.86 & 7.34 & 63.17 \T\B\\ \hline
\end{tabular}
}
\label{tab:slam_benchmark6}
\end{table}

\begin{table}[!h]
\centering
\caption{\textbf{SLAM Benchmarks for scene07.}}
\resizebox{0.85\textwidth}{!}{
\setlength{\tabcolsep}{10pt}
\begin{tabular}{lc|c|ccc}
\hline
\multicolumn{2}{c|}{Evaluation}                                                  & Tracking & \multicolumn{3}{c}{Mapping} \T\B\\ \hline
\multicolumn{1}{l|}{Methods}                        & \multicolumn{1}{l|}{Depth} & ATE\(\downarrow\) [cm]      & Acc\(\downarrow\) [cm]   & Comp\(\downarrow\) [cm]  & Comp Ratio\(\uparrow\) [\%]  \T\B\\ \hline
\multicolumn{1}{l|}{\multirow{3}{*}{NICE-SLAM~\cite{Zhu2022niceslam}}}          & GT & 5.01 & 3.26 & 7.39 & 58.74 \T\B\\
\multicolumn{1}{l|}{}                                                           & AS  & 24.81 & 19.59 & 18.14 & 28.77\T\B\\
\multicolumn{1}{l|}{}                                                           & ToF  & 5.96 & 15.60 & 8.67 & 54.41 \T\B\\ \hline
\multicolumn{1}{l|}{\multirow{3}{*}{CO-SLAM~\cite{wang2023coslam}}}             & GT & 5.22 & 1.74 & 1.76 & 97.57 \T\B\\
\multicolumn{1}{l|}{}                                                           & AS  & 14.07 & 21.75 & 14.83 & 33.20 \T\B\\
\multicolumn{1}{l|}{}                                                           & ToF   & 11.00 & 46.05 & 6.86 & 51.02 \T\B\\ \hline
\multicolumn{1}{l|}{\multirow{3}{*}{Gaussian-SLAM~\cite{yugay2023gaussianslam}}}& GT & 1.50 & 1.30 & 1.29 & 99.55 \T\B\\
\multicolumn{1}{l|}{}                                                           & AS & 151.90 & 28.53 & 14.04 & 34.61 \T\B\\
\multicolumn{1}{l|}{}                                                           & ToF  & fail & fail & fail & fail \T\B\\ \hline
\end{tabular}
}
\label{tab:slam_benchmark7}
\end{table}

\begin{table}[!h]
\centering
\caption{\textbf{SLAM Benchmarks for scene08.}}
\resizebox{0.85\textwidth}{!}{
\setlength{\tabcolsep}{10pt}
\begin{tabular}{lc|c|ccc}
\hline
\multicolumn{2}{c|}{Evaluation}                                                  & Tracking & \multicolumn{3}{c}{Mapping} \T\B\\ \hline
\multicolumn{1}{l|}{Methods}                        & \multicolumn{1}{l|}{Depth} & ATE\(\downarrow\) [cm]      & Acc\(\downarrow\) [cm]   & Comp\(\downarrow\) [cm]  & Comp Ratio\(\uparrow\) [\%]  \T\B\\ \hline
\multicolumn{1}{l|}{\multirow{3}{*}{NICE-SLAM~\cite{Zhu2022niceslam}}}          & GT & 2.39 & 2.08 & 6.56 & 81.59 \T\B\\
\multicolumn{1}{l|}{}                                                           & AS  & 80.66 & 14.95 & 12.94 & 35.21\T\B\\
\multicolumn{1}{l|}{}                                                           & ToF  & 11.41 & 11.51 & 9.99 & 57.69 \T\B\\ \hline
\multicolumn{1}{l|}{\multirow{3}{*}{CO-SLAM~\cite{wang2023coslam}}}             & GT & 3.64 & 1.61 & 1.68 & 96.88 \T\B\\
\multicolumn{1}{l|}{}                                                           & AS  & 17.86 & 23.03 & 12.87 & 34.23 \T\B\\
\multicolumn{1}{l|}{}                                                           & ToF   & 7.25 & 32.36 & 5.71 & 67.28 \T\B\\ \hline
\multicolumn{1}{l|}{\multirow{3}{*}{Gaussian-SLAM~\cite{yugay2023gaussianslam}}}& GT & 2.25 & 1.31 & 1.35 & 99.22 \T\B\\
\multicolumn{1}{l|}{}                                                           & AS & 19.46 & 21.68 & 10.73 & 36.49 \T\B\\
\multicolumn{1}{l|}{}                                                           & ToF  & 82.26 & 29.92 & 6.86 & 59.76\T\B\\ \hline
\end{tabular}
}
\label{tab:slam_benchmark8}
\end{table}

\begin{table}[!h]
\centering
\caption{\textbf{SLAM Benchmarks for scene09.}}
\resizebox{0.85\textwidth}{!}{
\setlength{\tabcolsep}{10pt}
\begin{tabular}{lc|c|ccc}
\hline
\multicolumn{2}{c|}{Evaluation}                                                  & Tracking & \multicolumn{3}{c}{Mapping} \T\B\\ \hline
\multicolumn{1}{l|}{Methods}                        & \multicolumn{1}{l|}{Depth} & ATE\(\downarrow\) [cm]      & Acc\(\downarrow\) [cm]   & Comp\(\downarrow\) [cm]  & Comp Ratio\(\uparrow\) [\%]  \T\B\\ \hline
\multicolumn{1}{l|}{\multirow{3}{*}{NICE-SLAM~\cite{Zhu2022niceslam}}}          & GT & 3.93 & 2.44 & 4.07 & 80.08\T\B\\
\multicolumn{1}{l|}{}                                                           & AS  & 30.05 & 18.92 & 14.53 & 35.47\T\B\\
\multicolumn{1}{l|}{}                                                           & ToF  & 22.15 & 24.98 & 31.79 & 20.78 \T\B\\ \hline
\multicolumn{1}{l|}{\multirow{3}{*}{CO-SLAM~\cite{wang2023coslam}}}             & GT & 2.29 & 1.66 & 1.69 & 97.64 \T\B\\
\multicolumn{1}{l|}{}                                                           & AS  & 19.39 & 17.50 & 10.74 & 45.87 \T\B\\
\multicolumn{1}{l|}{}                                                           & ToF   & 17.84 & 38.55 & 11.45 & 38.38 \T\B\\ \hline
\multicolumn{1}{l|}{\multirow{3}{*}{Gaussian-SLAM~\cite{yugay2023gaussianslam}}}& GT & 0.75 & 1.07 & 1.12 & 99.53 \T\B\\
\multicolumn{1}{l|}{}                                                           & AS & 4.28 & 14.46 & 6.61 & 53.73 \T\B\\
\multicolumn{1}{l|}{}                                                           & ToF  & 10.41 & 23.96 & 4.09 & 78.55\T\B\\ \hline
\end{tabular}
}
\label{tab:slam_benchmark9}
\end{table}

\clearpage

\begin{table}[!h]
\centering
\caption{\textbf{SLAM Benchmarks for scene10.}}
\resizebox{0.85\textwidth}{!}{
\setlength{\tabcolsep}{10pt}
\begin{tabular}{lc|c|ccc}
\hline
\multicolumn{2}{c|}{Evaluation}                                                  & Tracking & \multicolumn{3}{c}{Mapping} \T\B\\ \hline
\multicolumn{1}{l|}{Methods}                        & \multicolumn{1}{l|}{Depth} & ATE\(\downarrow\) [cm]      & Acc\(\downarrow\) [cm]   & Comp\(\downarrow\) [cm]  & Comp Ratio\(\uparrow\) [\%]  \T\B\\ \hline
\multicolumn{1}{l|}{\multirow{3}{*}{NICE-SLAM~\cite{Zhu2022niceslam}}}          & GT     & 5.13 & 1.94 & 2.63 & 91.72\T\B\\
\multicolumn{1}{l|}{}                                                           & AS & 50.65 & 34.19 & 20.48 & 20.74\T\B\\
\multicolumn{1}{l|}{}                                                           & ToF  & 18.95 & 25.41 & 12.89 & 36.88 \T\B\\ \hline
\multicolumn{1}{l|}{\multirow{3}{*}{CO-SLAM~\cite{wang2023coslam}}}             & GT    & 2.28 & 1.67 & 1.59 & 97.65 \T\B\\
\multicolumn{1}{l|}{}                                                           & AS  &242.38 & 75.08 & 21.55 & 22.98 \T\B\\
\multicolumn{1}{l|}{}                                                           & ToF   & 381.76 & 67.49 & 8.11 & 63.62 \T\B\\ \hline
\multicolumn{1}{l|}{\multirow{3}{*}{Gaussian-SLAM~\cite{yugay2023gaussianslam}}}& GT & 16.06 & 6.66 & 4.40 & 72.90 \T\B\\
\multicolumn{1}{l|}{}                                                           & AS & 56.91 & 77.00 & 19.55 & 16.58 \T\B\\
\multicolumn{1}{l|}{}                                                           & ToF  & 108.39 & 54.44 & 12.57 & 31.69\T\B\\ \hline
\end{tabular}
}
\label{tab:slam_benchmark10}
\end{table}

\begin{table}[!h]
\centering
\caption{\textbf{SLAM Benchmarks for scene11.}}
\resizebox{0.85\textwidth}{!}{
\setlength{\tabcolsep}{10pt}
\begin{tabular}{lc|c|ccc}
\hline
\multicolumn{2}{c|}{Evaluation}                                                  & Tracking & \multicolumn{3}{c}{Mapping} \T\B\\ \hline
\multicolumn{1}{l|}{Methods}                        & \multicolumn{1}{l|}{Depth} & ATE\(\downarrow\) [cm]      & Acc\(\downarrow\) [cm]   & Comp\(\downarrow\) [cm]  & Comp Ratio\(\uparrow\) [\%]  \T\B\\ \hline
\multicolumn{1}{l|}{\multirow{3}{*}{NICE-SLAM~\cite{Zhu2022niceslam}}}          & GT     & 1.07 & 1.93 & 3.37 & 88.64\T\B\\
\multicolumn{1}{l|}{}                                                           & AS & 79.10 & 34.19 & 29.38 & 16.50\T\B\\
\multicolumn{1}{l|}{}                                                           & ToF  & 11.86 & 16.00 & 8.72 & 52.62 \T\B\\ \hline
\multicolumn{1}{l|}{\multirow{3}{*}{CO-SLAM~\cite{wang2023coslam}}}             & GT    & 3.06 & 1.96 & 1.70 & 97.92 \T\B\\
\multicolumn{1}{l|}{}                                                           & AS  & 51.78 & 40.79 & 19.51 & 17.23 \T\B\\
\multicolumn{1}{l|}{}                                                           & ToF   & 42.3 & 71.10 & 9.68 & 40.71 \T\B\\ \hline
\multicolumn{1}{l|}{\multirow{3}{*}{Gaussian-SLAM~\cite{yugay2023gaussianslam}}}& GT & 7.21 & 3.66 & 2.80 & 85.46 \T\B\\
\multicolumn{1}{l|}{}                                                           & AS & 119.20 & 60.03 & 33.32 & 14.11 \T\B\\
\multicolumn{1}{l|}{}                                                           & ToF  & 69.43 & 46.15 & 11.18 & 36.03\T\B\\ \hline
\end{tabular}
}
\label{tab:slam_benchmark11}
\end{table}

\clearpage
